# Supplementary material for: DeforestVis: Behavior Analysis of Machine Learning Models with Surrogate Decision Stumps
Source: arXiv:2304.00133 source file (2024-04-18)

# Supplemental Material

## DeforestVis: Behavior Analysis of Machine Learning Models with Surrogate Decision Stump

A. Chatzimparpas, R. M. Martins, A. C. Telea, and A. Kerren

## Section 6.1: Use case

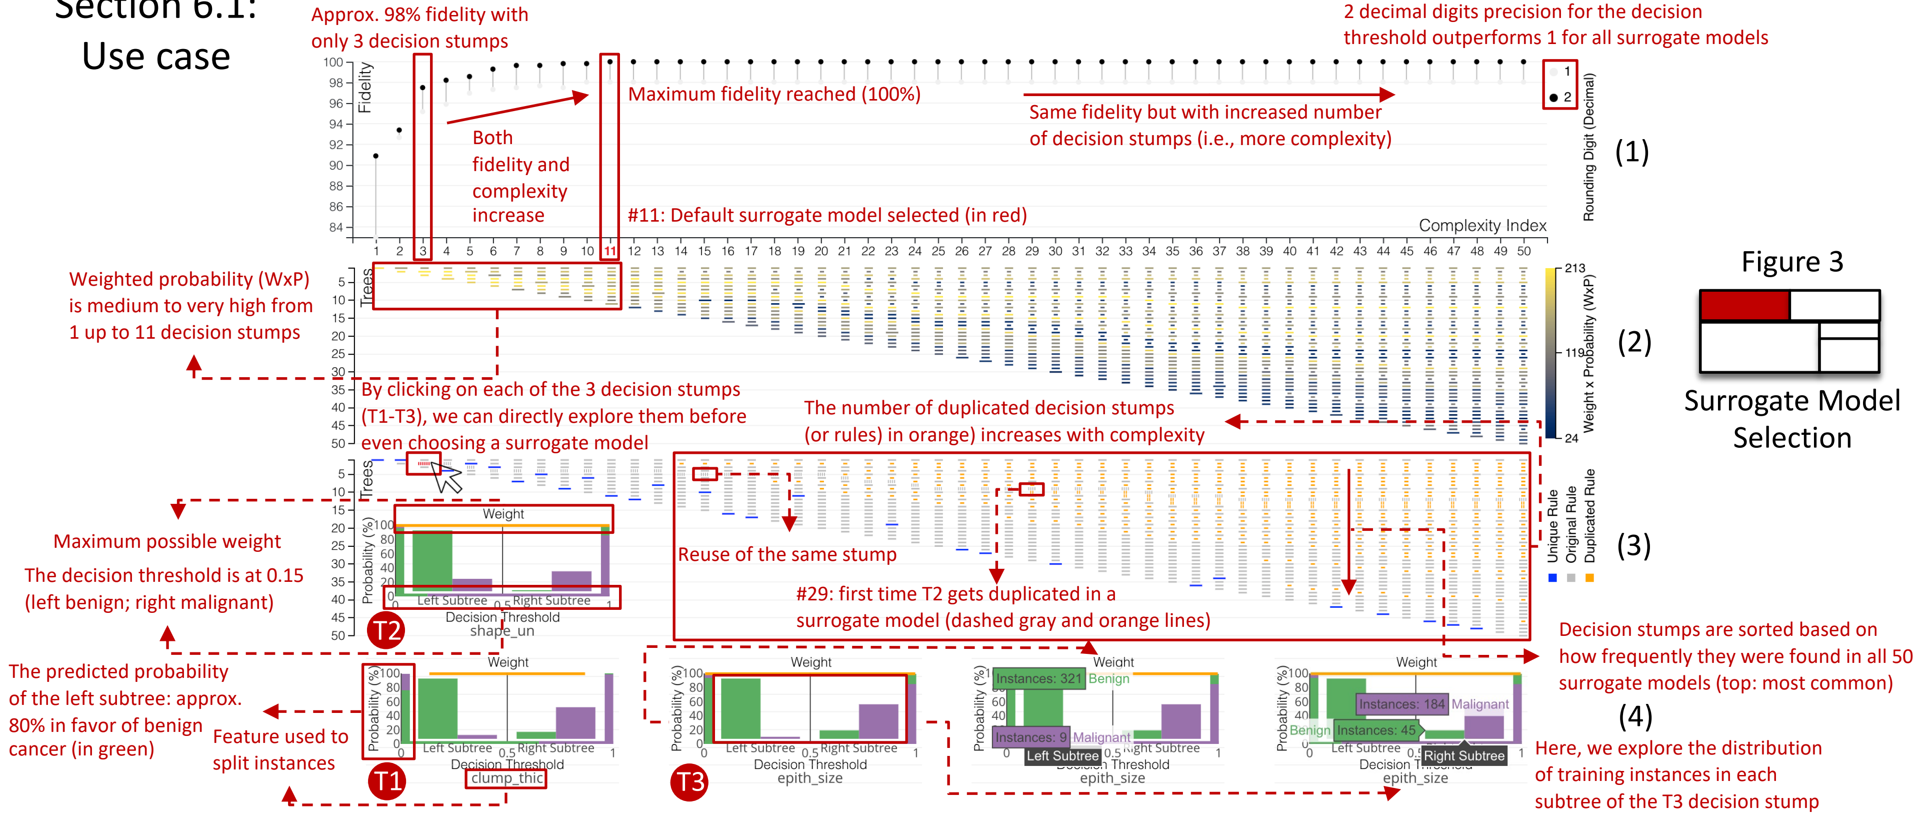


Figure 3

Surrogate Model Selection

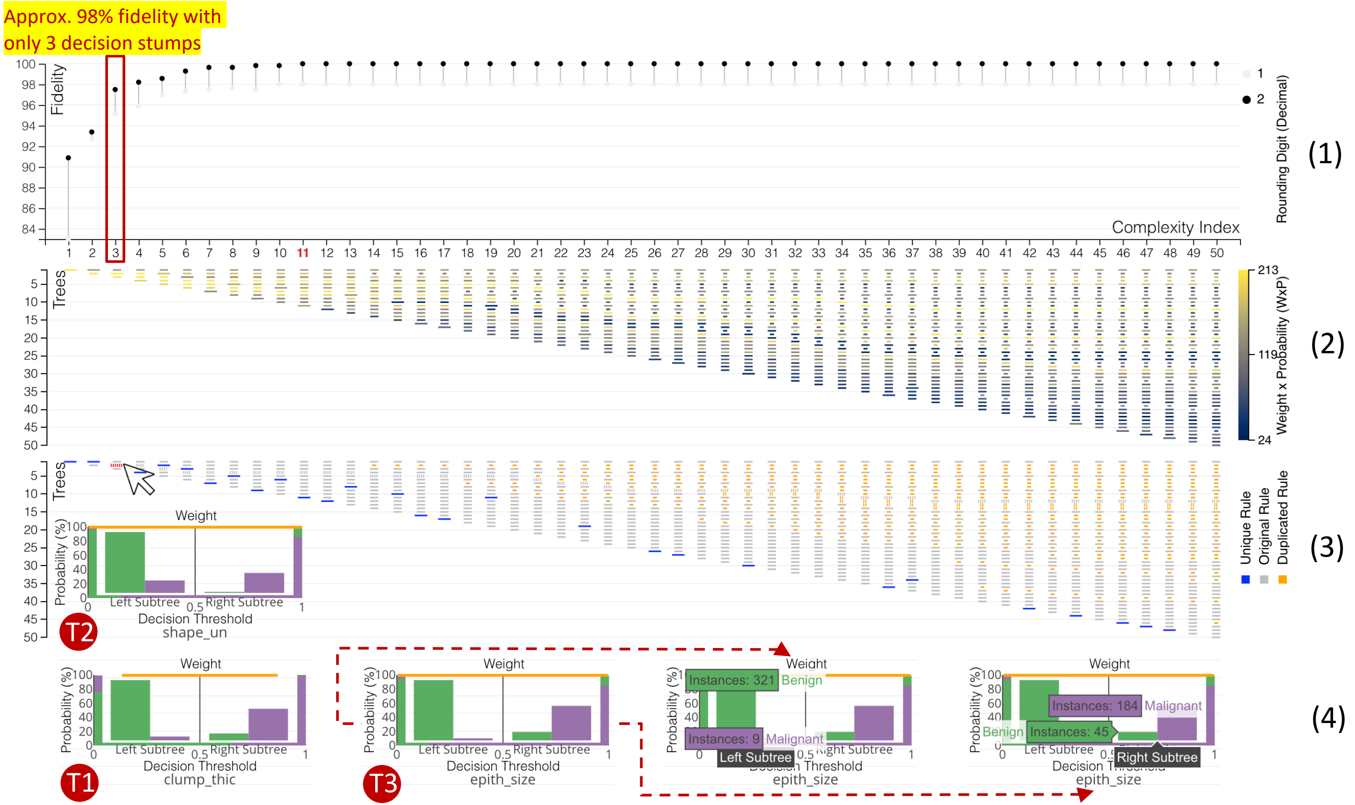


Figure 3

Surrogate Model Selection

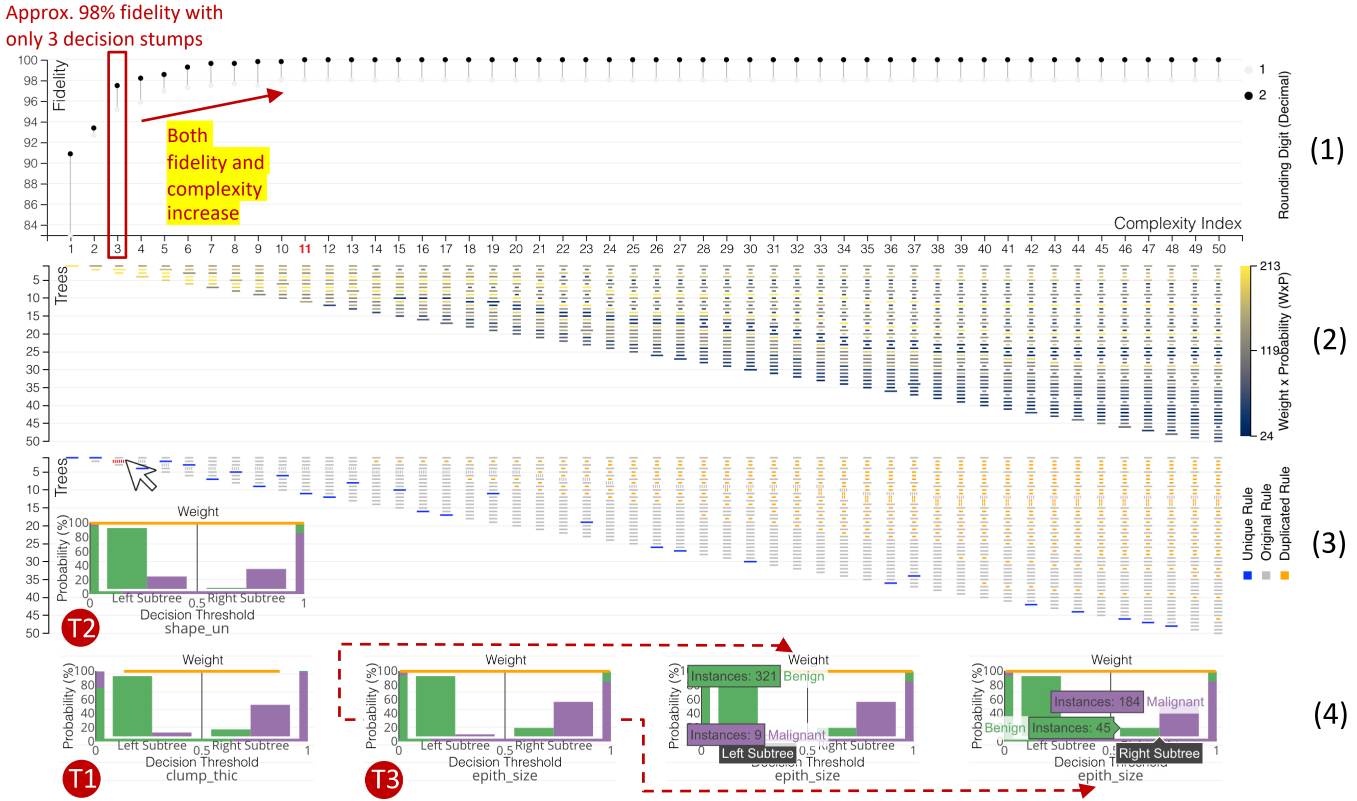


Figure 3

Surrogate Model Selection

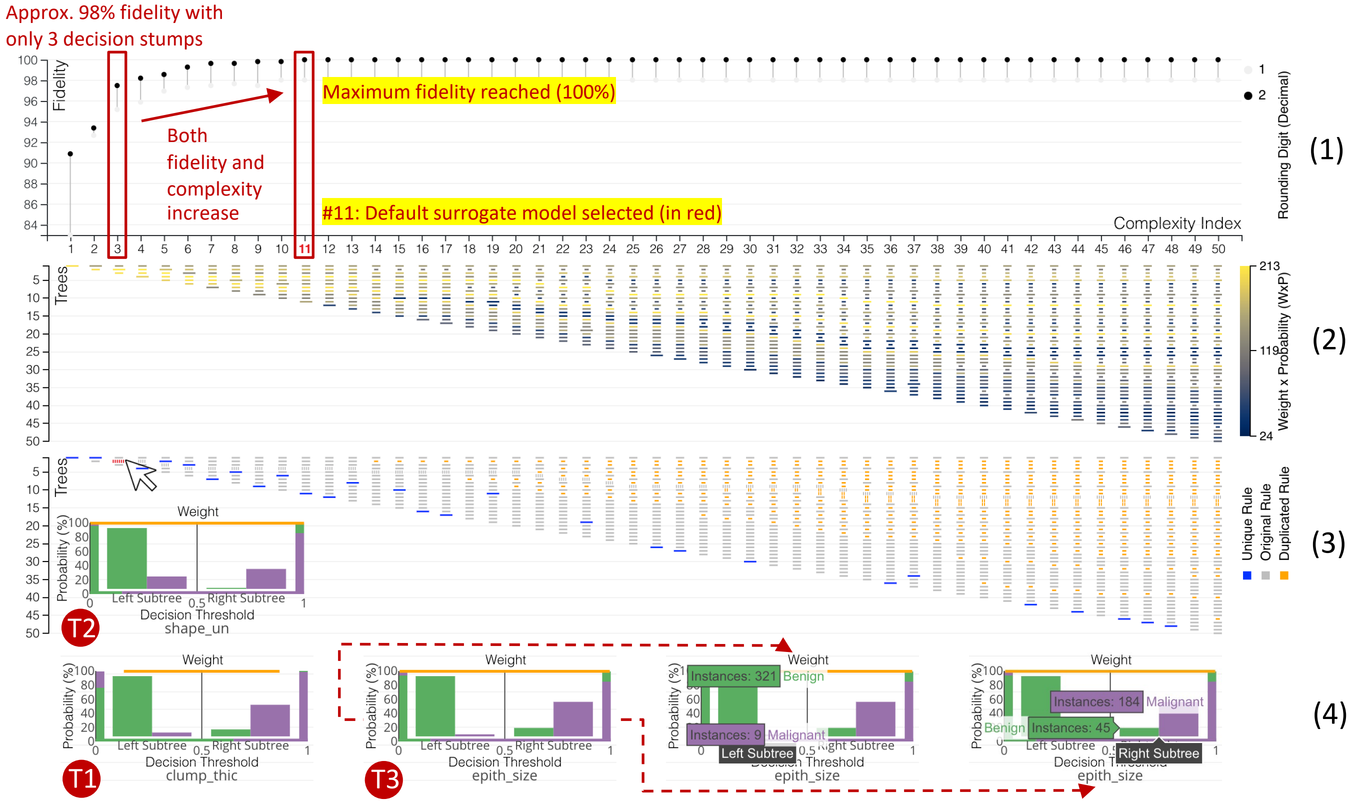


Figure 3

Surrogate Model Selection

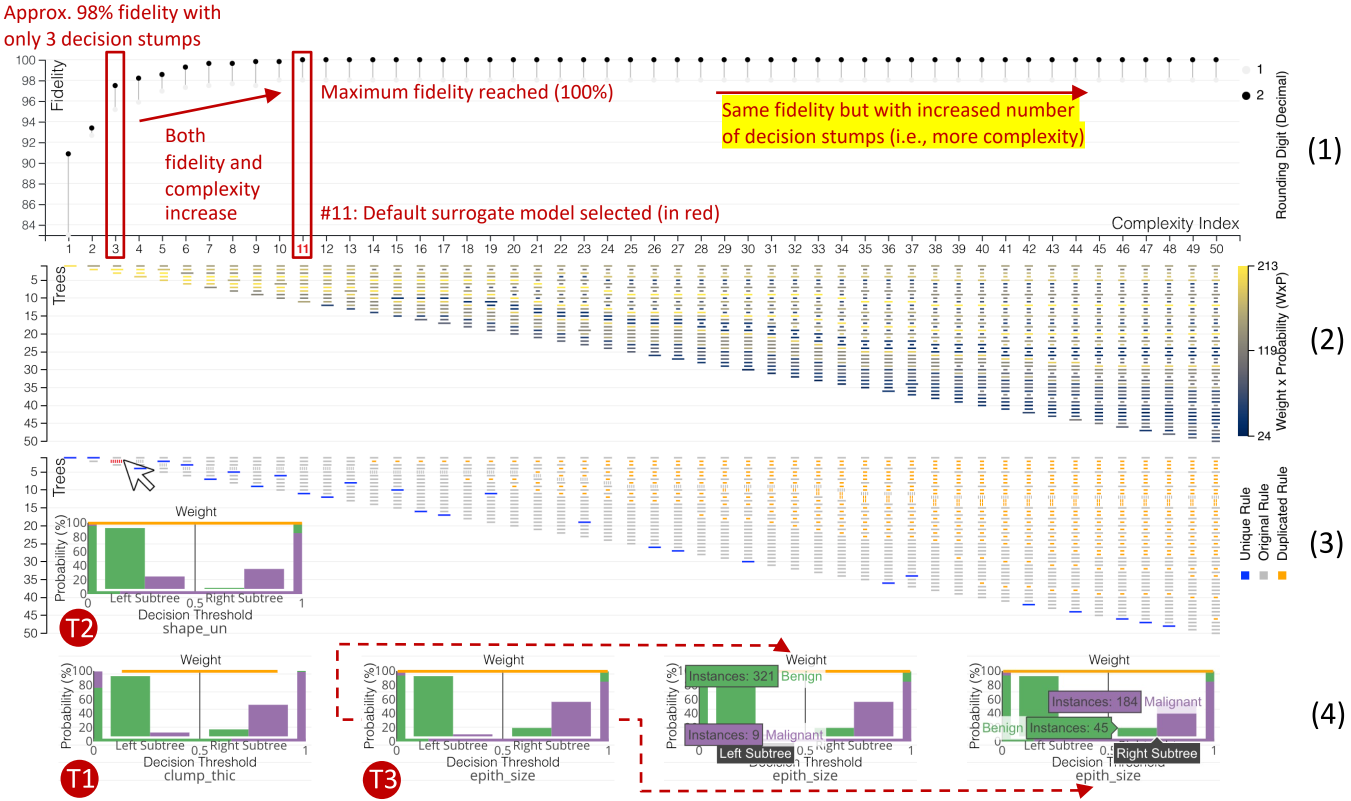


Figure 3

Surrogate Model Selection

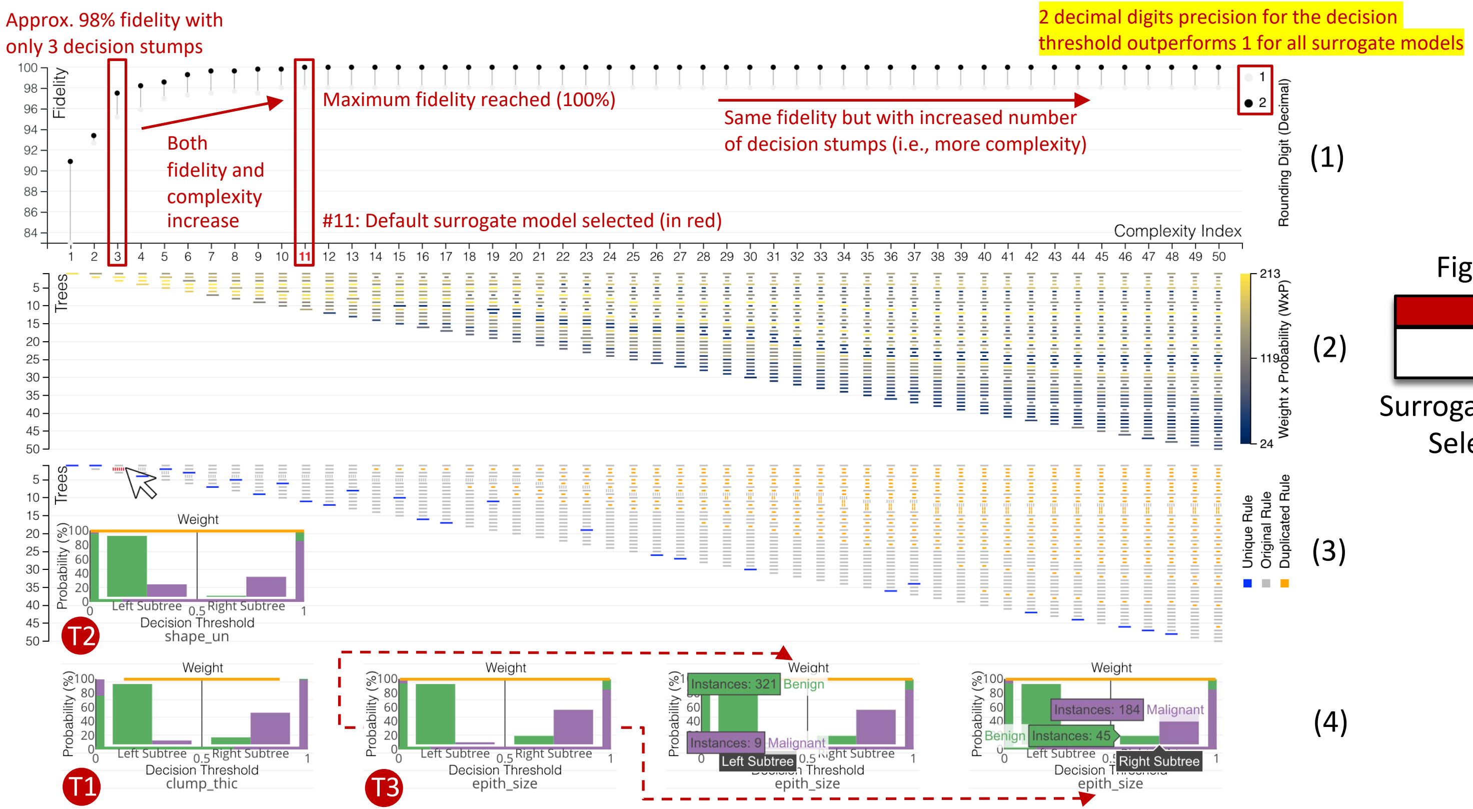


Figure 3

Surrogate Model Selection

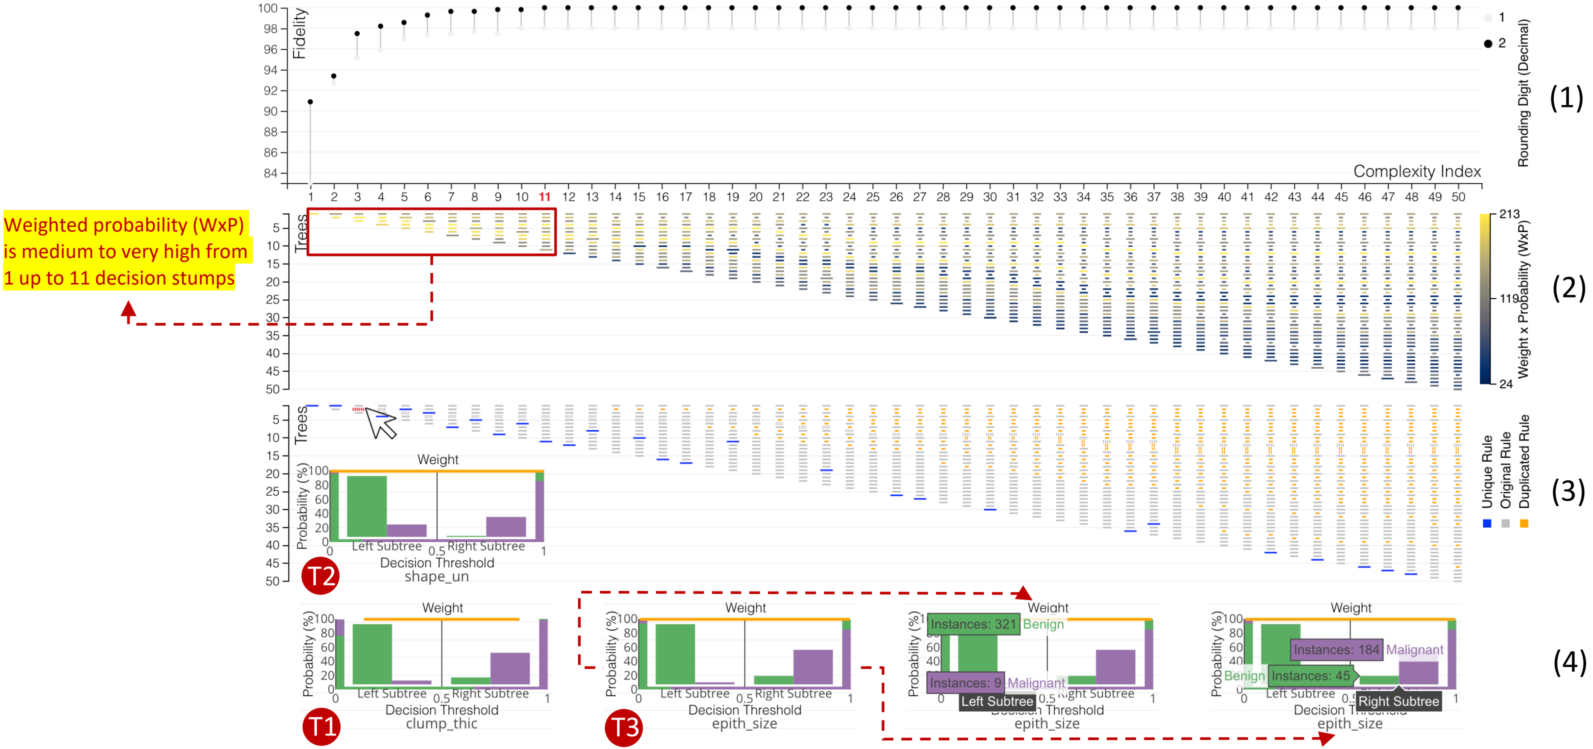


Figure 3

Surrogate Model Selection

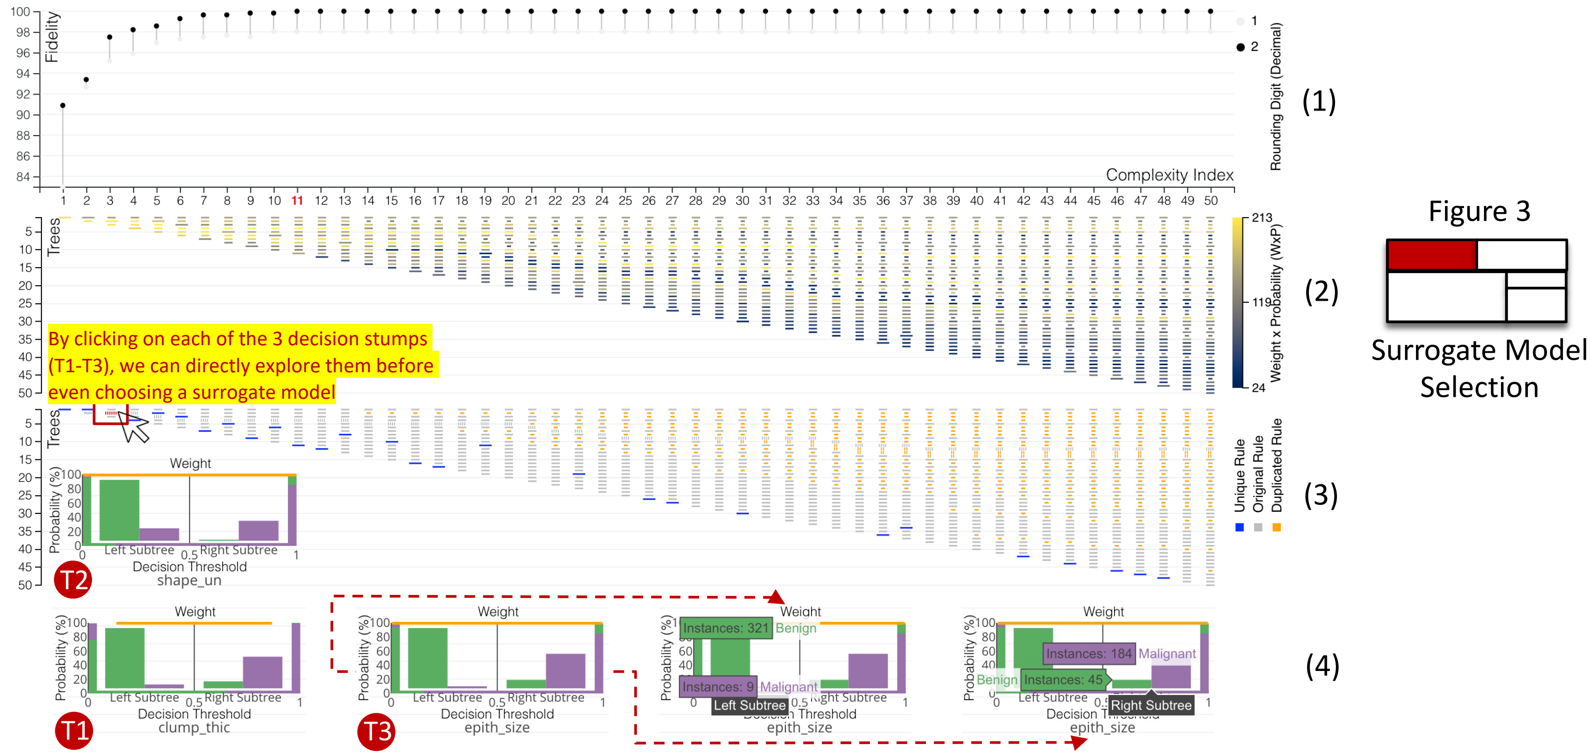
Fidelity
Complexity Index
Rounding Digit (Decimal)
(1)
Trees
Weight x Probability (WxP)
(2)
By clicking on each of the 3 decision stumps (T1-T3), we can directly explore them before even choosing a surrogate model
Unique Rule
Original Rule
Duplicated Rule
(3)
Weight
Probability (%)
Left Subtree
Right Subtree
Decision Threshold
shape_un
T2
clump_thic
T1
epith_size
T3
Instances: 321
Benign
Instances: 9
Malignant
Instances: 184
Instances: 45
(4)
Figure 3
Surrogate Model Selection

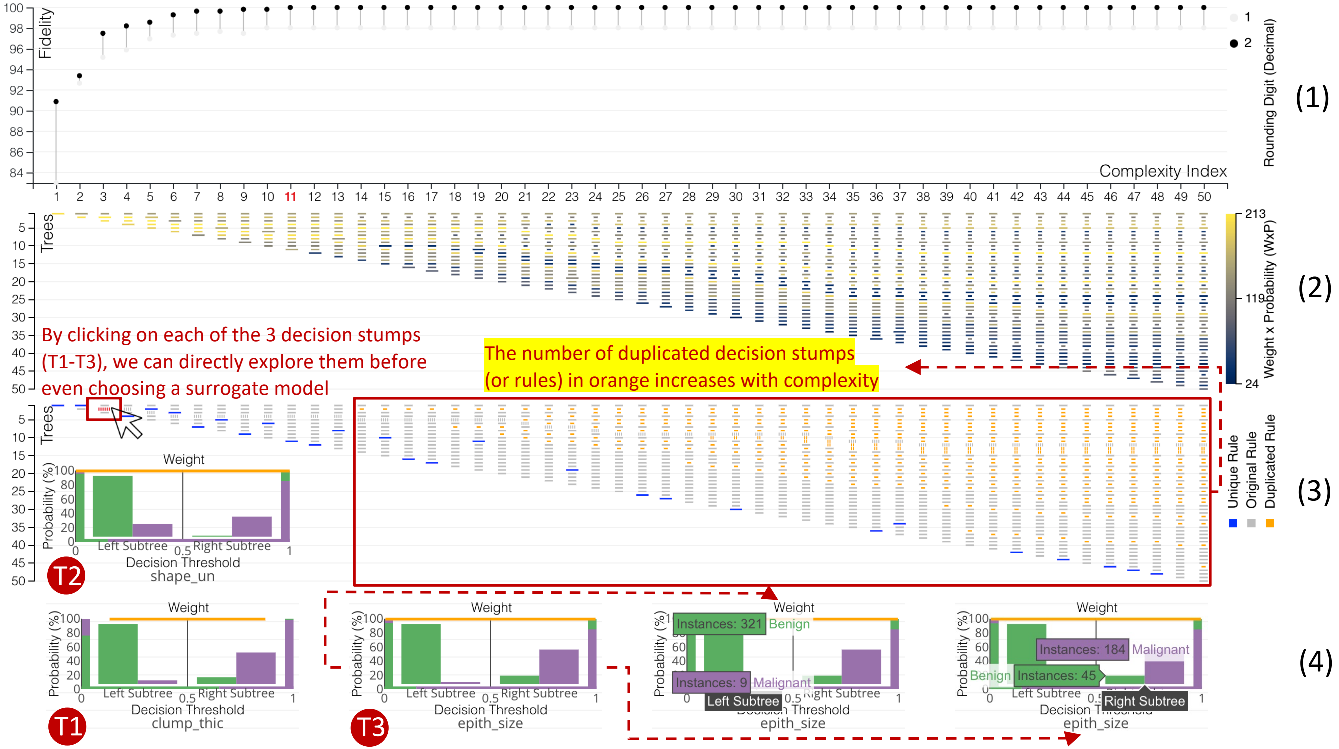


# Figure 3

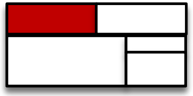

## Surrogate Model Selection

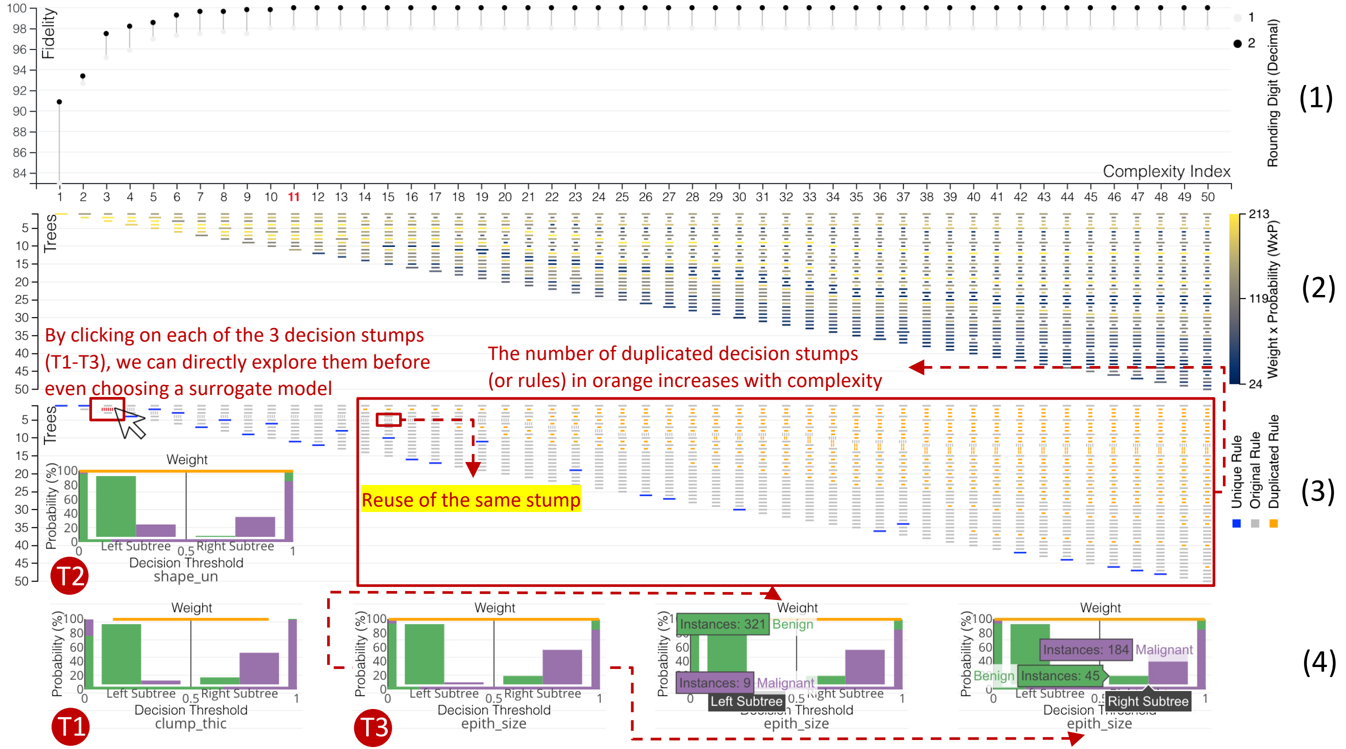


Figure 3

Surrogate Model Selection

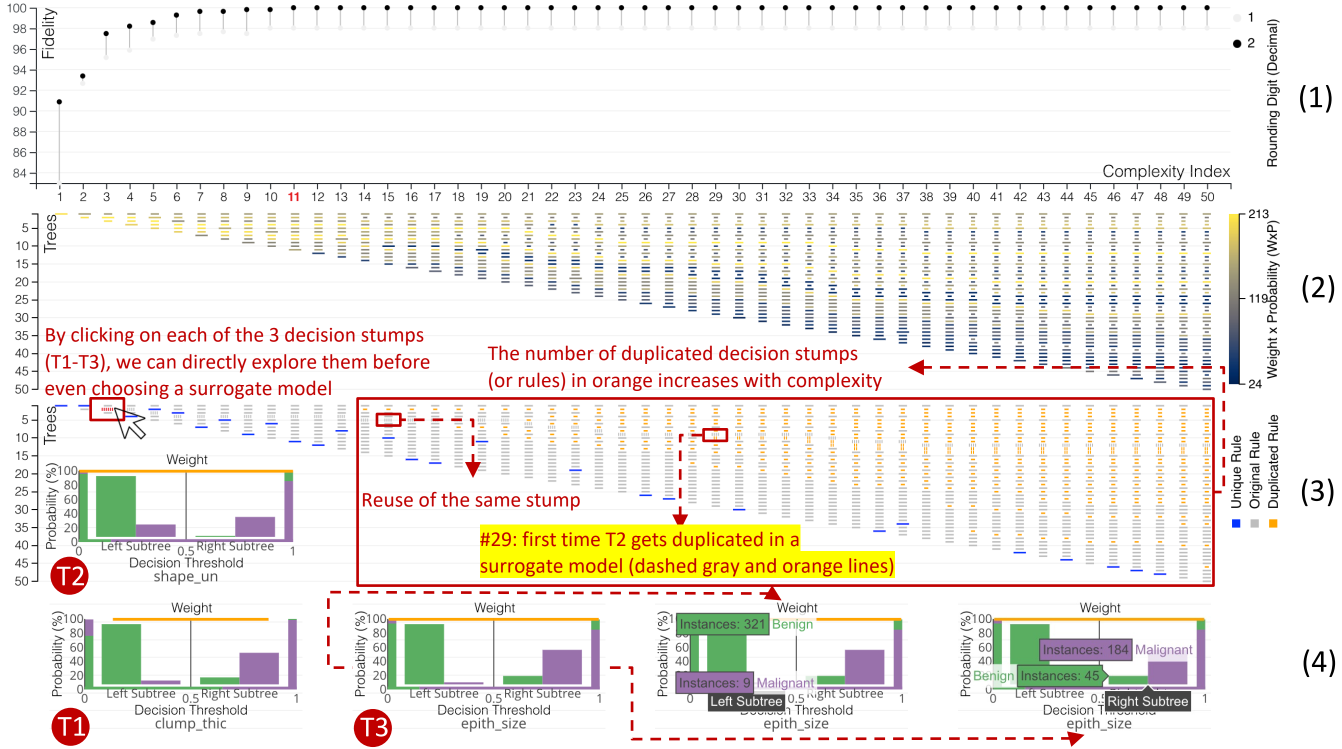


## Figure 3

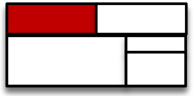

Surrogate Model Selection

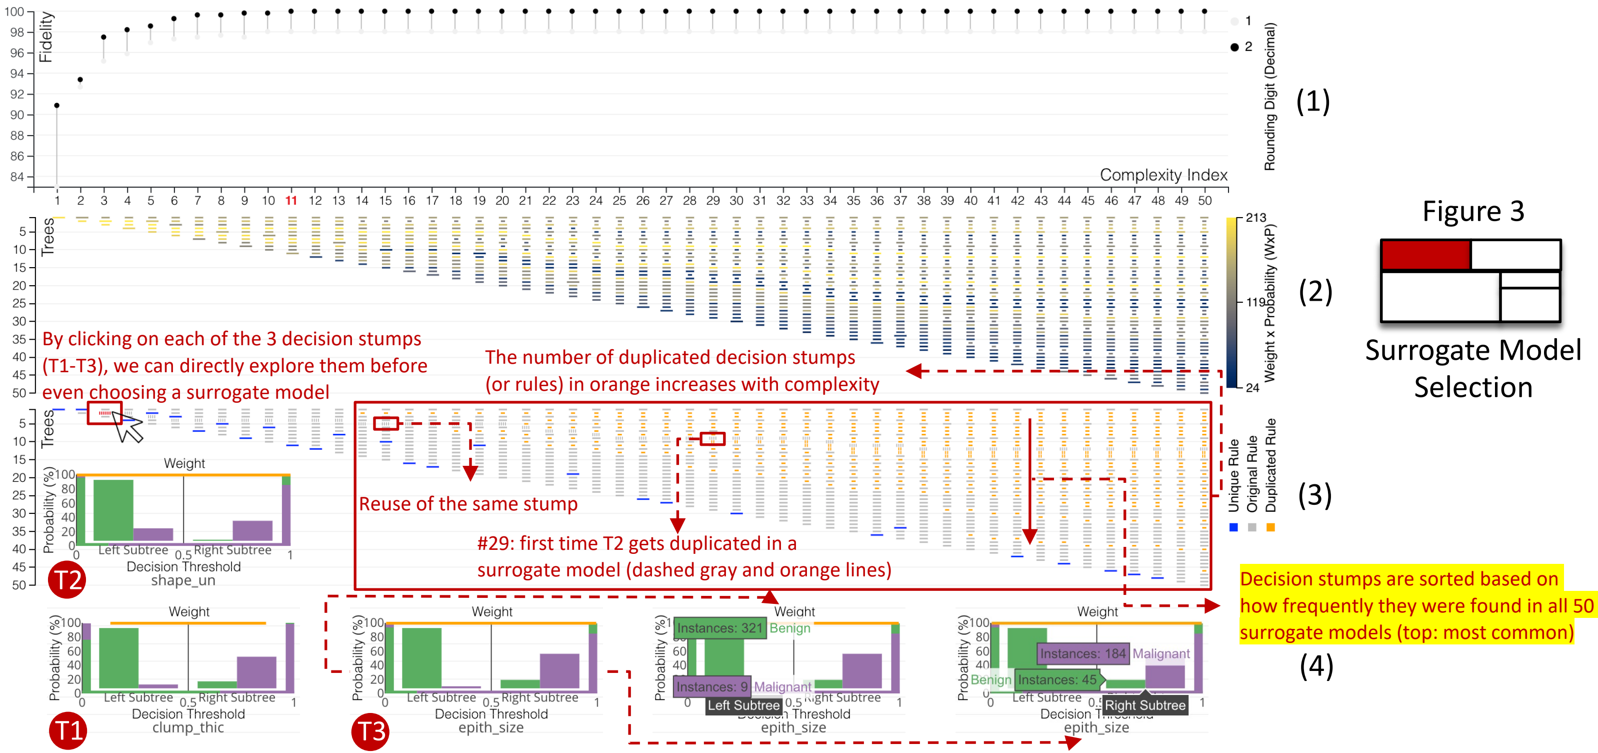


Figure 3

Surrogate Model Selection

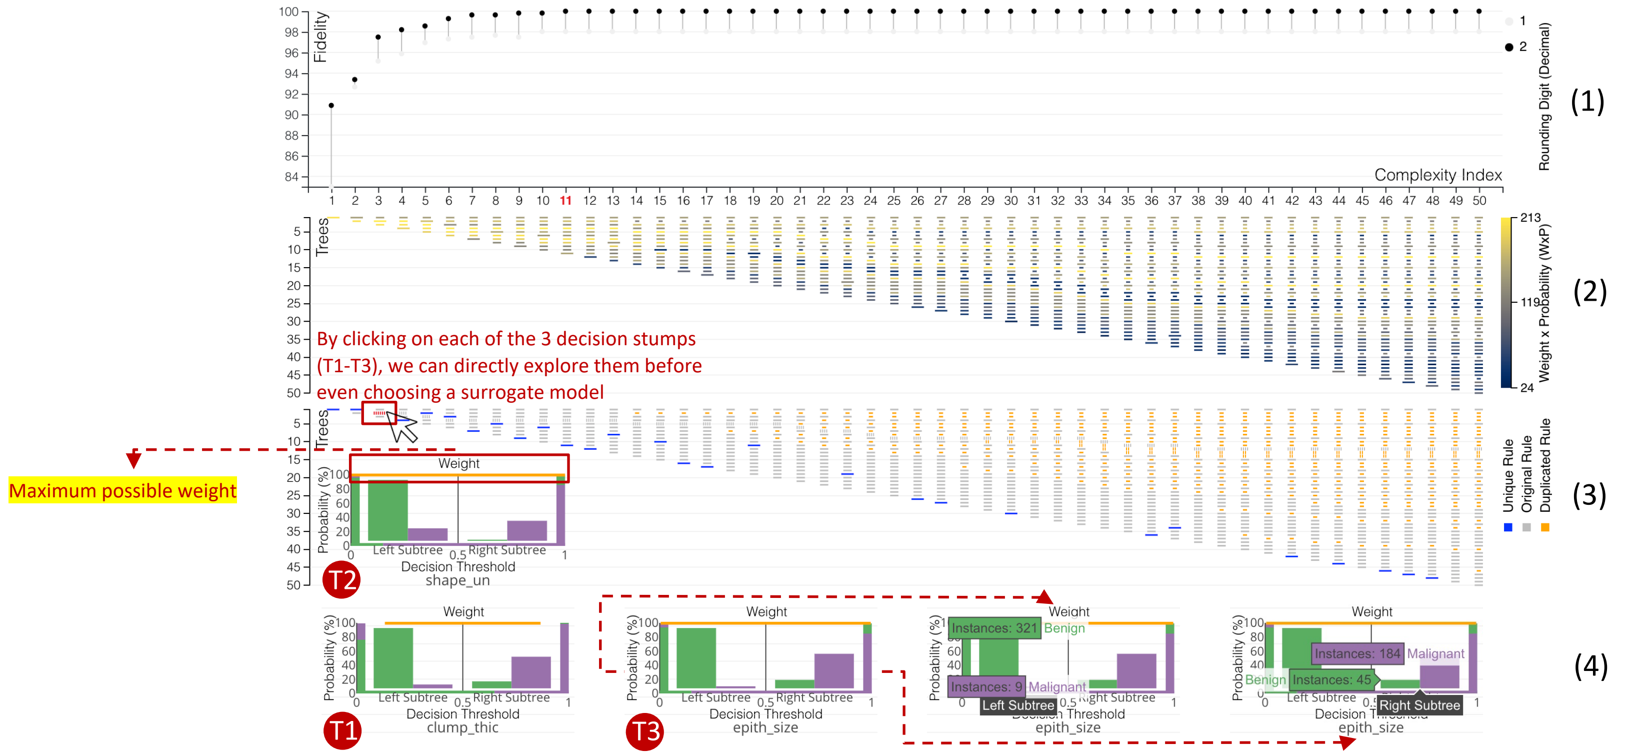


Figure 3

Surrogate Model Selection

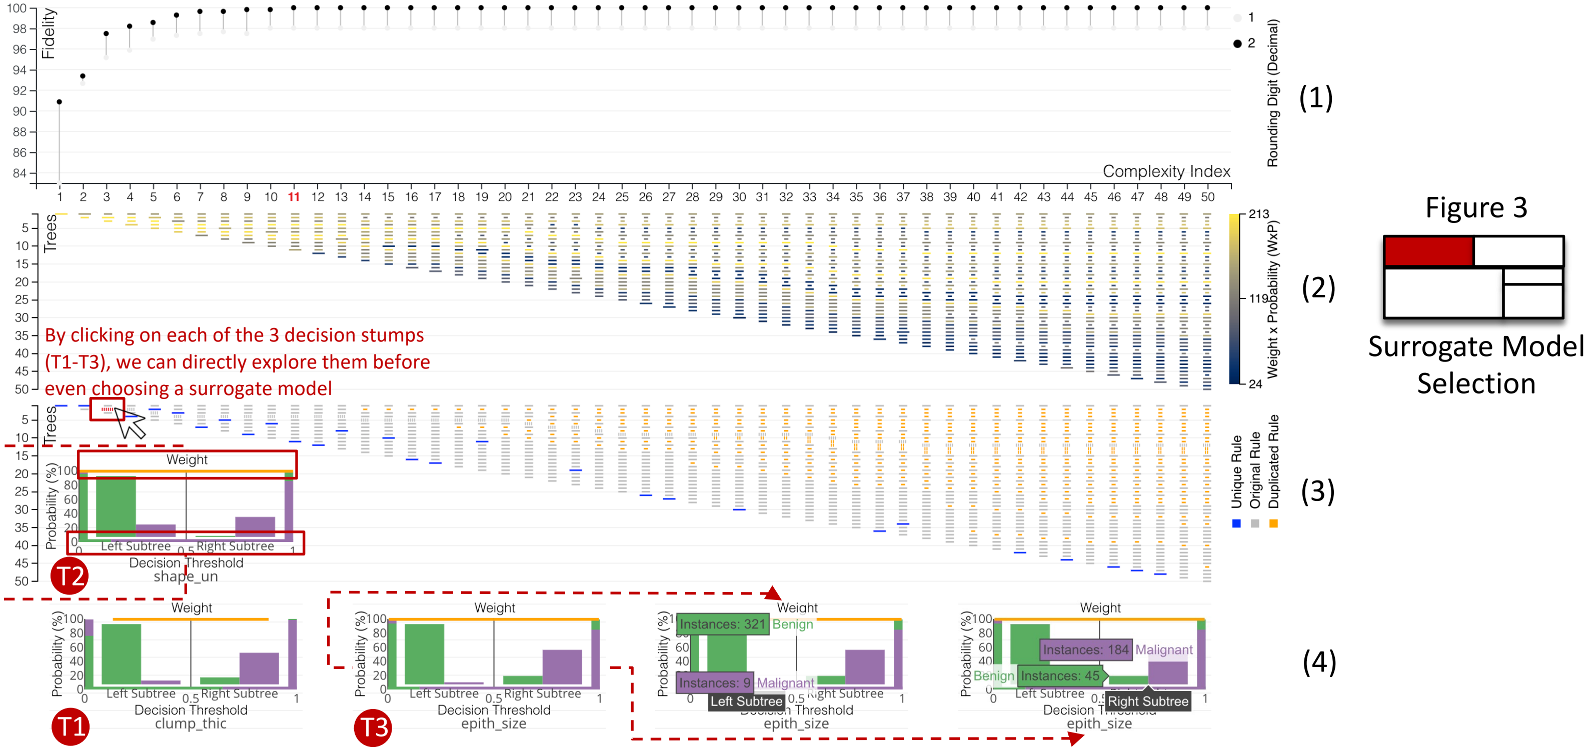
Fidelity
Complexity Index
Rounding Digit (Decimal)
(1)
Trees
Weight x Probability (WxP)
(2)
By clicking on each of the 3 decision stumps (T1-T3), we can directly explore them before even choosing a surrogate model
Unique Rule
Original Rule
Duplicated Rule
(3)
Maximum possible weight
The decision threshold is at 0.15 (left benign; right malignant)
Weight
Probability (%)
Left Subtree
Right Subtree
Decision Threshold
shape_un
T2
clump_thic
T1
epith_size
T3
Instances: 321
Benign
Instances: 9
Malignant
Instances: 184
Instances: 45
(4)
Figure 3
Surrogate Model Selection

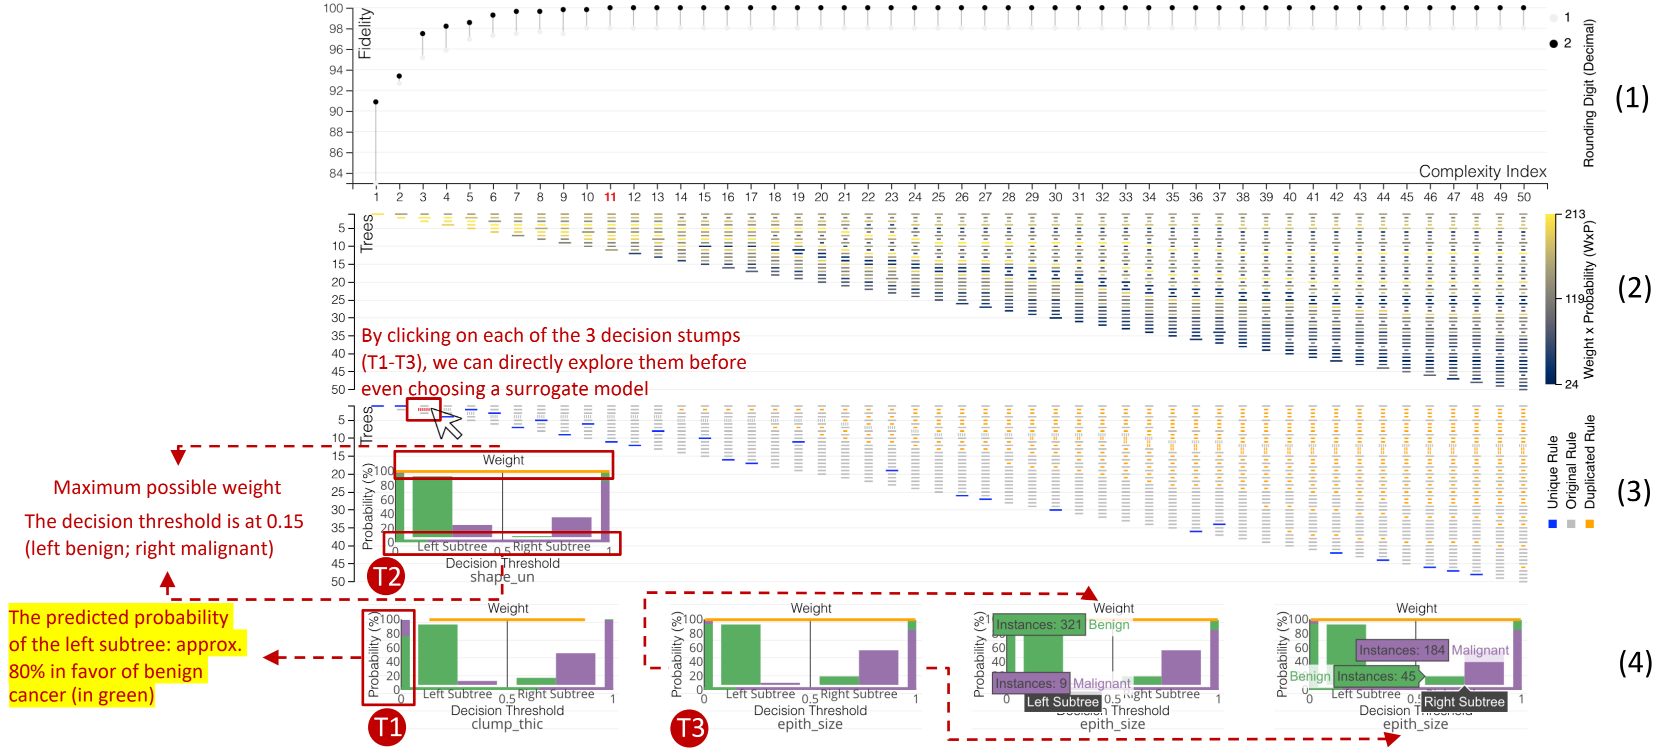


## Figure 3

Surrogate Model Selection

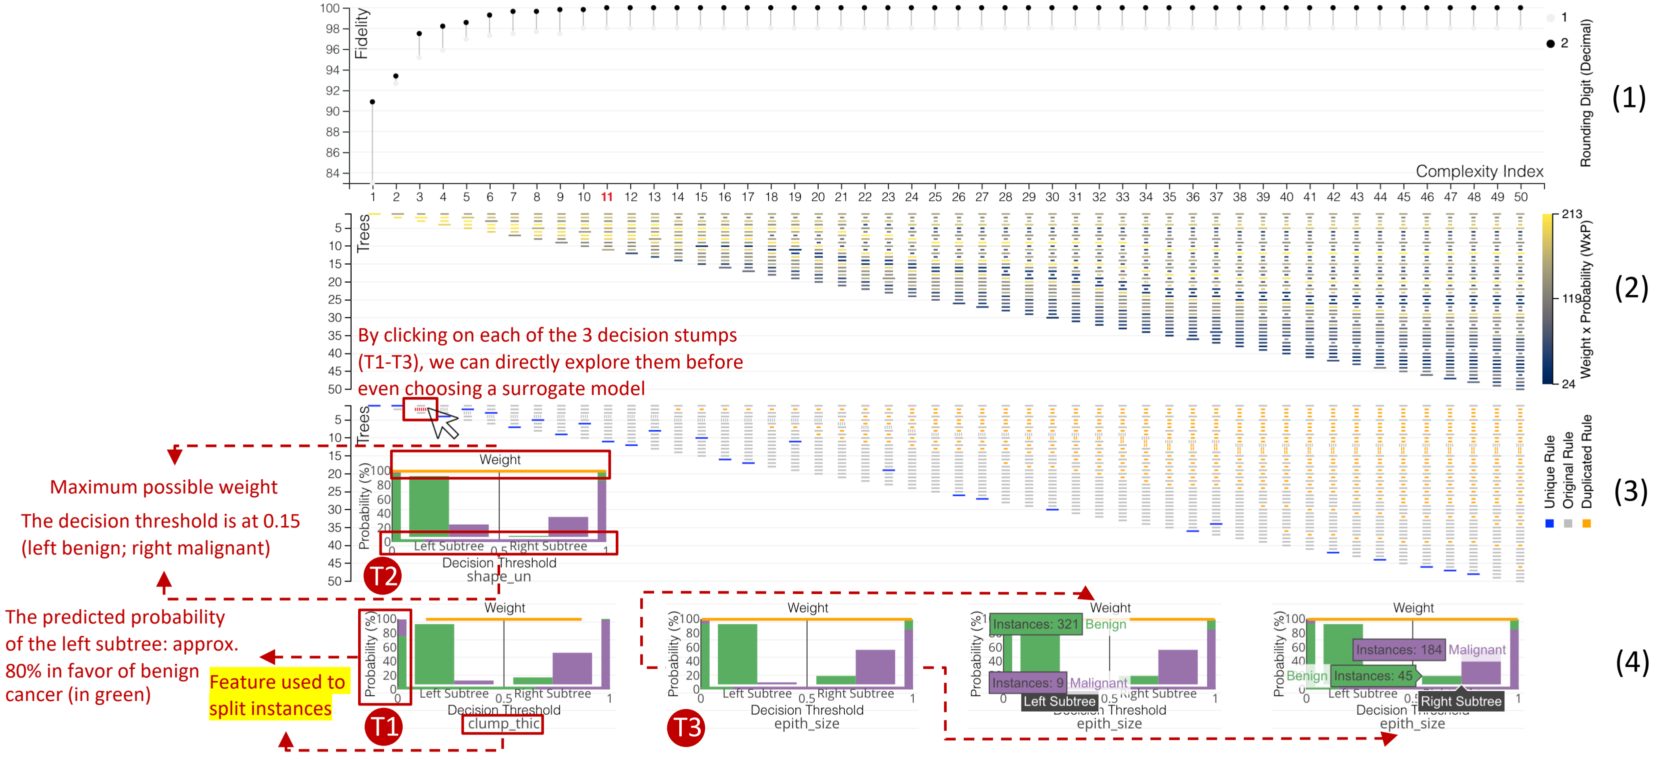


# Figure 3

Surrogate Model Selection

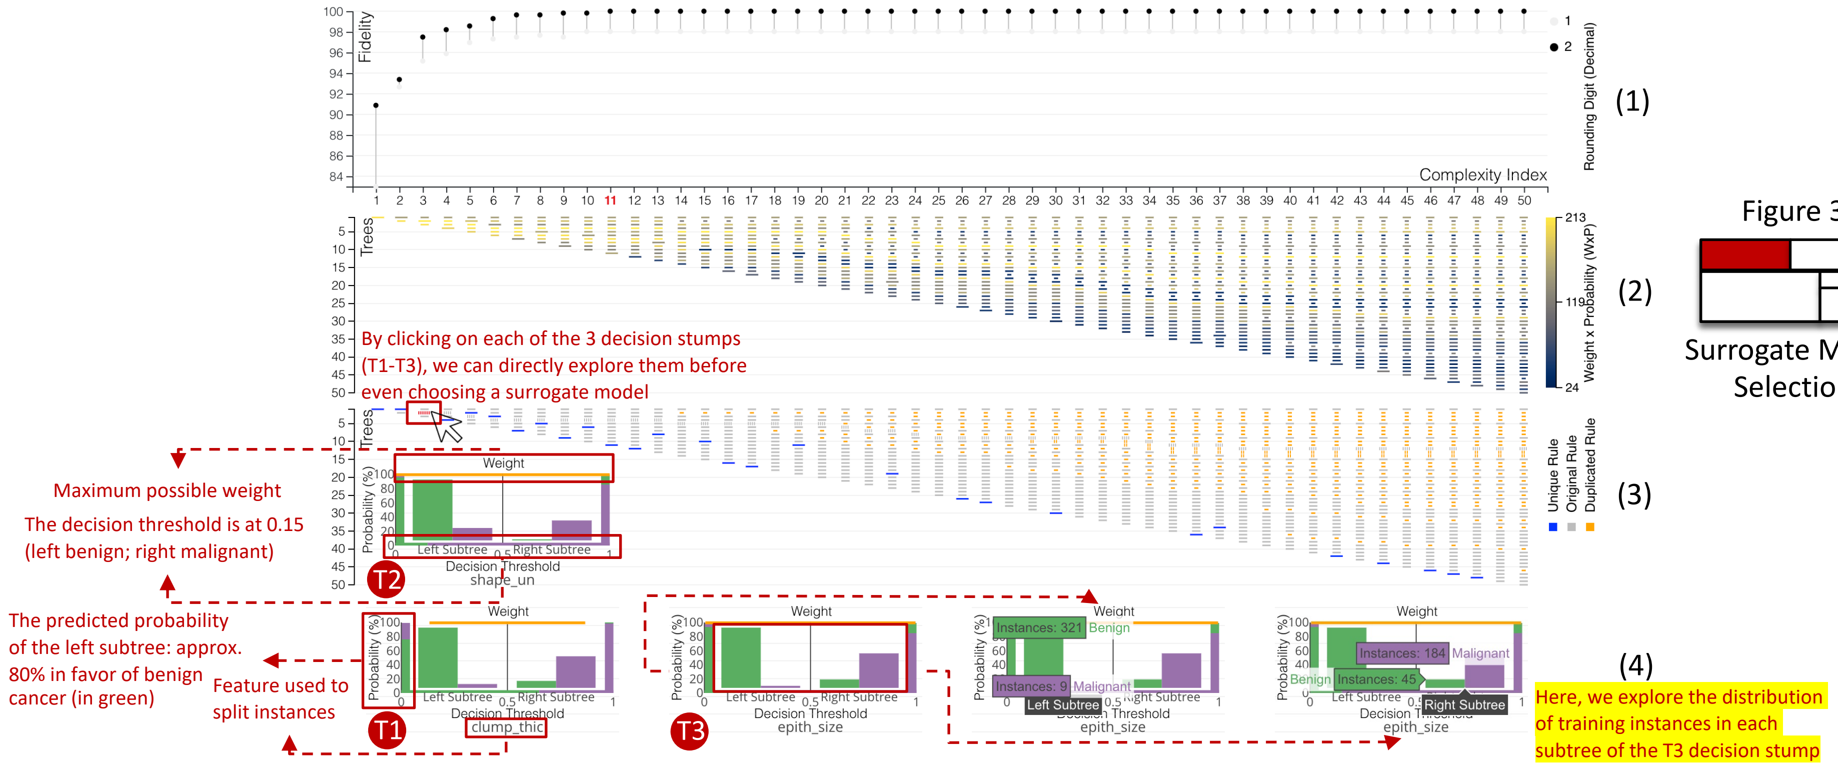


Figure 3

Surrogate Model Selection

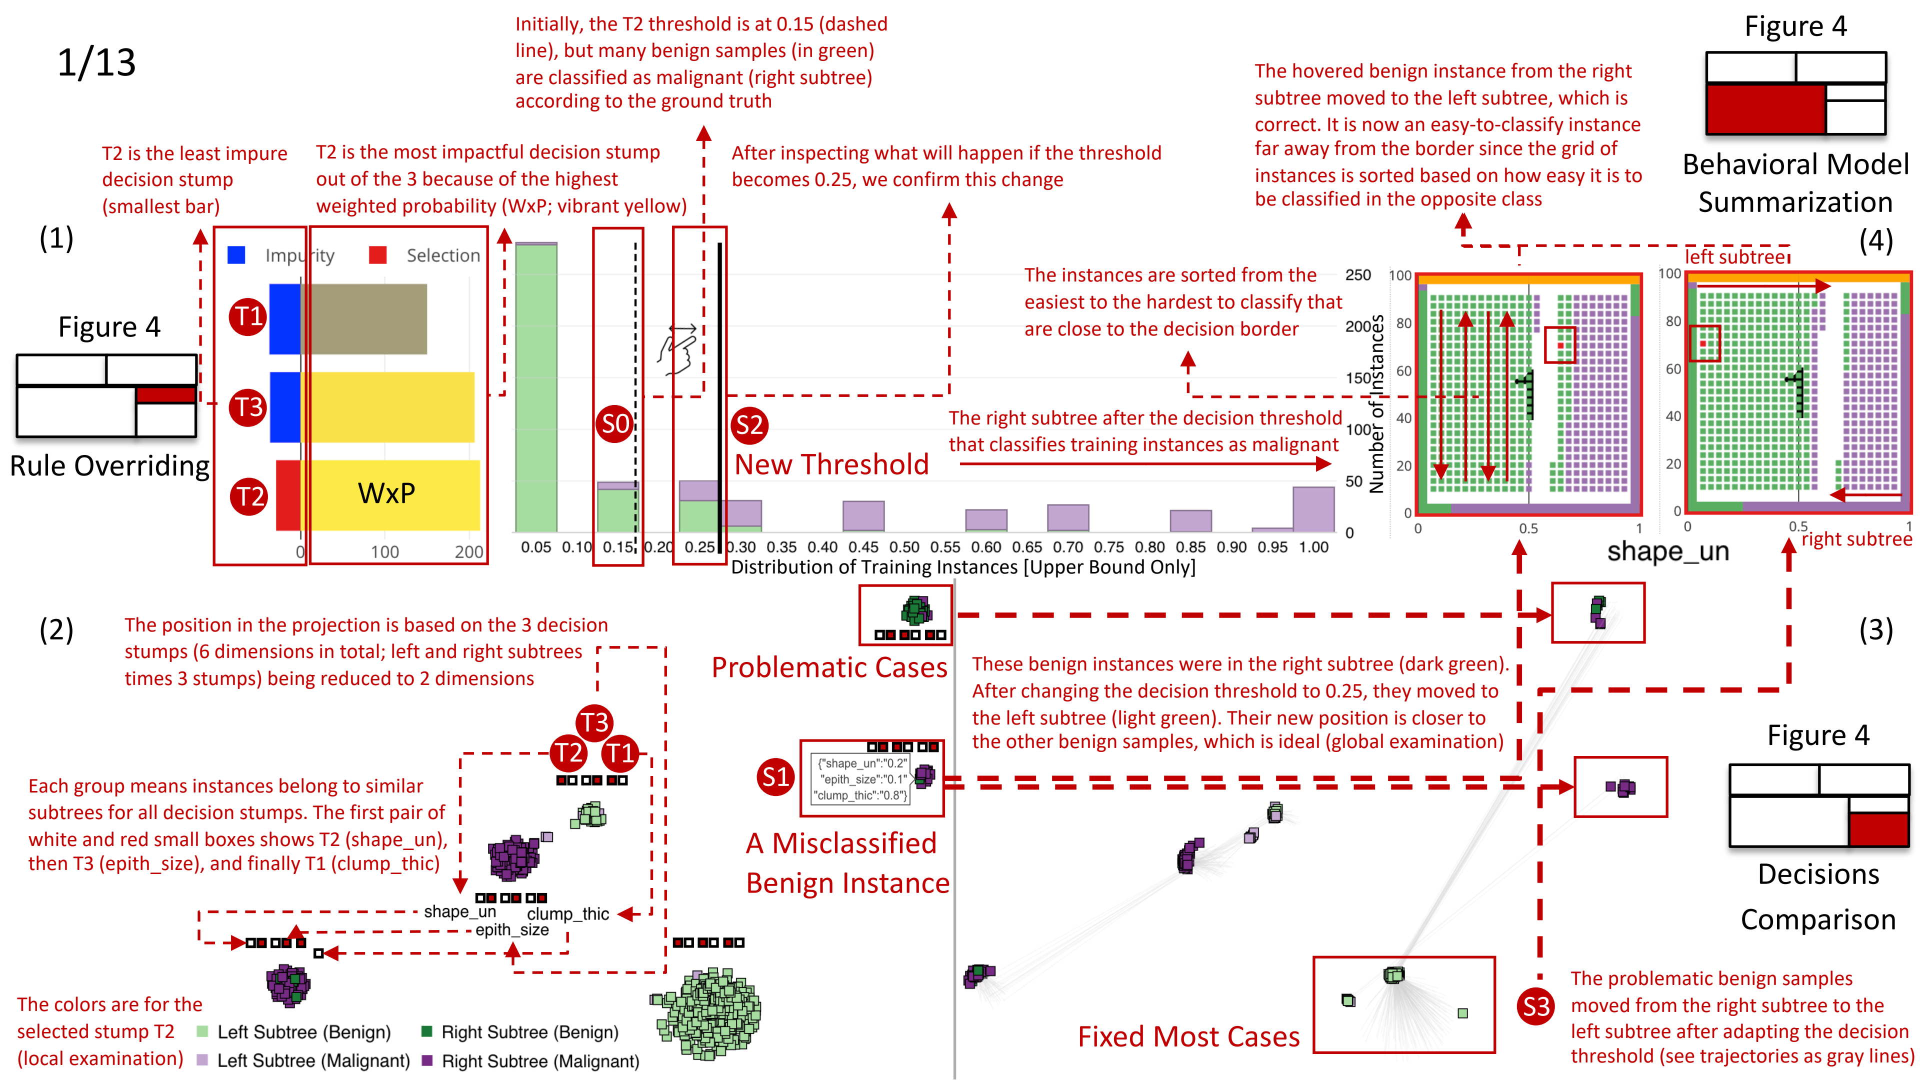
1/13
(1)
Figure 4
Rule Overriding
T2 is the least impure decision stump (smallest bar)
T2 is the most impactful decision stump out of the 3 because of the highest weighted probability (WxP; vibrant yellow)
Initially, the T2 threshold is at 0.15 (dashed line), but many benign samples (in green) are classified as malignant (right subtree) according to the ground truth
After inspecting what will happen if the threshold becomes 0.25, we confirm this change
Impurity
Selection
T1
T3
T2
WxP
0
100
200
S0
S2
New Threshold
The instances are sorted from the easiest to the hardest to classify that are close to the decision border
The right subtree after the decision threshold that classifies training instances as malignant
0.05 0.10 0.15 0.20 0.25 0.30 0.35 0.40 0.45 0.50 0.55 0.60 0.65 0.70 0.75 0.80 0.85 0.90 0.95 1.00
Distribution of Training Instances [Upper Bound Only]
Number of Instances
250
200
150
100
50
0
Figure 4
Behavioral Model Summarization
(4)
The hovered benign instance from the right subtree moved to the left subtree, which is correct. It is now an easy-to-classify instance far away from the border since the grid of instances is sorted based on how easy it is to be classified in the opposite class
left subtree
right subtree
shape_un
(2)
The position in the projection is based on the 3 decision stumps (6 dimensions in total; left and right subtrees times 3 stumps) being reduced to 2 dimensions
Each group means instances belong to similar subtrees for all decision stumps. The first pair of white and red small boxes shows T2 (shape_un), then T3 (epith_size), and finally T1 (clump_thic)
shape_un
epith_size
clump_thic
The colors are for the selected stump T2 (local examination)
Left Subtree (Benign)
Right Subtree (Benign)
Left Subtree (Malignant)
Right Subtree (Malignant)
Problematic Cases
S1
{"shape_un":"0.2" "epith_size":"0.1" "clump_thic":"0.8"}
A Misclassified Benign Instance
These benign instances were in the right subtree (dark green). After changing the decision threshold to 0.25, they moved to the left subtree (light green). Their new position is closer to the other benign samples, which is ideal (global examination)
(3)
Figure 4
Decisions Comparison
Fixed Most Cases
S3
The problematic benign samples moved from the right subtree to the left subtree after adapting the decision threshold (see trajectories as gray lines)

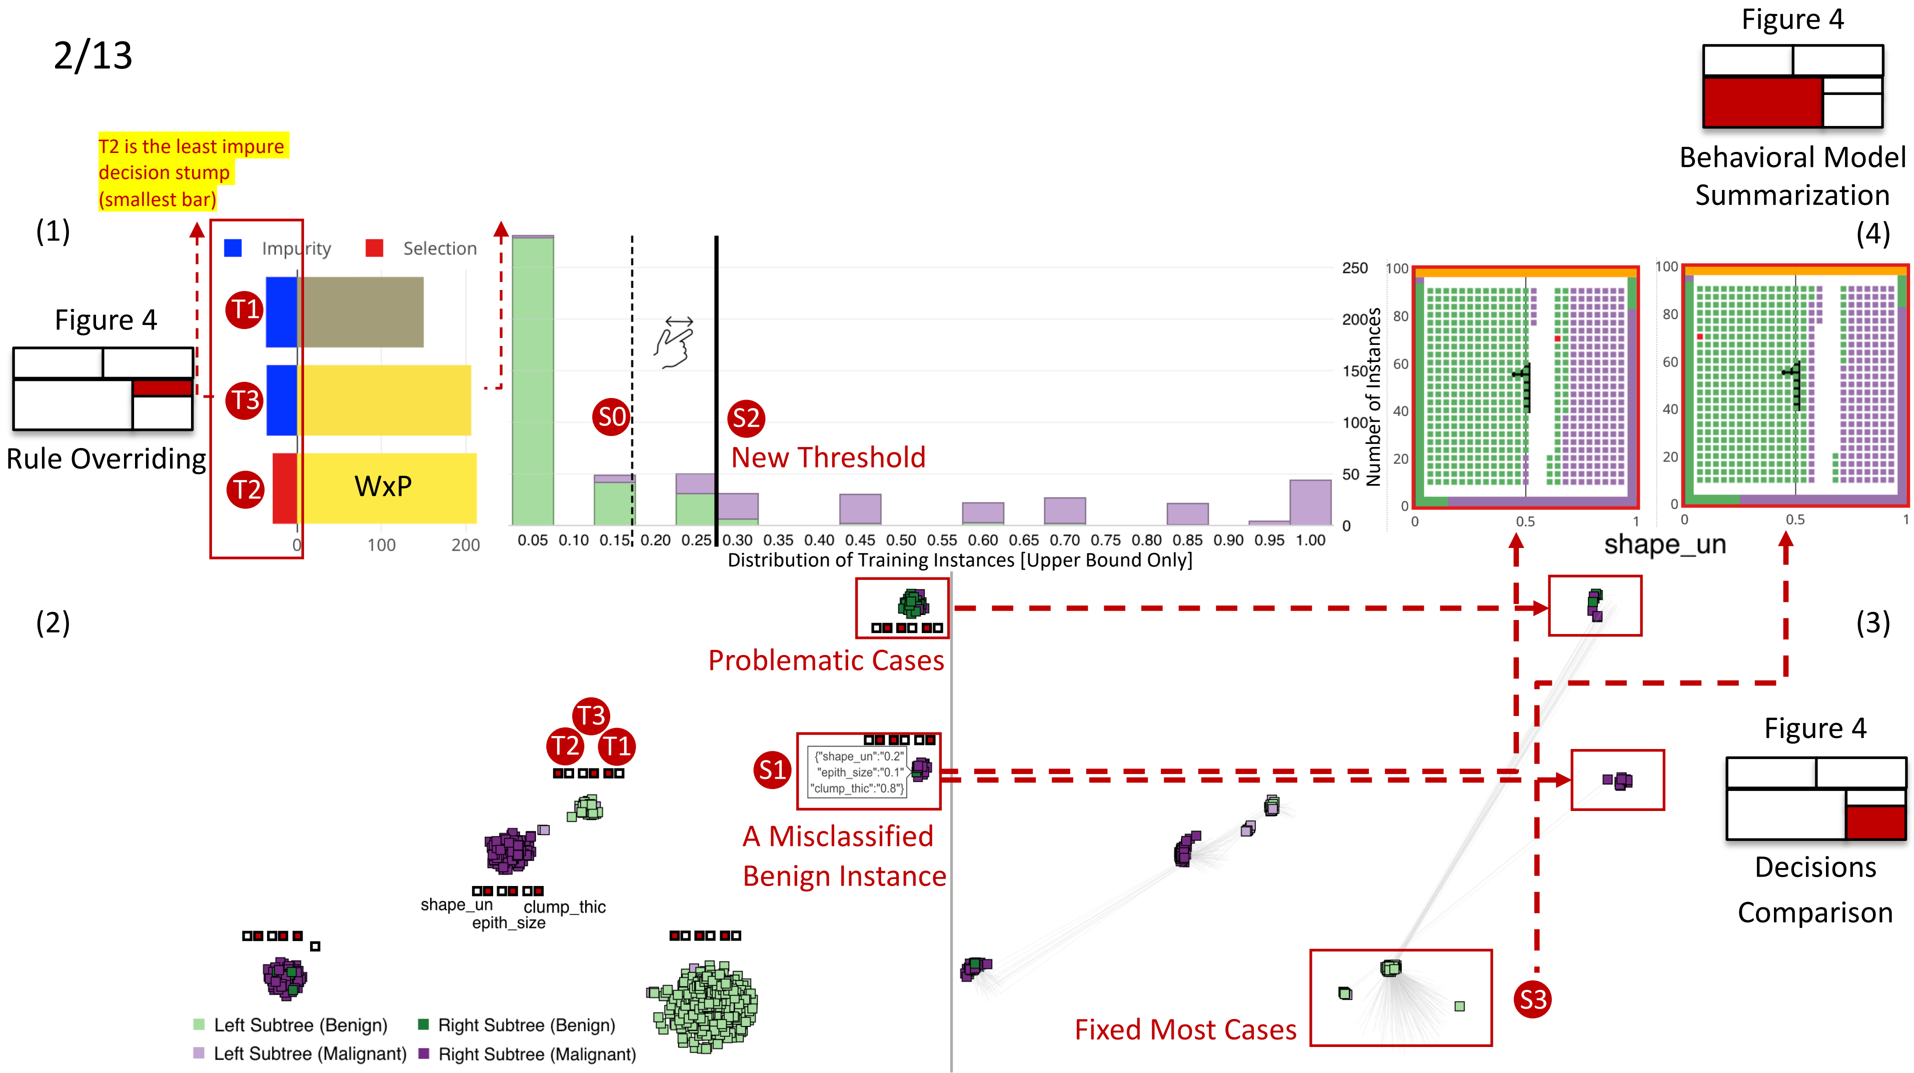

Figure 4
Behavioral Model Summarization
(4)
T2 is the least impure decision stump (smallest bar)
(1)
Figure 4
Rule Overriding
Impurity
Selection
T1
T3
T2
WxP
0
100
200
S0
S2
New Threshold
Distribution of Training Instances [Upper Bound Only]
0.05 0.10 0.15 0.20 0.25 0.30 0.35 0.40 0.45 0.50 0.55 0.60 0.65 0.70 0.75 0.80 0.85 0.90 0.95 1.00
Number of Instances
250
200
150
100
50
0
shape_un
(2)
(3)
Problematic Cases
S1
{"shape_un":"0.2"
"epith_size":"0.1"
"clump_thic":"0.8"}
A Misclassified Benign Instance
Figure 4
Decisions Comparison
T3
T2
T1
shape_un
clump_thic
epith_size
S3
Fixed Most Cases
Left Subtree (Benign)
Right Subtree (Benign)
Left Subtree (Malignant)
Right Subtree (Malignant)

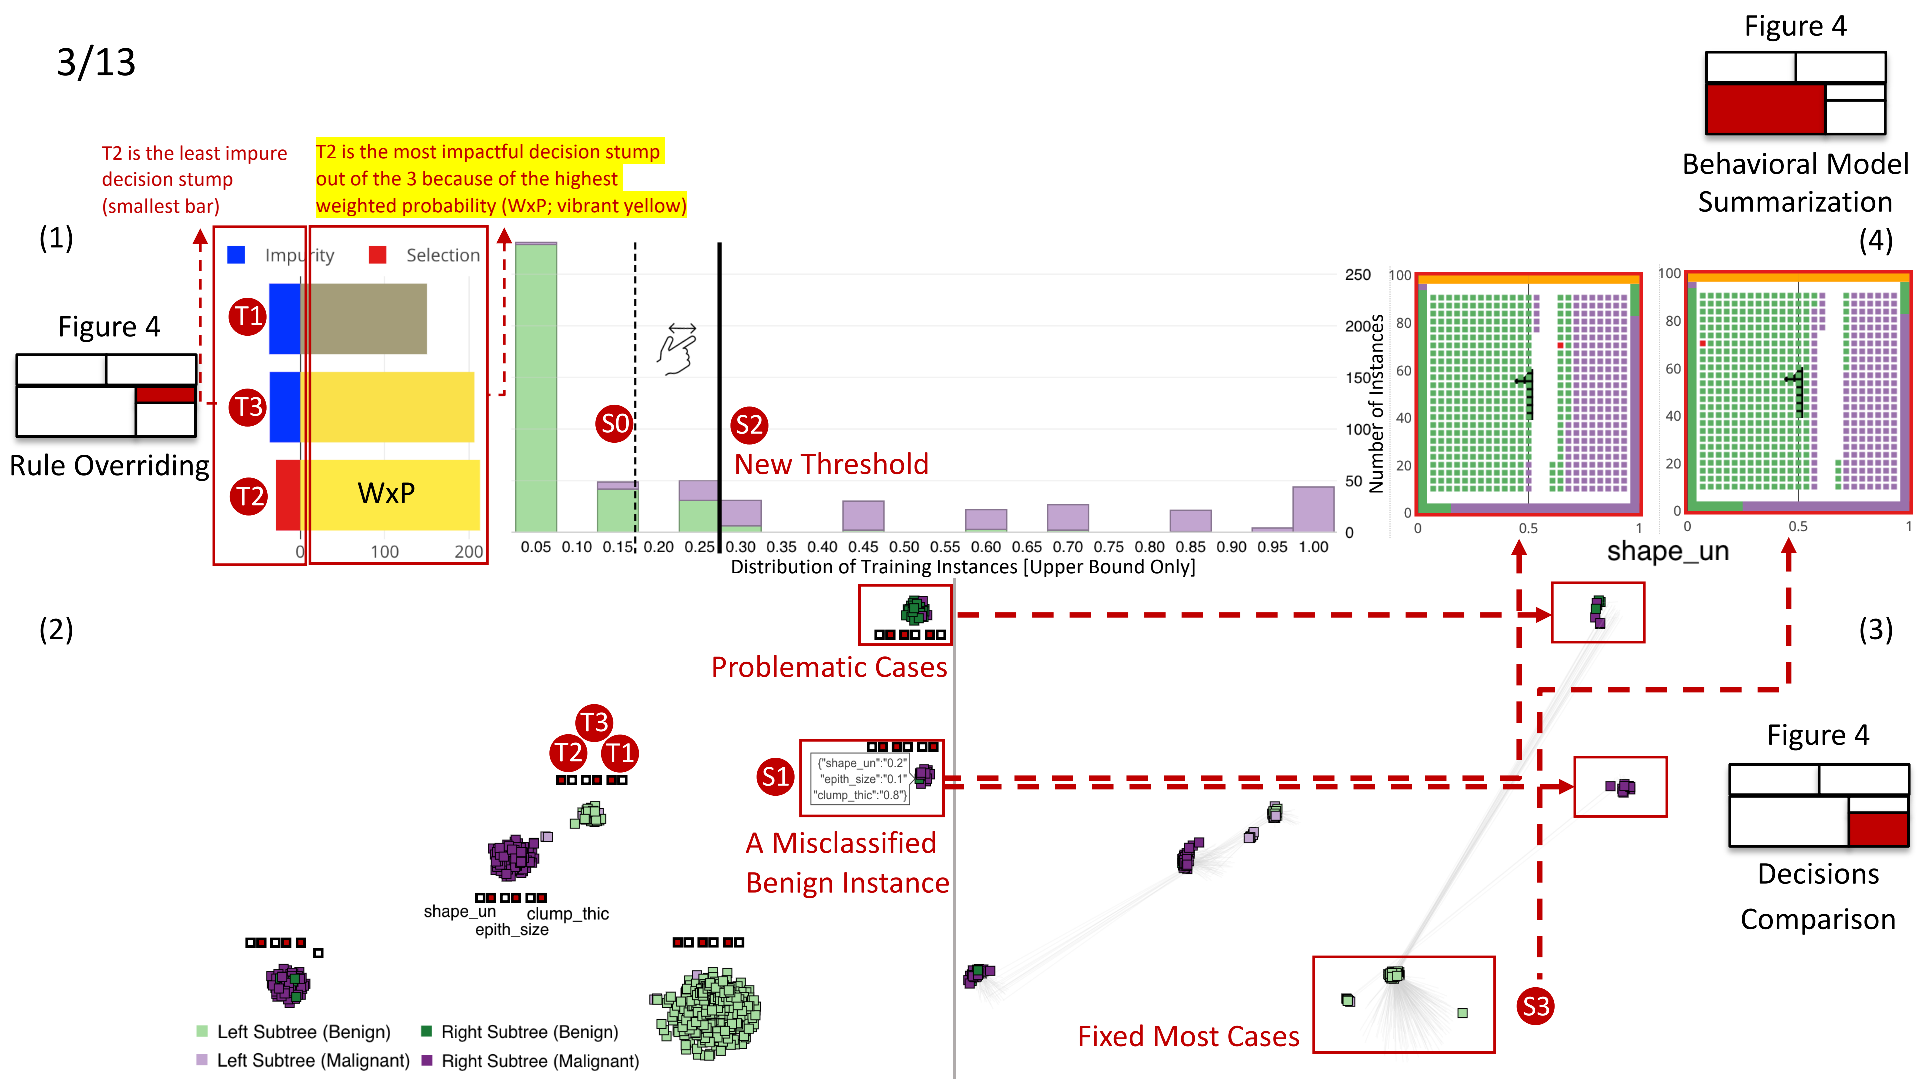

Figure 4
Behavioral Model Summarization
T2 is the least impure decision stump (smallest bar)
T2 is the most impactful decision stump out of the 3 because of the highest weighted probability (WxP; vibrant yellow)
(1)
Figure 4
Rule Overriding
Impurity
Selection
T1
T3
T2
WxP
0
100
200
S0
S2
New Threshold
0.05 0.10 0.15 0.20 0.25 0.30 0.35 0.40 0.45 0.50 0.55 0.60 0.65 0.70 0.75 0.80 0.85 0.90 0.95 1.00
Distribution of Training Instances [Upper Bound Only]
250
200
150
100
50
0
Number of Instances
(4)
shape_un
(2)
Problematic Cases
(3)
T3
T2
T1
S1
{"shape_un":"0.2"
"epith_size":"0.1"
"clump_thic":"0.8"}
A Misclassified Benign Instance
Figure 4
Decisions Comparison
shape_un
clump_thic
epith_size
Fixed Most Cases
S3
Left Subtree (Benign)
Right Subtree (Benign)
Left Subtree (Malignant)
Right Subtree (Malignant)

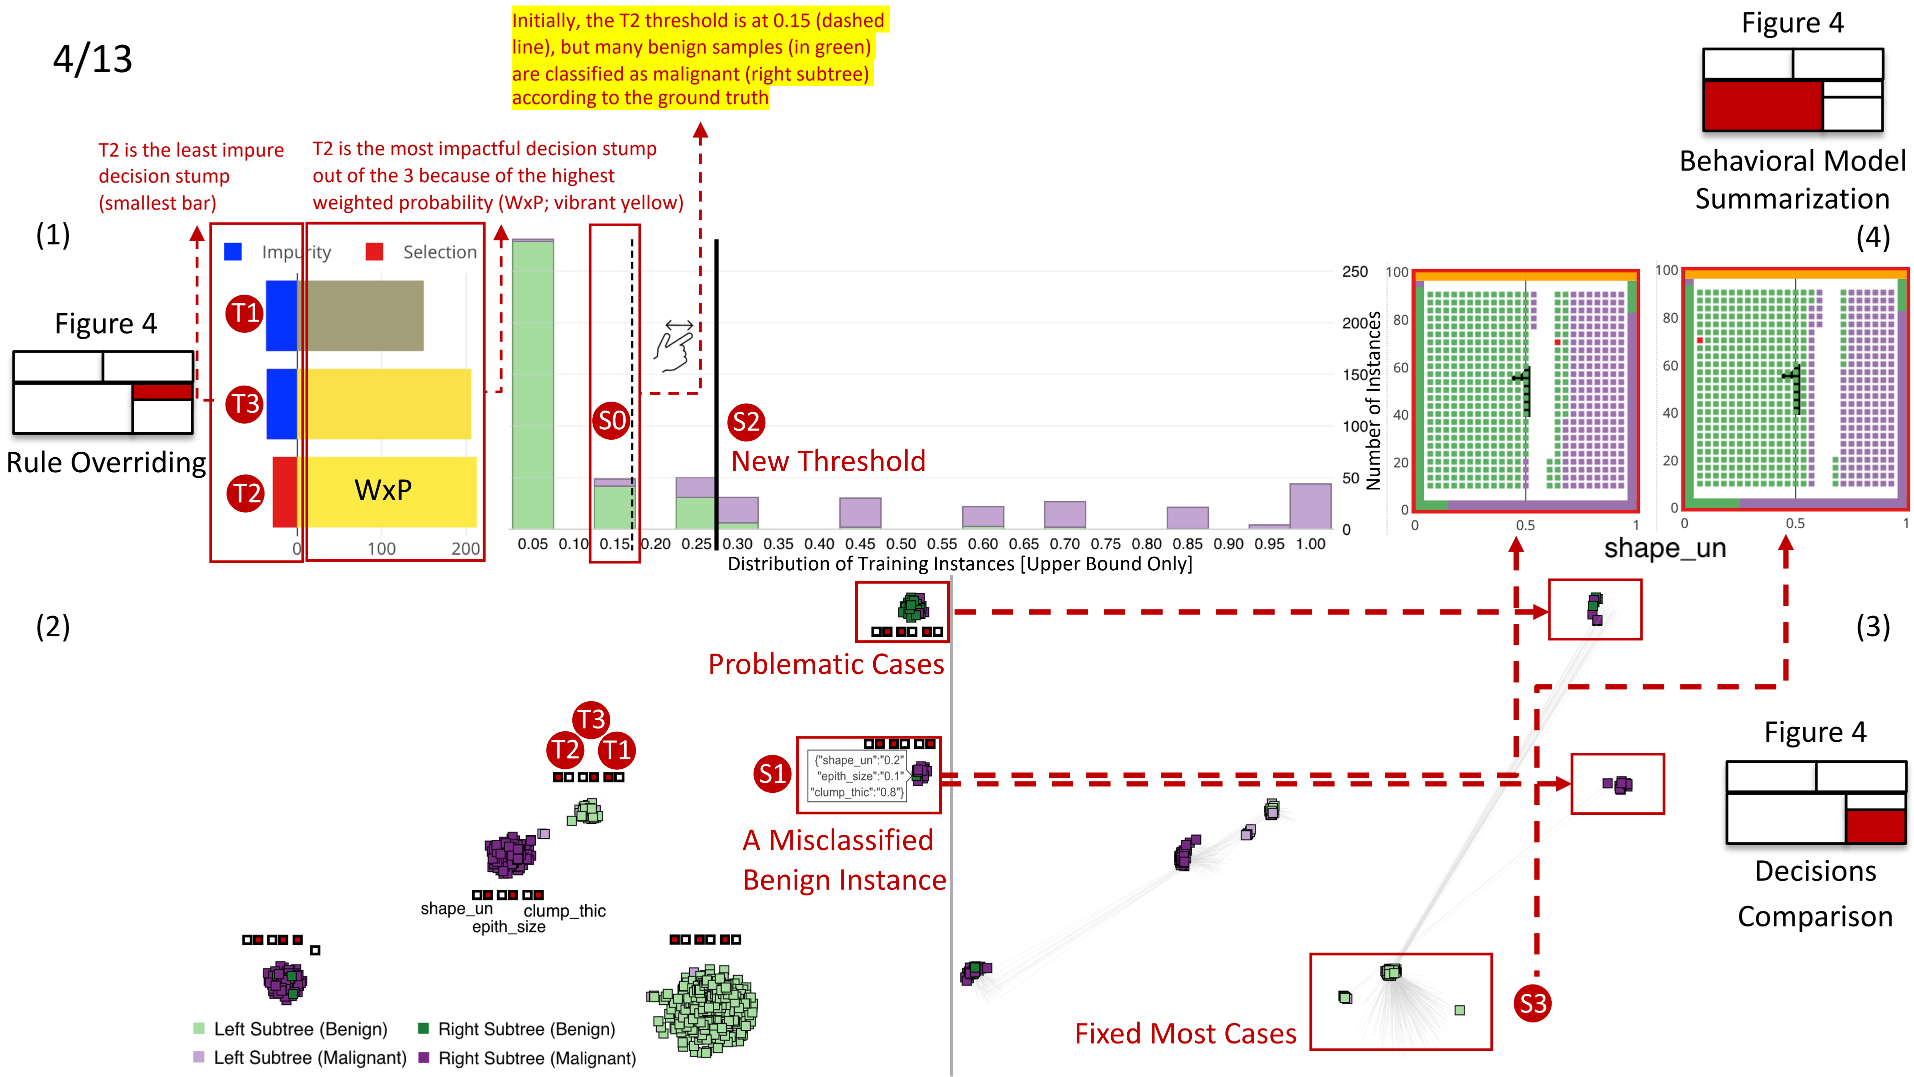

4/13
Initially, the T2 threshold is at 0.15 (dashed line), but many benign samples (in green) are classified as malignant (right subtree) according to the ground truth
T2 is the least impure decision stump (smallest bar)
T2 is the most impactful decision stump out of the 3 because of the highest weighted probability (WxP; vibrant yellow)
Figure 4
Behavioral Model Summarization
(1)
(4)
Figure 4
Rule Overriding
Impurity
Selection
T1
T3
T2
WxP
0
100
200
S0
S2
New Threshold
0.05 0.10 0.15 0.20 0.25 0.30 0.35 0.40 0.45 0.50 0.55 0.60 0.65 0.70 0.75 0.80 0.85 0.90 0.95 1.00
Distribution of Training Instances [Upper Bound Only]
Number of Instances
250
200
150
100
50
0
shape_un
(2)
(3)
Problematic Cases
S1
{"shape_un":"0.2"
"epith_size":"0.1"
"clump_thic":"0.8"}
A Misclassified Benign Instance
Figure 4
Decisions Comparison
shape_un
epith_size
clump_thic
S3
Fixed Most Cases
Left Subtree (Benign)
Right Subtree (Benign)
Left Subtree (Malignant)
Right Subtree (Malignant)

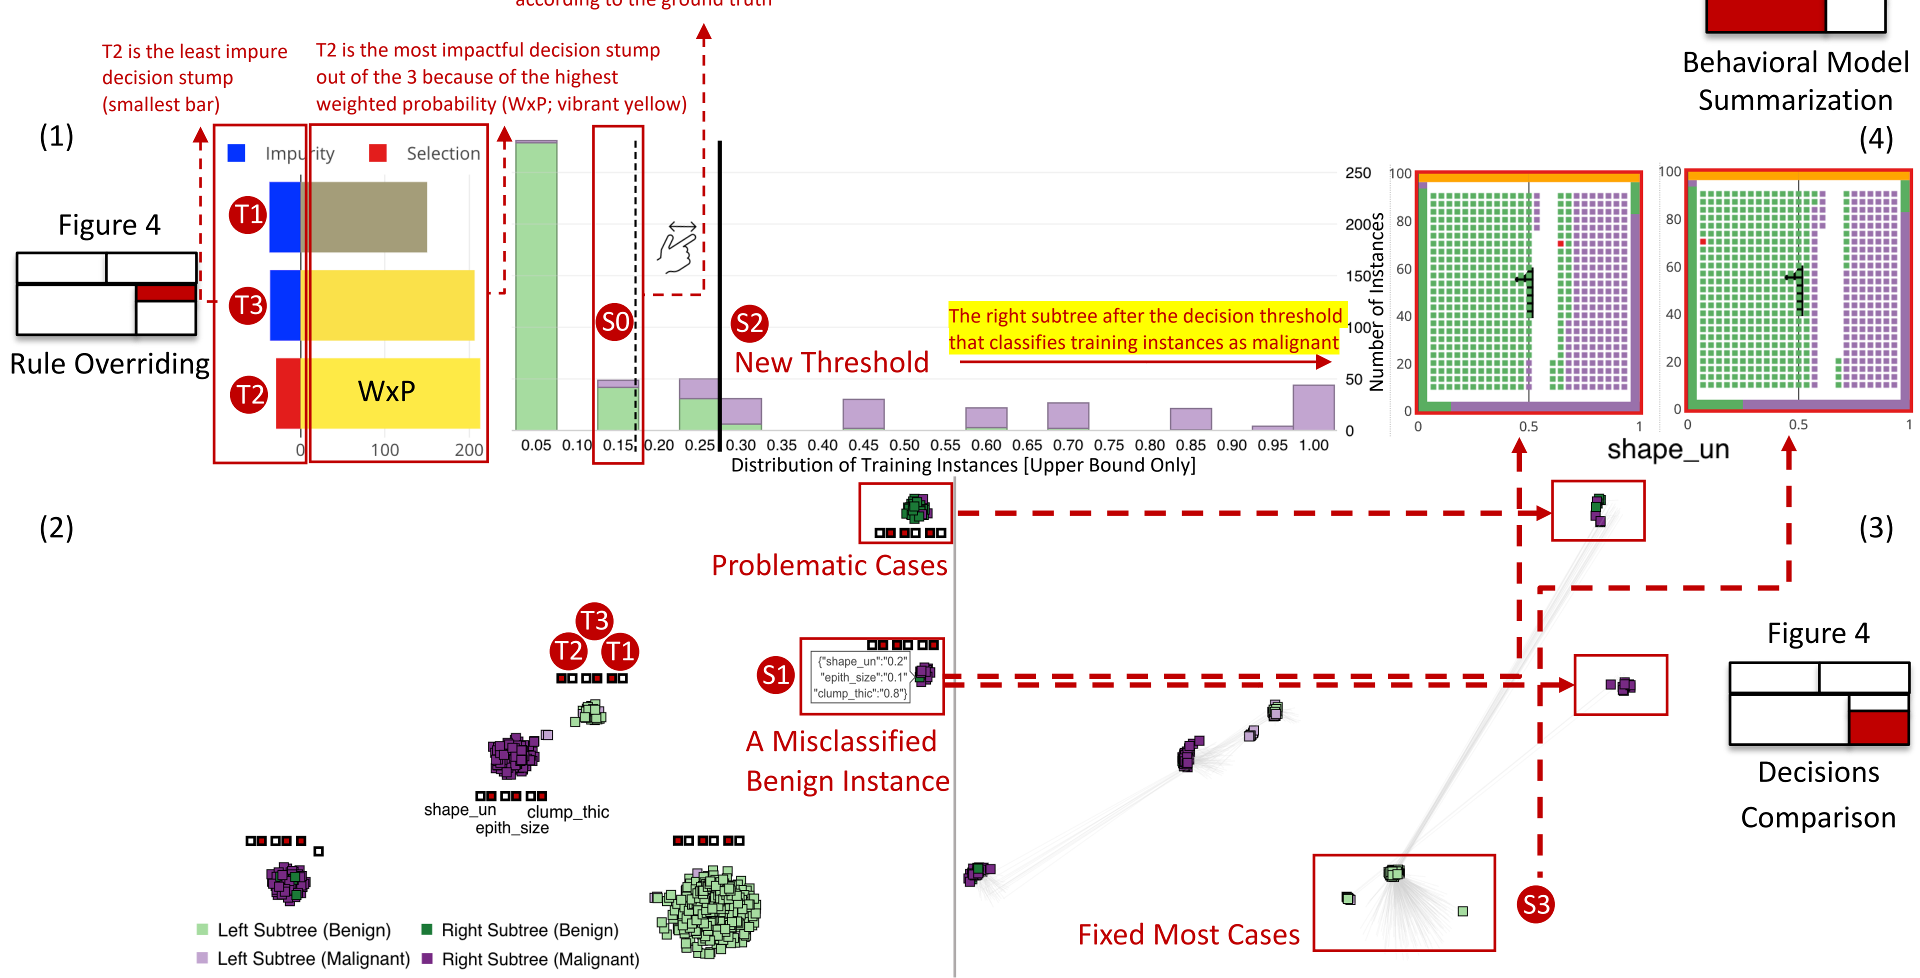

Initially, the T2 threshold is at 0.15 (dashed line), but many benign samples (in green) are classified as malignant (right subtree) according to the ground truth
T2 is the least impure decision stump (smallest bar)
T2 is the most impactful decision stump out of the 3 because of the highest weighted probability (WxP; vibrant yellow)
Figure 4
Behavioral Model Summarization
(1)
(4)
Figure 4
Rule Overriding
Impurity
Selection
T1
T3
T2
WxP
0
100
200
S0
S2
New Threshold
The right subtree after the decision threshold that classifies training instances as malignant
Distribution of Training Instances [Upper Bound Only]
Number of Instances
shape_un
(2)
(3)
Problematic Cases
S1
{"shape_un":"0.2" "epith_size":"0.1" "clump_thic":"0.8"}
A Misclassified Benign Instance
Figure 4
Decisions Comparison
shape_un
epith_size
clump_thic
Fixed Most Cases
S3
Left Subtree (Benign)
Right Subtree (Benign)
Left Subtree (Malignant)
Right Subtree (Malignant)

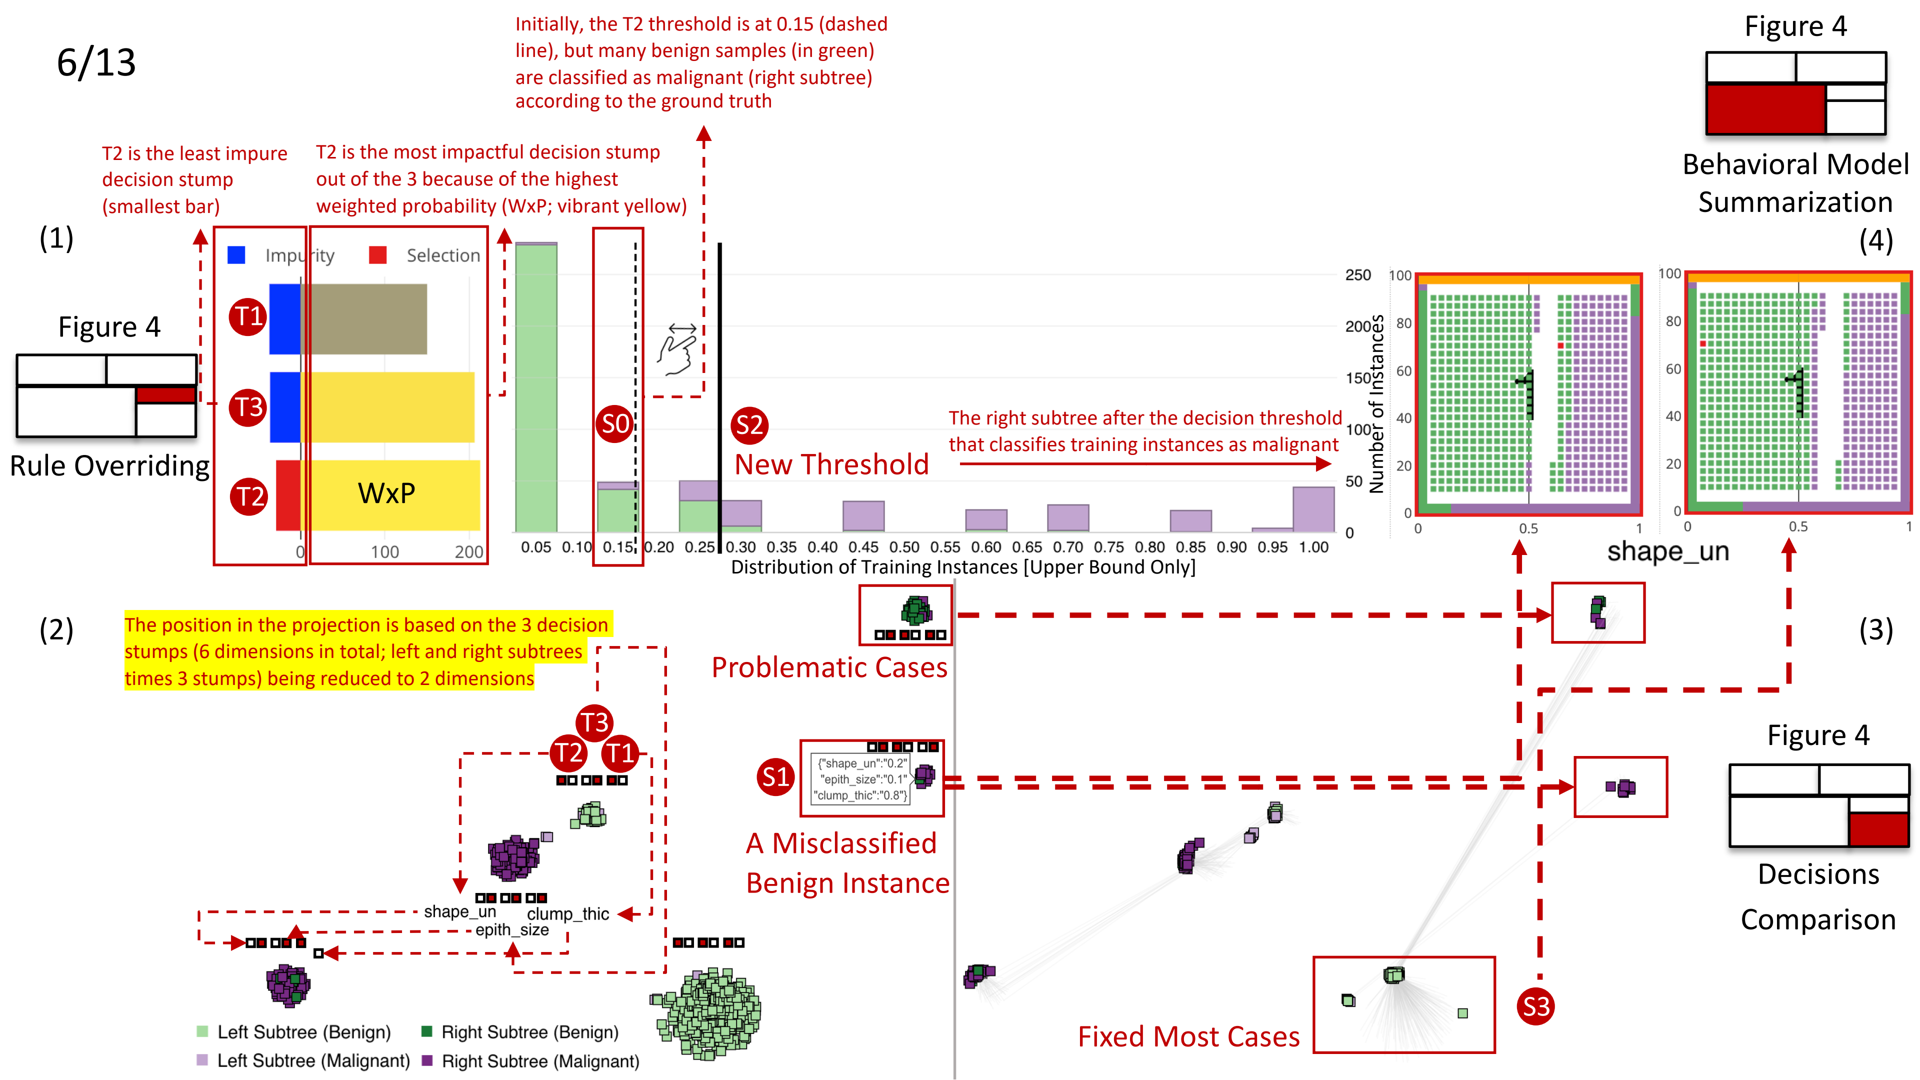
6/13
Initially, the T2 threshold is at 0.15 (dashed line), but many benign samples (in green) are classified as malignant (right subtree) according to the ground truth
Figure 4
Behavioral Model Summarization
T2 is the least impure decision stump (smallest bar)
T2 is the most impactful decision stump out of the 3 because of the highest weighted probability (WxP; vibrant yellow)
(1)
(4)
Impurity
Selection
T1
T3
T2
WxP
0
100
200
Figure 4
Rule Overriding
S0
S2
New Threshold
The right subtree after the decision threshold that classifies training instances as malignant
0.05 0.10 0.15 0.20 0.25 0.30 0.35 0.40 0.45 0.50 0.55 0.60 0.65 0.70 0.75 0.80 0.85 0.90 0.95 1.00
Distribution of Training Instances [Upper Bound Only]
Number of Instances
250
200
150
100
50
0
shape_un
(2)
The position in the projection is based on the 3 decision stumps (6 dimensions in total; left and right subtrees times 3 stumps) being reduced to 2 dimensions
Problematic Cases
(3)
S1
{"shape_un":"0.2"
"epith_size":"0.1"
"clump_thic":"0.8"}
A Misclassified Benign Instance
Figure 4
Decisions Comparison
shape_un
clump_thic
epith_size
S3
Fixed Most Cases
Left Subtree (Benign)
Right Subtree (Benign)
Left Subtree (Malignant)
Right Subtree (Malignant)

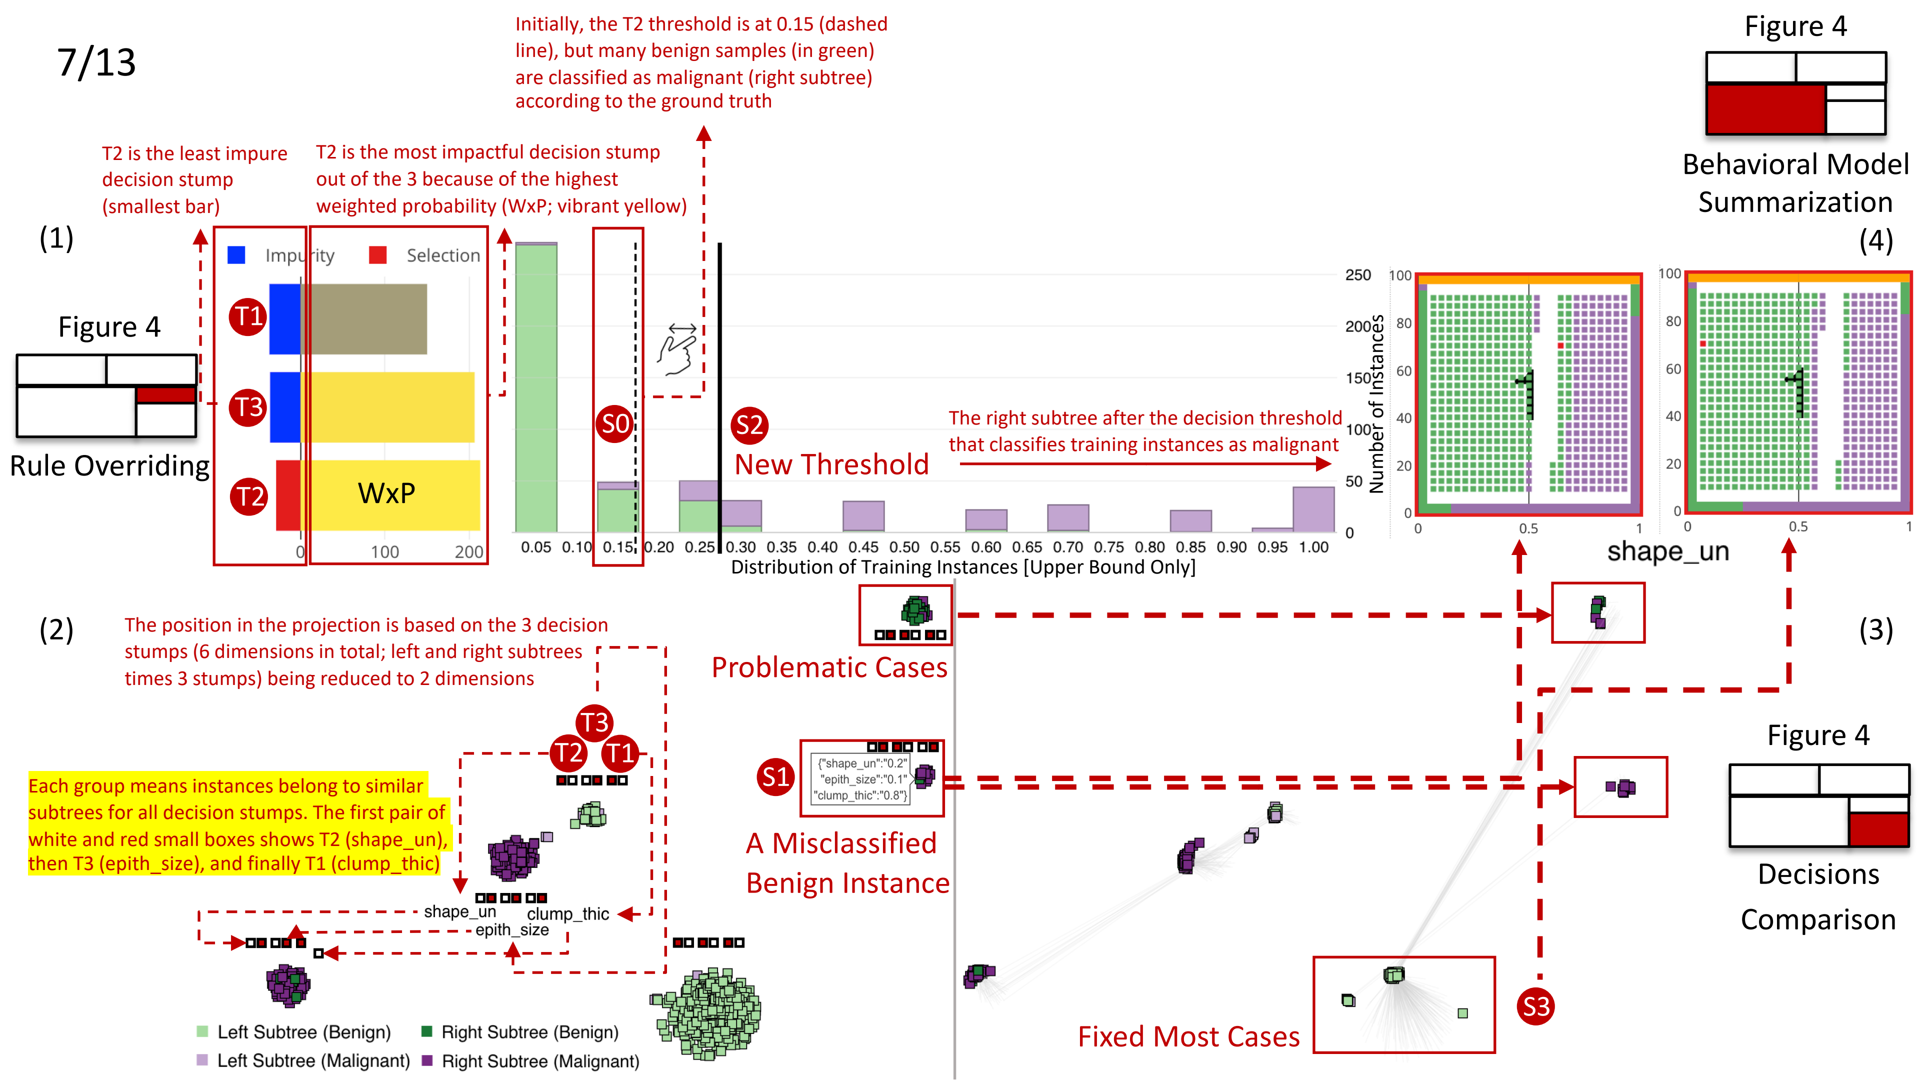
Initially, the T2 threshold is at 0.15 (dashed line), but many benign samples (in green) are classified as malignant (right subtree) according to the ground truth
Figure 4
Behavioral Model Summarization
(4)
T2 is the least impure decision stump (smallest bar)
T2 is the most impactful decision stump out of the 3 because of the highest weighted probability (WxP; vibrant yellow)
(1)
Impurity
Selection
T1
T3
T2
WxP
Figure 4
Rule Overriding
S0
S2
New Threshold
The right subtree after the decision threshold that classifies training instances as malignant
Number of Instances
Distribution of Training Instances [Upper Bound Only]
shape_un
(2)
The position in the projection is based on the 3 decision stumps (6 dimensions in total; left and right subtrees times 3 stumps) being reduced to 2 dimensions
Problematic Cases
(3)
Each group means instances belong to similar subtrees for all decision stumps. The first pair of white and red small boxes shows T2 (shape_un), then T3 (epith_size), and finally T1 (clump_thic)
S1
{"shape_un":"0.2" "epith_size":"0.1" "clump_thic":"0.8"}
A Misclassified Benign Instance
Figure 4
Decisions Comparison
shape_un
clump_thic
epith_size
Fixed Most Cases
S3
Left Subtree (Benign)
Right Subtree (Benign)
Left Subtree (Malignant)
Right Subtree (Malignant)

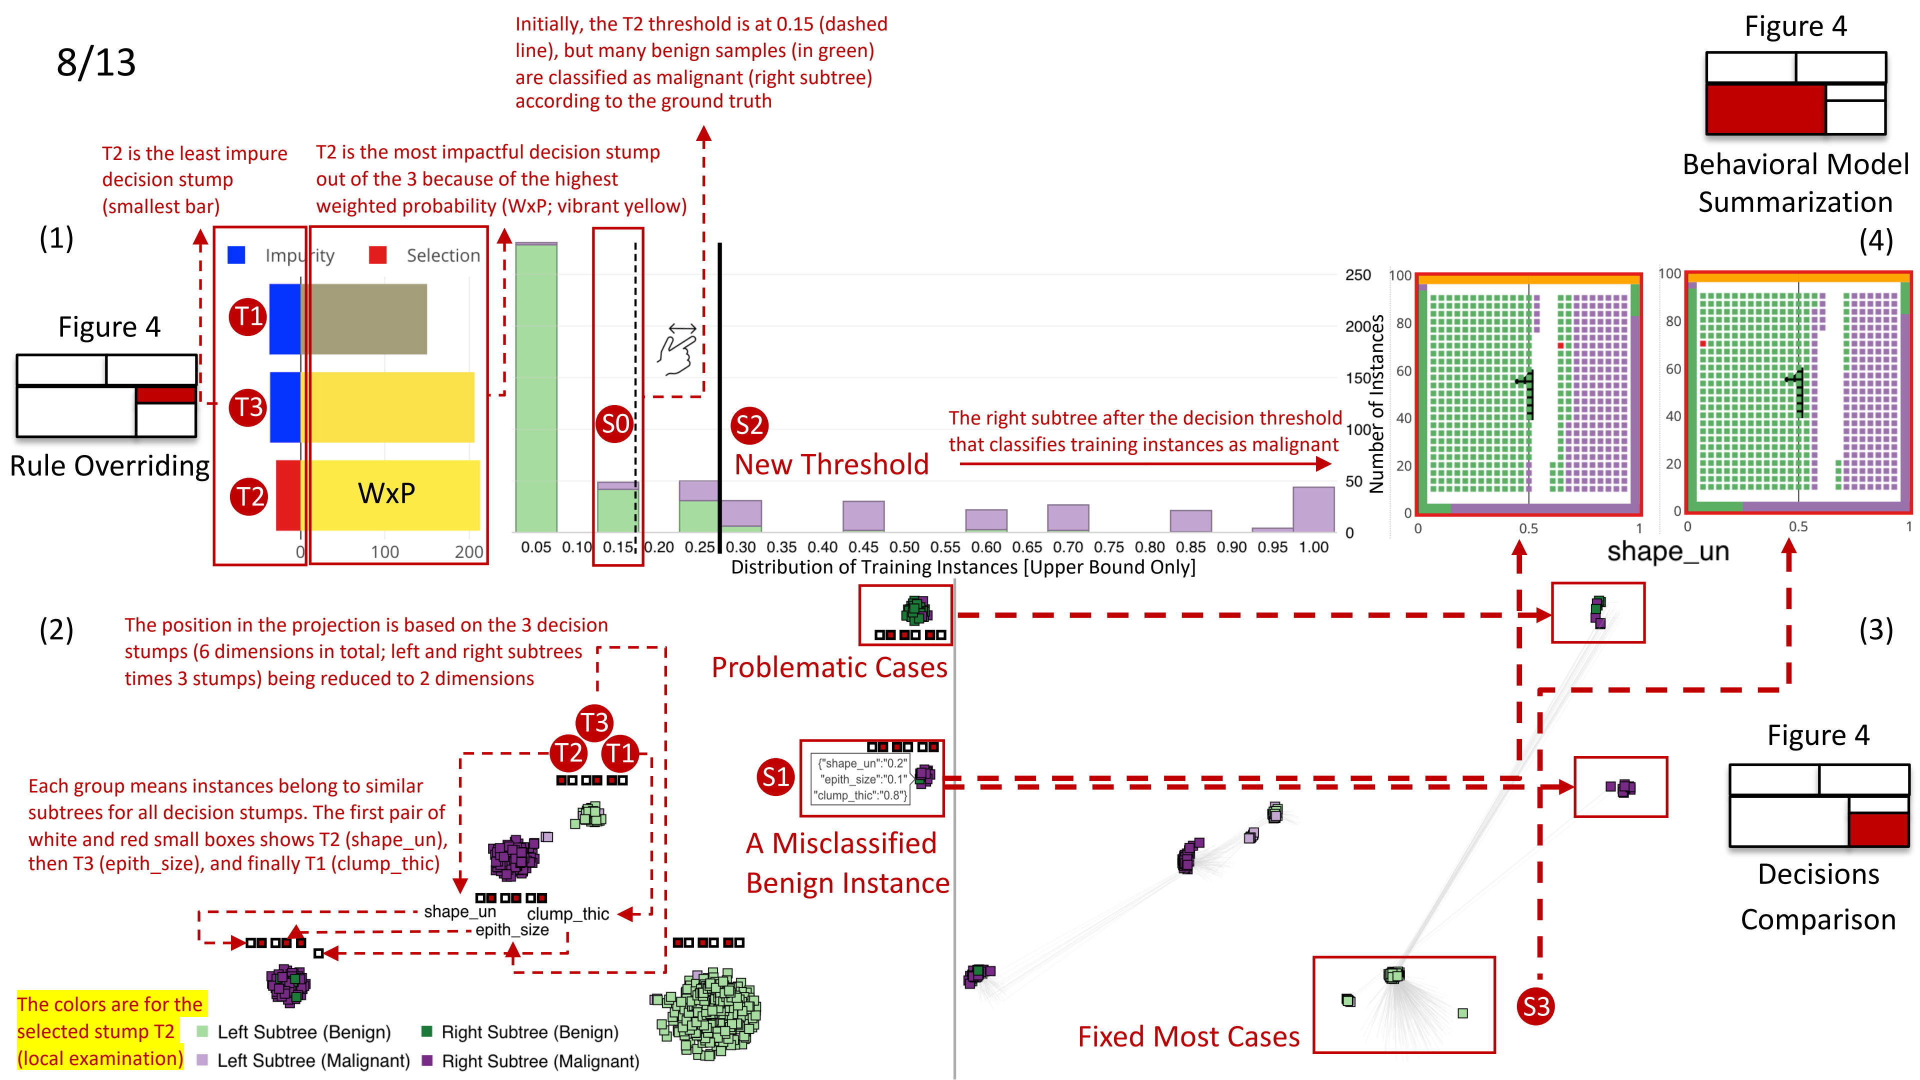
Initially, the T2 threshold is at 0.15 (dashed line), but many benign samples (in green) are classified as malignant (right subtree) according to the ground truth
Figure 4
Behavioral Model Summarization
T2 is the least impure decision stump (smallest bar)
T2 is the most impactful decision stump out of the 3 because of the highest weighted probability (WxP; vibrant yellow)
(1)
(4)
Impurity
Selection
T1
T3
T2
WxP
Figure 4
Rule Overriding
S0
S2
New Threshold
The right subtree after the decision threshold that classifies training instances as malignant
Number of Instances
Distribution of Training Instances [Upper Bound Only]
shape_un
(2)
(3)
The position in the projection is based on the 3 decision stumps (6 dimensions in total; left and right subtrees times 3 stumps) being reduced to 2 dimensions
Problematic Cases
Each group means instances belong to similar subtrees for all decision stumps. The first pair of white and red small boxes shows T2 (shape_un), then T3 (epith_size), and finally T1 (clump_thic)
S1
{"shape_un":"0.2" "epith_size":"0.1" "clump_thic":"0.8"}
A Misclassified Benign Instance
Figure 4
Decisions Comparison
shape_un
epith_size
clump_thic
S3
Fixed Most Cases
The colors are for the selected stump T2 (local examination)
Left Subtree (Benign)
Right Subtree (Benign)
Left Subtree (Malignant)
Right Subtree (Malignant)

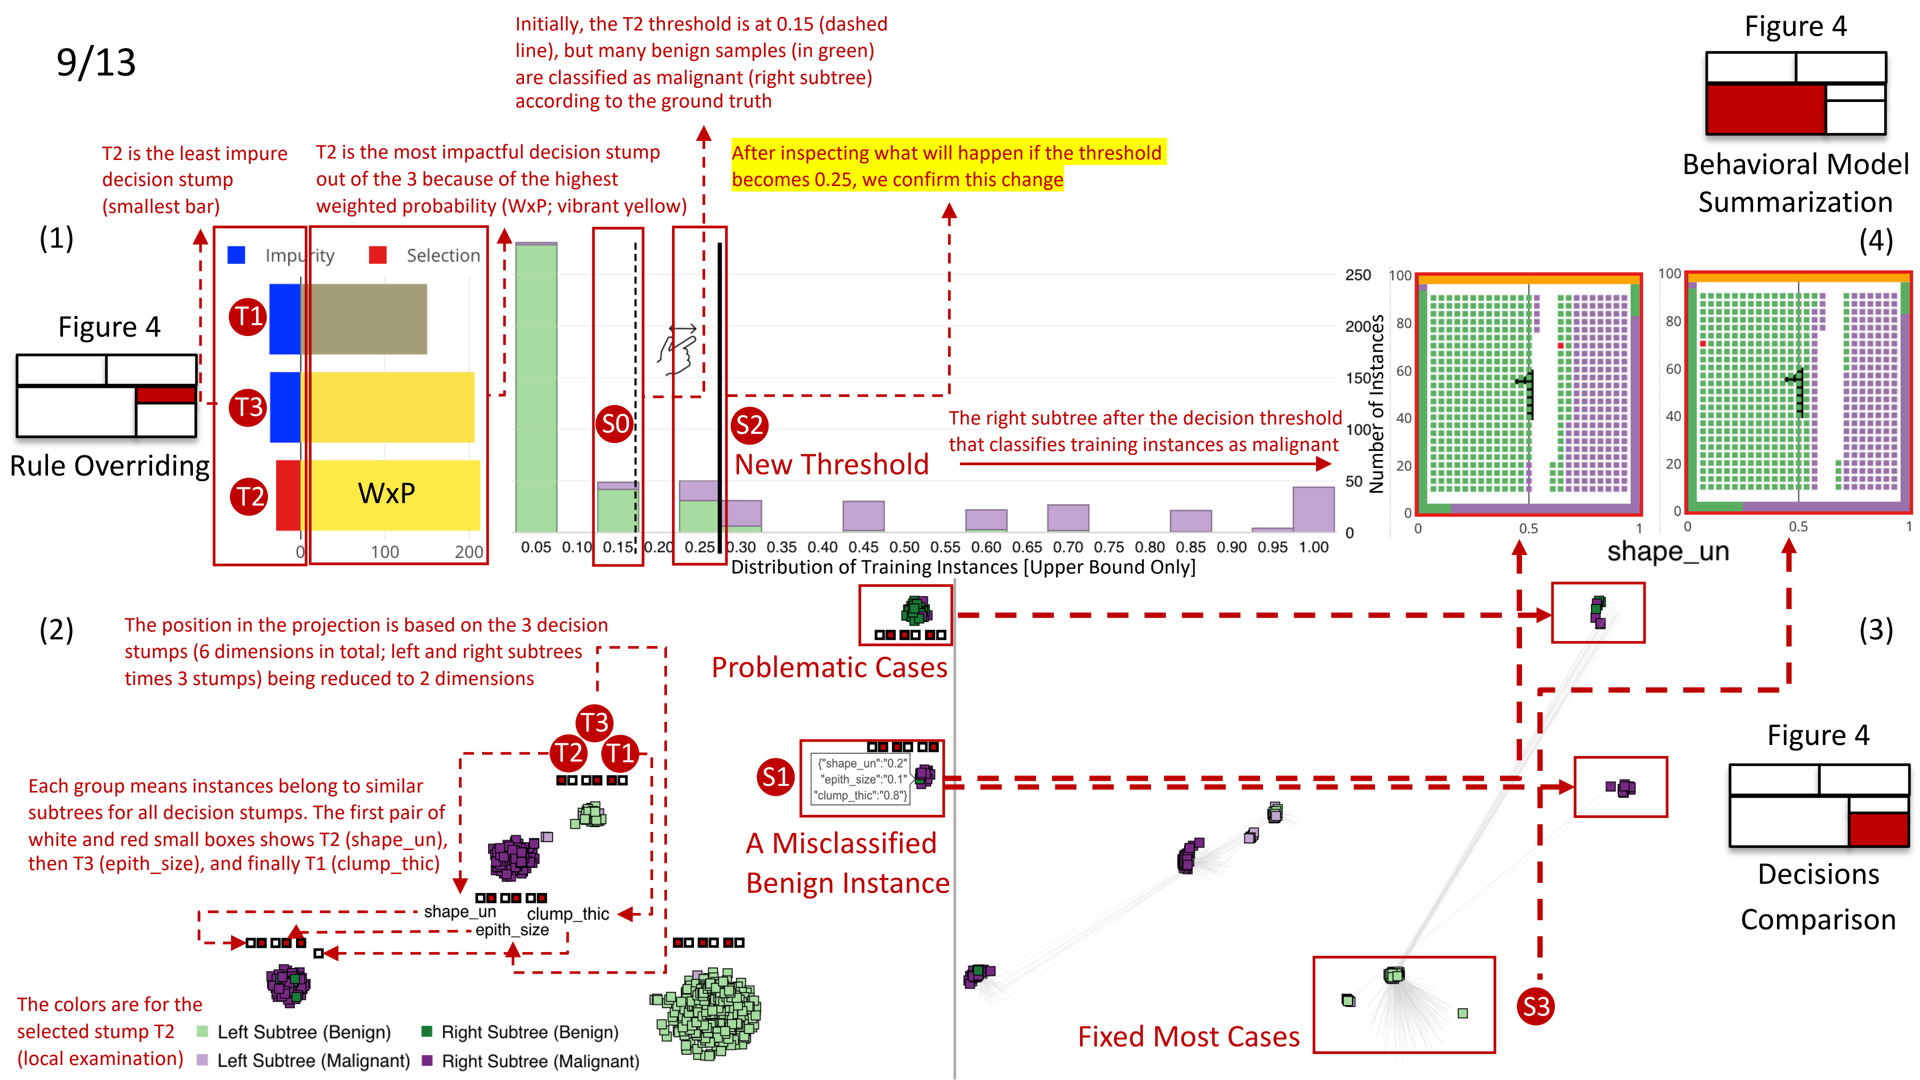
Initially, the T2 threshold is at 0.15 (dashed line), but many benign samples (in green) are classified as malignant (right subtree) according to the ground truth
Figure 4
Behavioral Model Summarization
T2 is the least impure decision stump (smallest bar)
T2 is the most impactful decision stump out of the 3 because of the highest weighted probability (WxP; vibrant yellow)
After inspecting what will happen if the threshold becomes 0.25, we confirm this change
(1)
(4)
Impurity
Selection
T1
T3
T2
WxP
Figure 4
Rule Overriding
S0
S2
New Threshold
The right subtree after the decision threshold that classifies training instances as malignant
Number of Instances
Distribution of Training Instances [Upper Bound Only]
shape_un
(2)
(3)
The position in the projection is based on the 3 decision stumps (6 dimensions in total; left and right subtrees times 3 stumps) being reduced to 2 dimensions
Problematic Cases
Each group means instances belong to similar subtrees for all decision stumps. The first pair of white and red small boxes shows T2 (shape_un), then T3 (epith_size), and finally T1 (clump_thic)
S1
{"shape_un":"0.2" "epith_size":"0.1" "clump_thic":"0.8"}
A Misclassified Benign Instance
Figure 4
Decisions Comparison
shape_un
epith_size
clump_thic
The colors are for the selected stump T2 (local examination)
Left Subtree (Benign)
Right Subtree (Benign)
Left Subtree (Malignant)
Right Subtree (Malignant)
Fixed Most Cases
S3

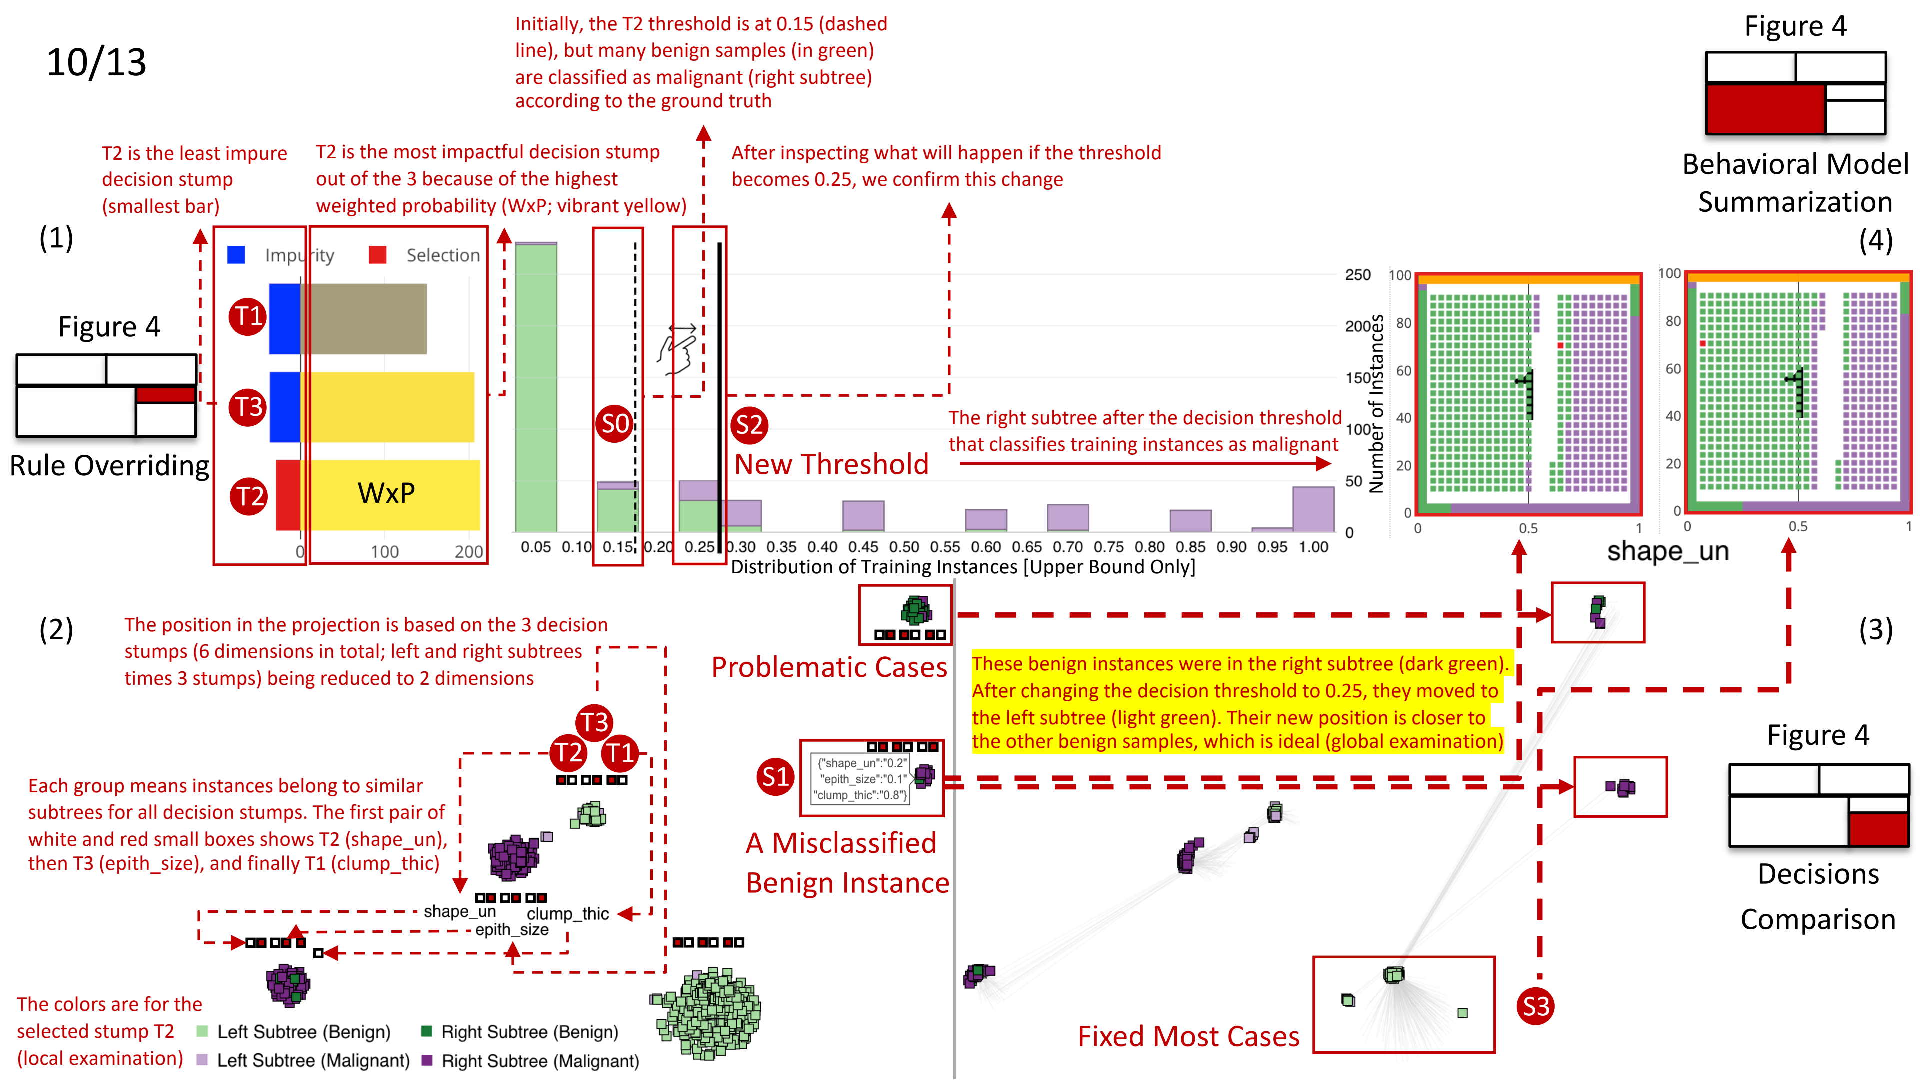
10/13
Initially, the T2 threshold is at 0.15 (dashed line), but many benign samples (in green) are classified as malignant (right subtree) according to the ground truth
Figure 4
Behavioral Model Summarization
T2 is the least impure decision stump (smallest bar)
T2 is the most impactful decision stump out of the 3 because of the highest weighted probability (WxP; vibrant yellow)
After inspecting what will happen if the threshold becomes 0.25, we confirm this change
(1)
(4)
Figure 4
Rule Overriding
Impurity
Selection
T1
T3
T2
WxP
S0
S2
New Threshold
The right subtree after the decision threshold that classifies training instances as malignant
Number of Instances
Distribution of Training Instances [Upper Bound Only]
shape_un
(2)
(3)
The position in the projection is based on the 3 decision stumps (6 dimensions in total; left and right subtrees times 3 stumps) being reduced to 2 dimensions
Problematic Cases
These benign instances were in the right subtree (dark green). After changing the decision threshold to 0.25, they moved to the left subtree (light green). Their new position is closer to the other benign samples, which is ideal (global examination)
Figure 4
Decisions Comparison
Each group means instances belong to similar subtrees for all decision stumps. The first pair of white and red small boxes shows T2 (shape_un), then T3 (epith_size), and finally T1 (clump_thic)
S1
{"shape_un":"0.2" "epith_size":"0.1" "clump_thic":"0.8"}
A Misclassified Benign Instance
shape_un
epith_size
clump_thic
S3
Fixed Most Cases
The colors are for the selected stump T2 (local examination)
Left Subtree (Benign)
Right Subtree (Benign)
Left Subtree (Malignant)
Right Subtree (Malignant)

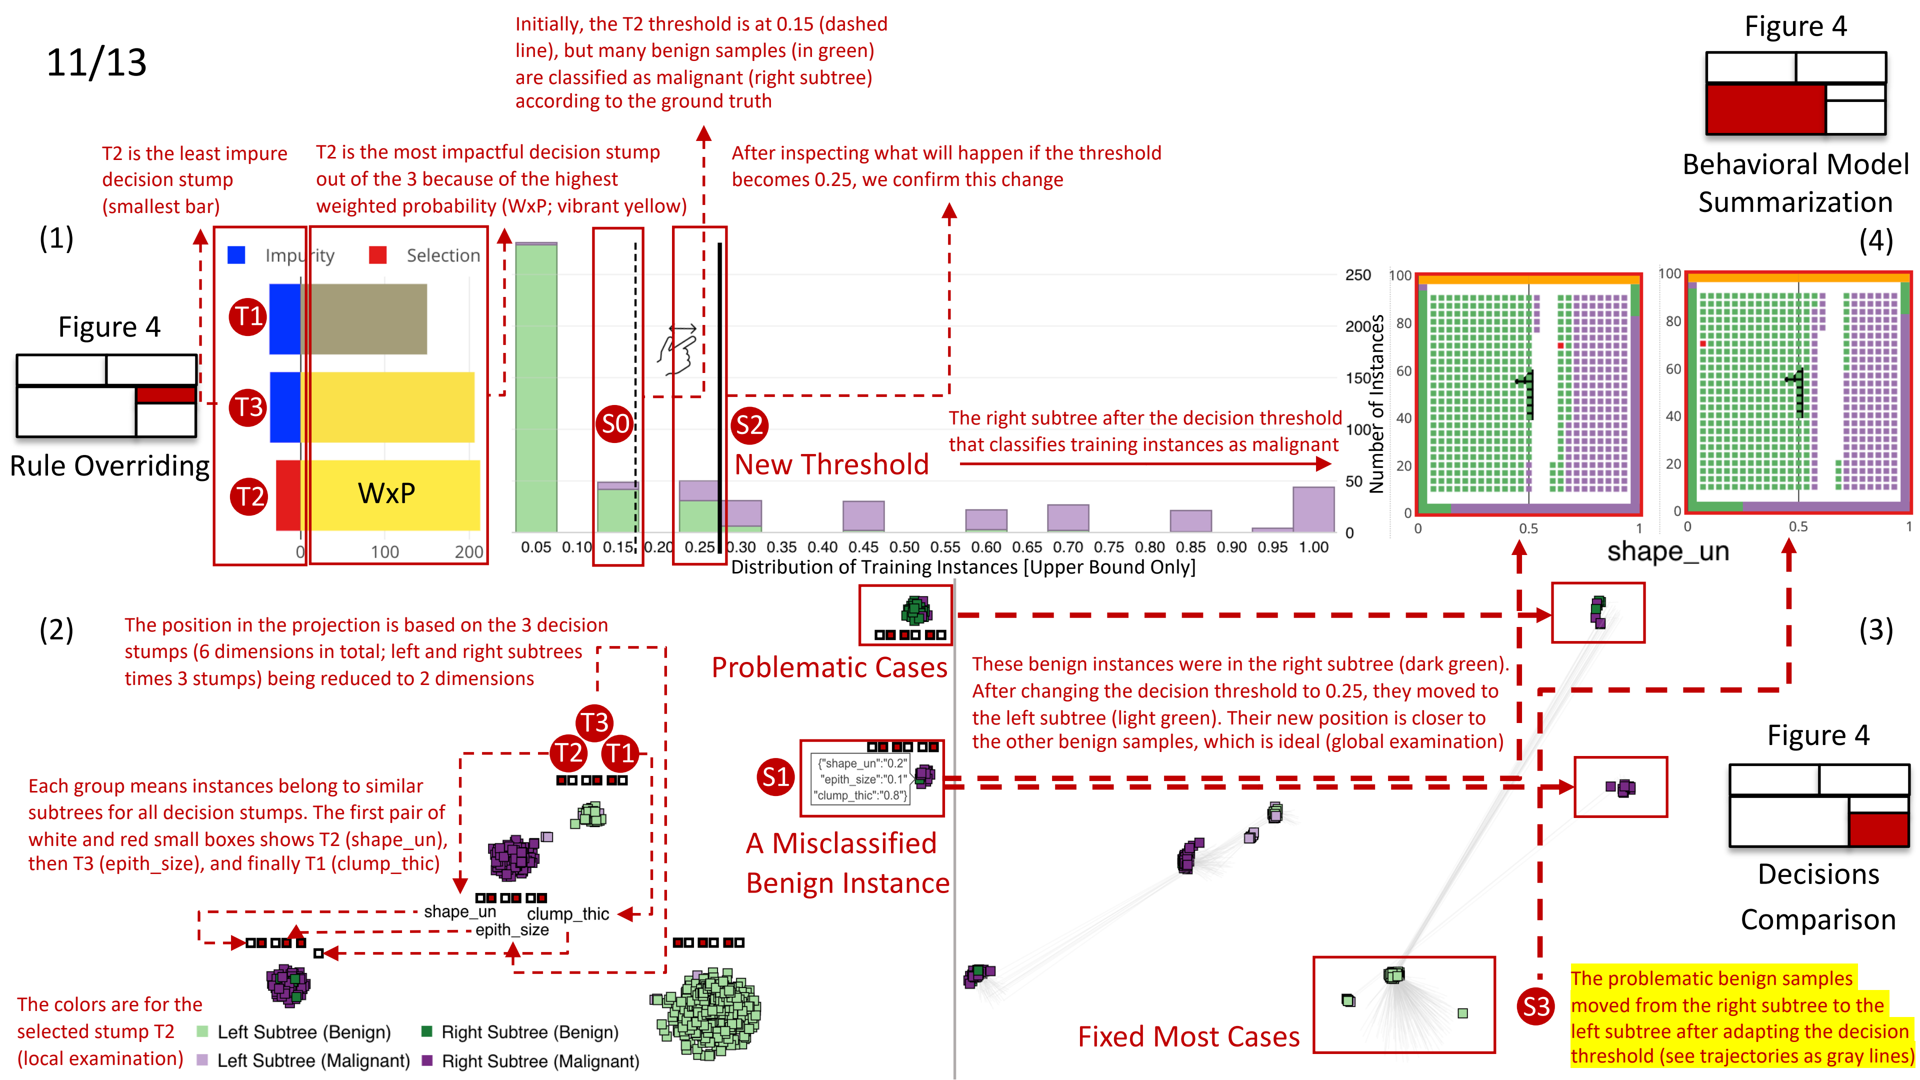

Figure 4
Behavioral Model Summarization
(1)
(2)
(3)
(4)
Figure 4
Rule Overriding
Figure 4
Decisions Comparison
T2 is the least impure decision stump (smallest bar)
T2 is the most impactful decision stump out of the 3 because of the highest weighted probability (WxP; vibrant yellow)
Initially, the T2 threshold is at 0.15 (dashed line), but many benign samples (in green) are classified as malignant (right subtree) according to the ground truth
After inspecting what will happen if the threshold becomes 0.25, we confirm this change
Impurity
Selection
T1
T3
T2
WxP
S0
S2
New Threshold
The right subtree after the decision threshold that classifies training instances as malignant
Distribution of Training Instances [Upper Bound Only]
Number of Instances
shape_un
The position in the projection is based on the 3 decision stumps (6 dimensions in total; left and right subtrees times 3 stumps) being reduced to 2 dimensions
Each group means instances belong to similar subtrees for all decision stumps. The first pair of white and red small boxes shows T2 (shape_un), then T3 (epith_size), and finally T1 (clump_thic)
shape_un
epith_size
clump_thic
The colors are for the selected stump T2 (local examination)
Left Subtree (Benign)
Right Subtree (Benign)
Left Subtree (Malignant)
Right Subtree (Malignant)
Problematic Cases
These benign instances were in the right subtree (dark green). After changing the decision threshold to 0.25, they moved to the left subtree (light green). Their new position is closer to the other benign samples, which is ideal (global examination)
S1
{"shape_un":"0.2" "epith_size":"0.1" "clump_thic":"0.8"}
A Misclassified Benign Instance
Fixed Most Cases
S3
The problematic benign samples moved from the right subtree to the left subtree after adapting the decision threshold (see trajectories as gray lines)

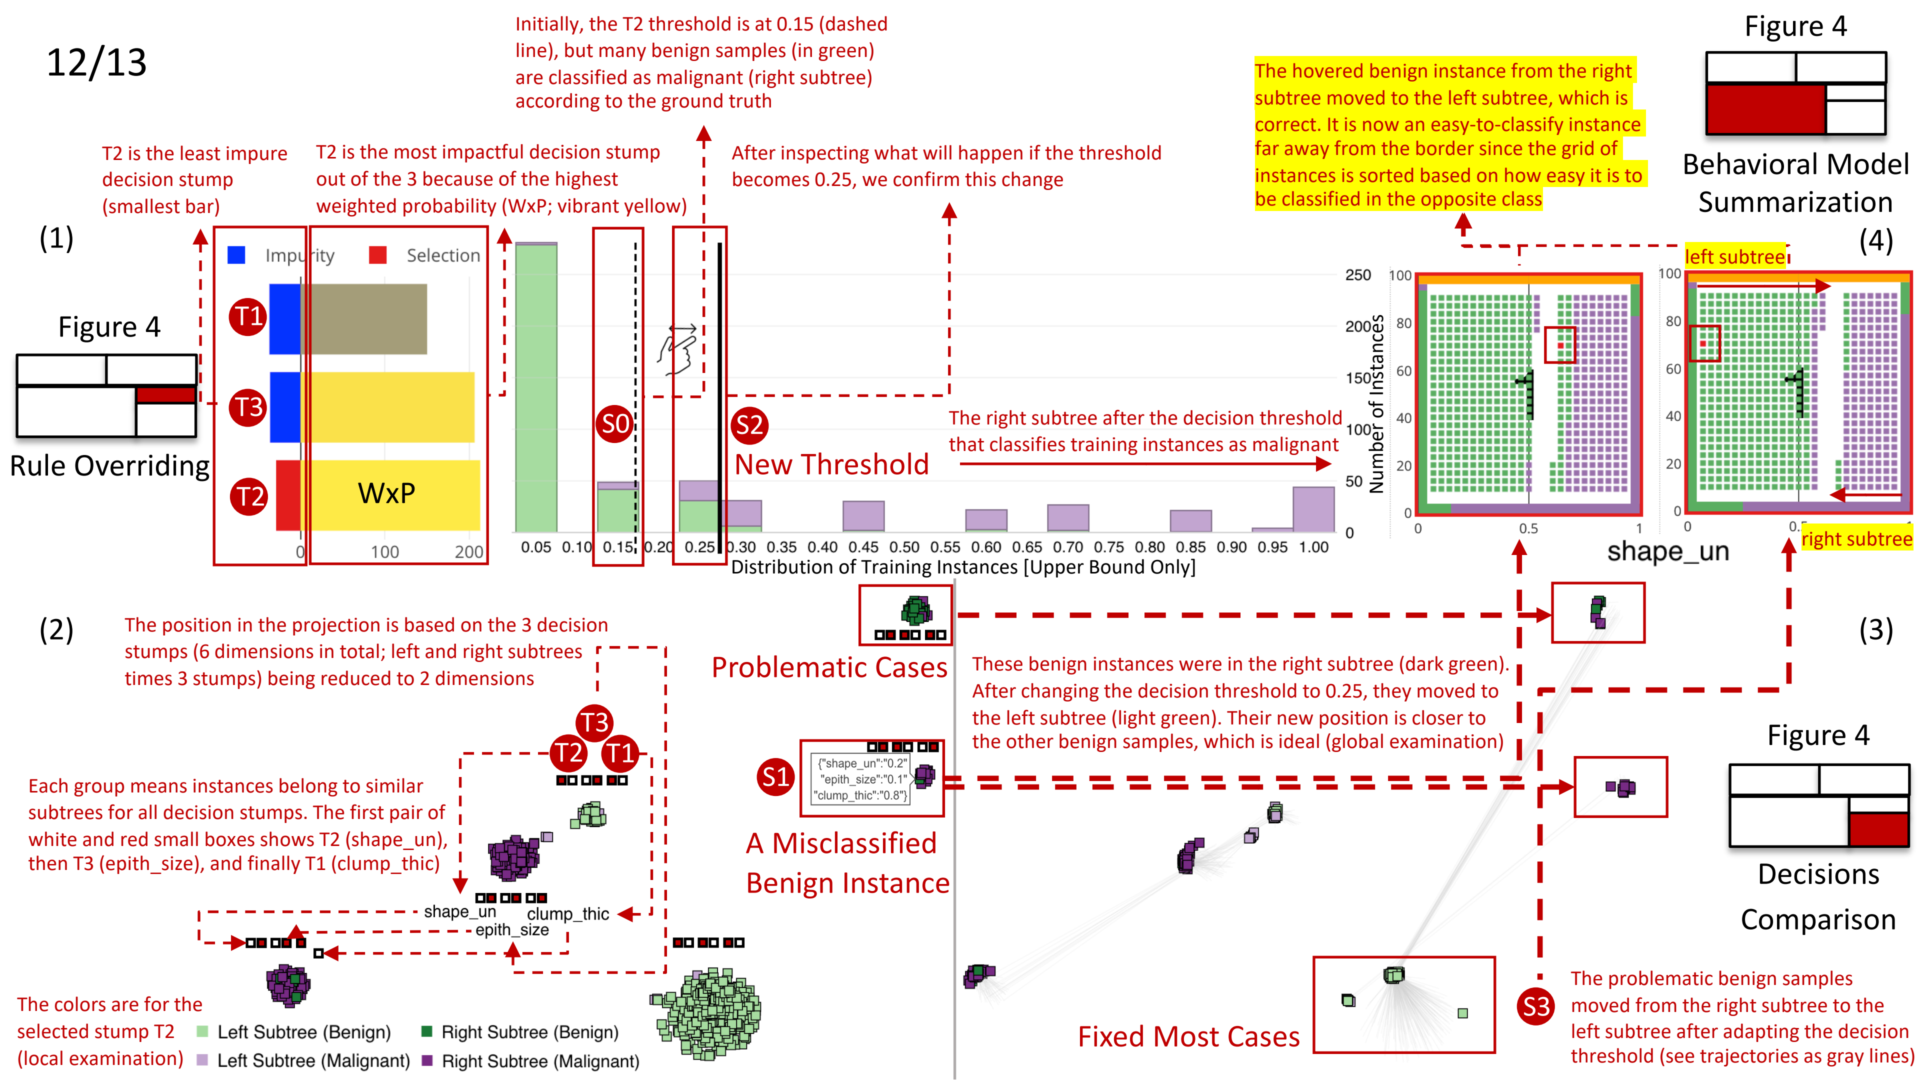
12/13
Initially, the T2 threshold is at 0.15 (dashed line), but many benign samples (in green) are classified as malignant (right subtree) according to the ground truth
Figure 4
Behavioral Model Summarization
The hovered benign instance from the right subtree moved to the left subtree, which is correct. It is now an easy-to-classify instance far away from the border since the grid of instances is sorted based on how easy it is to be classified in the opposite class
T2 is the least impure decision stump (smallest bar)
T2 is the most impactful decision stump out of the 3 because of the highest weighted probability (WxP; vibrant yellow)
After inspecting what will happen if the threshold becomes 0.25, we confirm this change
(1)
(4)
left subtree
right subtree
Figure 4
Rule Overriding
Impurity
Selection
T1
T3
T2
WxP
S0
S2
New Threshold
The right subtree after the decision threshold that classifies training instances as malignant
Number of Instances
Distribution of Training Instances [Upper Bound Only]
shape_un
(2)
(3)
The position in the projection is based on the 3 decision stumps (6 dimensions in total; left and right subtrees times 3 stumps) being reduced to 2 dimensions
Problematic Cases
These benign instances were in the right subtree (dark green). After changing the decision threshold to 0.25, they moved to the left subtree (light green). Their new position is closer to the other benign samples, which is ideal (global examination)
Each group means instances belong to similar subtrees for all decision stumps. The first pair of white and red small boxes shows T2 (shape_un), then T3 (epith_size), and finally T1 (clump_thic)
S1
{"shape_un":"0.2" "epith_size":"0.1" "clump_thic":"0.8"}
A Misclassified Benign Instance
Figure 4
Decisions Comparison
shape_un
epith_size
clump_thic
The colors are for the selected stump T2 (local examination)
Left Subtree (Benign)
Right Subtree (Benign)
Left Subtree (Malignant)
Right Subtree (Malignant)
Fixed Most Cases
S3
The problematic benign samples moved from the right subtree to the left subtree after adapting the decision threshold (see trajectories as gray lines)

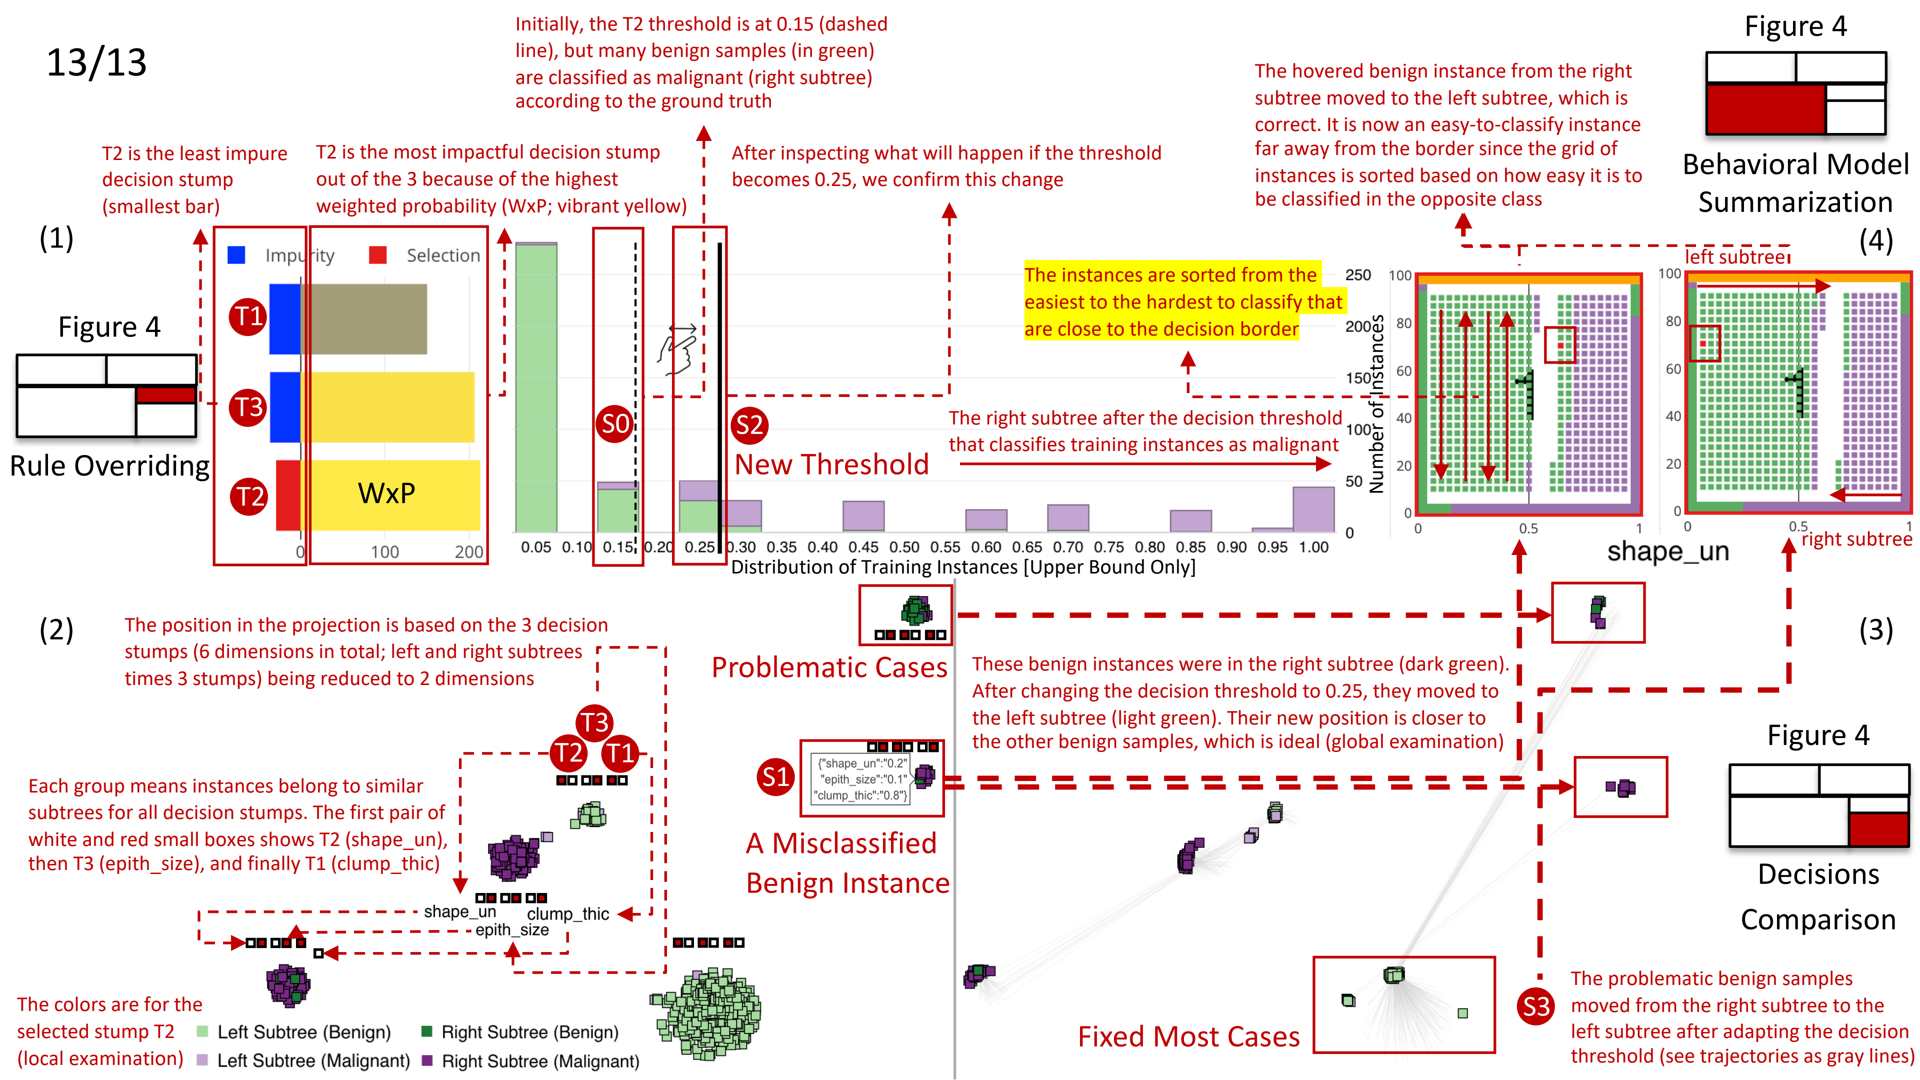
Initially, the T2 threshold is at 0.15 (dashed line), but many benign samples (in green) are classified as malignant (right subtree) according to the ground truth
Figure 4
The hovered benign instance from the right subtree moved to the left subtree, which is correct. It is now an easy-to-classify instance far away from the border since the grid of instances is sorted based on how easy it is to be classified in the opposite class
Behavioral Model Summarization
T2 is the least impure decision stump (smallest bar)
T2 is the most impactful decision stump out of the 3 because of the highest weighted probability (WxP; vibrant yellow)
After inspecting what will happen if the threshold becomes 0.25, we confirm this change
(1)
(4)
Impurity
Selection
The instances are sorted from the easiest to the hardest to classify that are close to the decision border
left subtree
Figure 4
Rule Overriding
T1
T3
T2
WxP
S0
S2
New Threshold
The right subtree after the decision threshold that classifies training instances as malignant
Number of Instances
Distribution of Training Instances [Upper Bound Only]
shape_un
right subtree
(2)
The position in the projection is based on the 3 decision stumps (6 dimensions in total; left and right subtrees times 3 stumps) being reduced to 2 dimensions
Problematic Cases
These benign instances were in the right subtree (dark green). After changing the decision threshold to 0.25, they moved to the left subtree (light green). Their new position is closer to the other benign samples, which is ideal (global examination)
(3)
Each group means instances belong to similar subtrees for all decision stumps. The first pair of white and red small boxes shows T2 (shape_un), then T3 (epith_size), and finally T1 (clump_thic)
S1
{"shape_un":"0.2" "epith_size":"0.1" "clump_thic":"0.8"}
A Misclassified Benign Instance
Figure 4
Decisions Comparison
shape_un
epith_size
clump_thic
The colors are for the selected stump T2 (local examination)
Left Subtree (Benign)
Left Subtree (Malignant)
Right Subtree (Benign)
Right Subtree (Malignant)
Fixed Most Cases
S3
The problematic benign samples moved from the right subtree to the left subtree after adapting the decision threshold (see trajectories as gray lines)

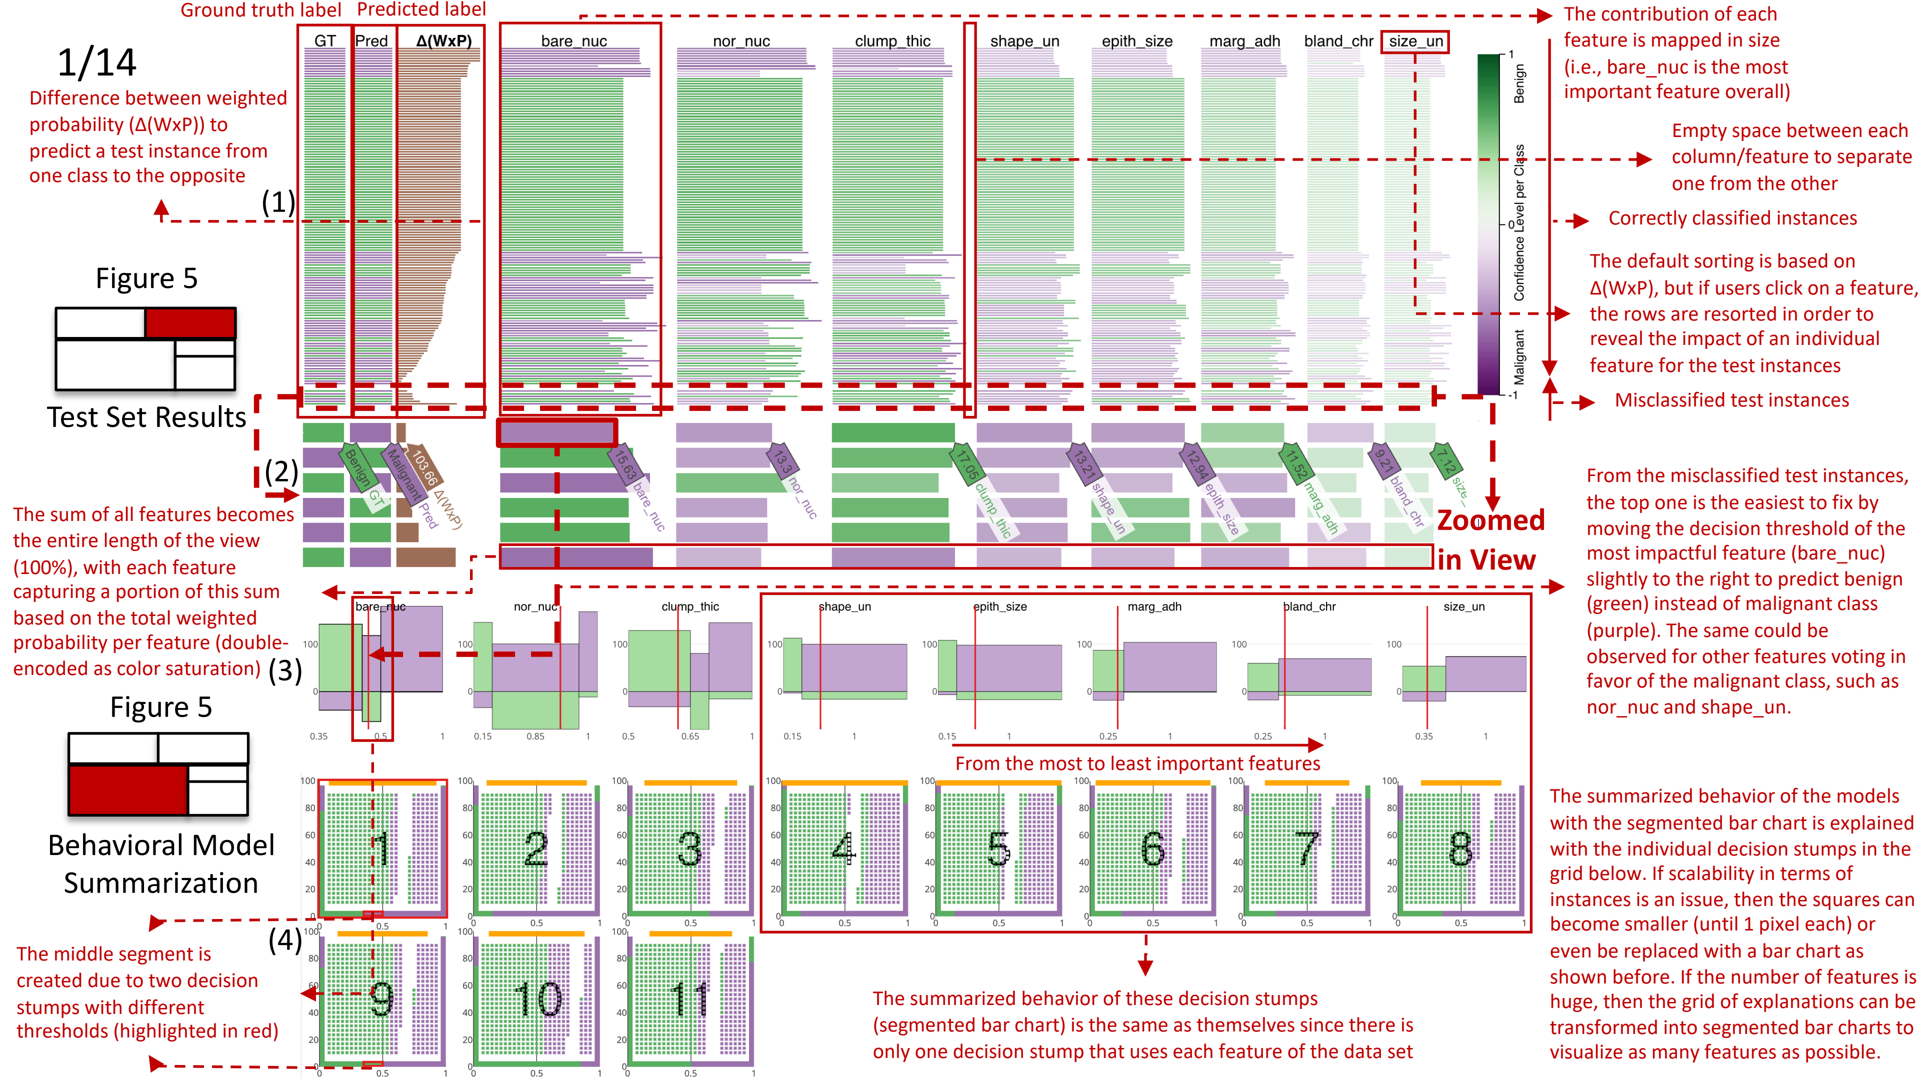
1/14
Figure 5
Test Set Results
Figure 5
Behavioral Model Summarization
Ground truth label
Predicted label
GT
Pred
Δ(WxP)
bare_nuc
nor_nuc
clump_thic
shape_un
epith_size
marg_adh
bland_chr
size_un
Benign
Confidence Level per Class
Malignant
Difference between weighted probability (Δ(WxP)) to predict a test instance from one class to the opposite
(1)
The contribution of each feature is mapped in size (i.e., bare_nuc is the most important feature overall)
Empty space between each column/feature to separate one from the other
Correctly classified instances
The default sorting is based on Δ(WxP), but if users click on a feature, the rows are resorted in order to reveal the impact of an individual feature for the test instances
Misclassified test instances
(2)
Benign GT
Malignant Pred
103.66 Δ(WxP)
15.63 bare_nuc
13.3 nor_nuc
17.05 clump_thic
13.21 shape_un
12.94 epith_size
11.52 marg_adh
9.21 bland_chr
7.12 size_
Zoomed in View
The sum of all features becomes the entire length of the view (100%), with each feature capturing a portion of this sum based on the total weighted probability per feature (double-encoded as color saturation)
(3)
From the misclassified test instances, the top one is the easiest to fix by moving the decision threshold of the most impactful feature (bare_nuc) slightly to the right to predict benign (green) instead of malignant class (purple). The same could be observed for other features voting in favor of the malignant class, such as nor_nuc and shape_un.
From the most to least important features
(4)
The middle segment is created due to two decision stumps with different thresholds (highlighted in red)
The summarized behavior of these decision stumps (segmented bar chart) is the same as themselves since there is only one decision stump that uses each feature of the data set
The summarized behavior of the models with the segmented bar chart is explained with the individual decision stumps in the grid below. If scalability in terms of instances is an issue, then the squares can become smaller (until 1 pixel each) or even be replaced with a bar chart as shown before. If the number of features is huge, then the grid of explanations can be transformed into segmented bar charts to visualize as many features as possible.
1
2
3
4
5
6
7
8
9
10
11

Figure 5

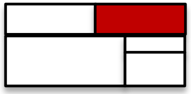

Test Set Results

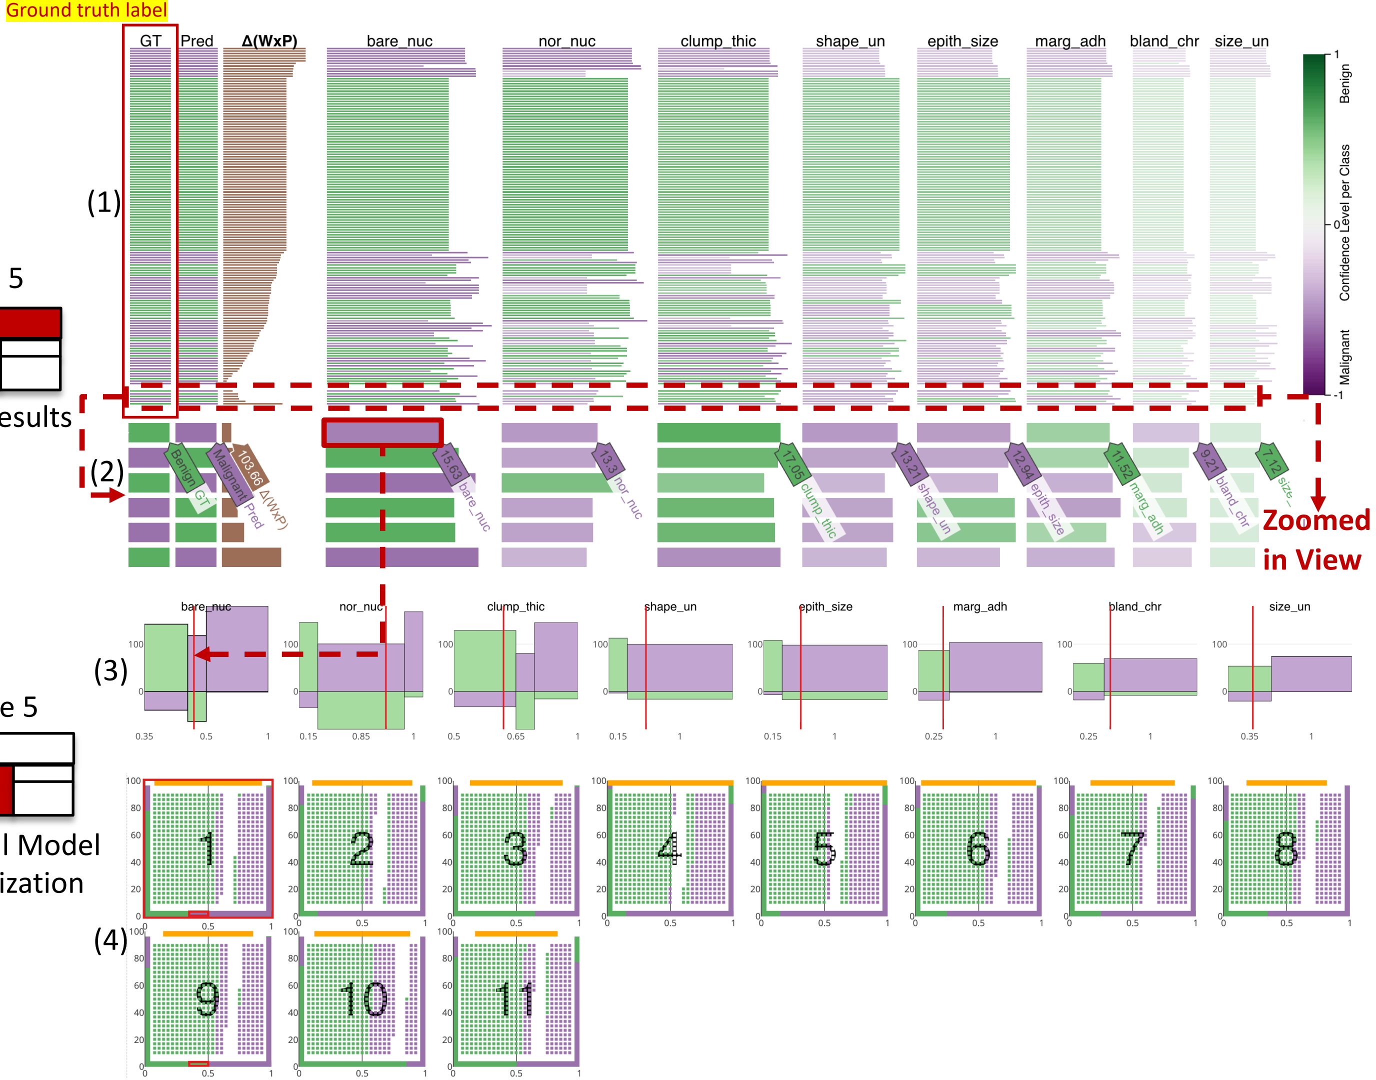


Figure 5

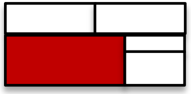

Behavioral Model Summarization

Figure 5

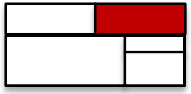

Test Set Results

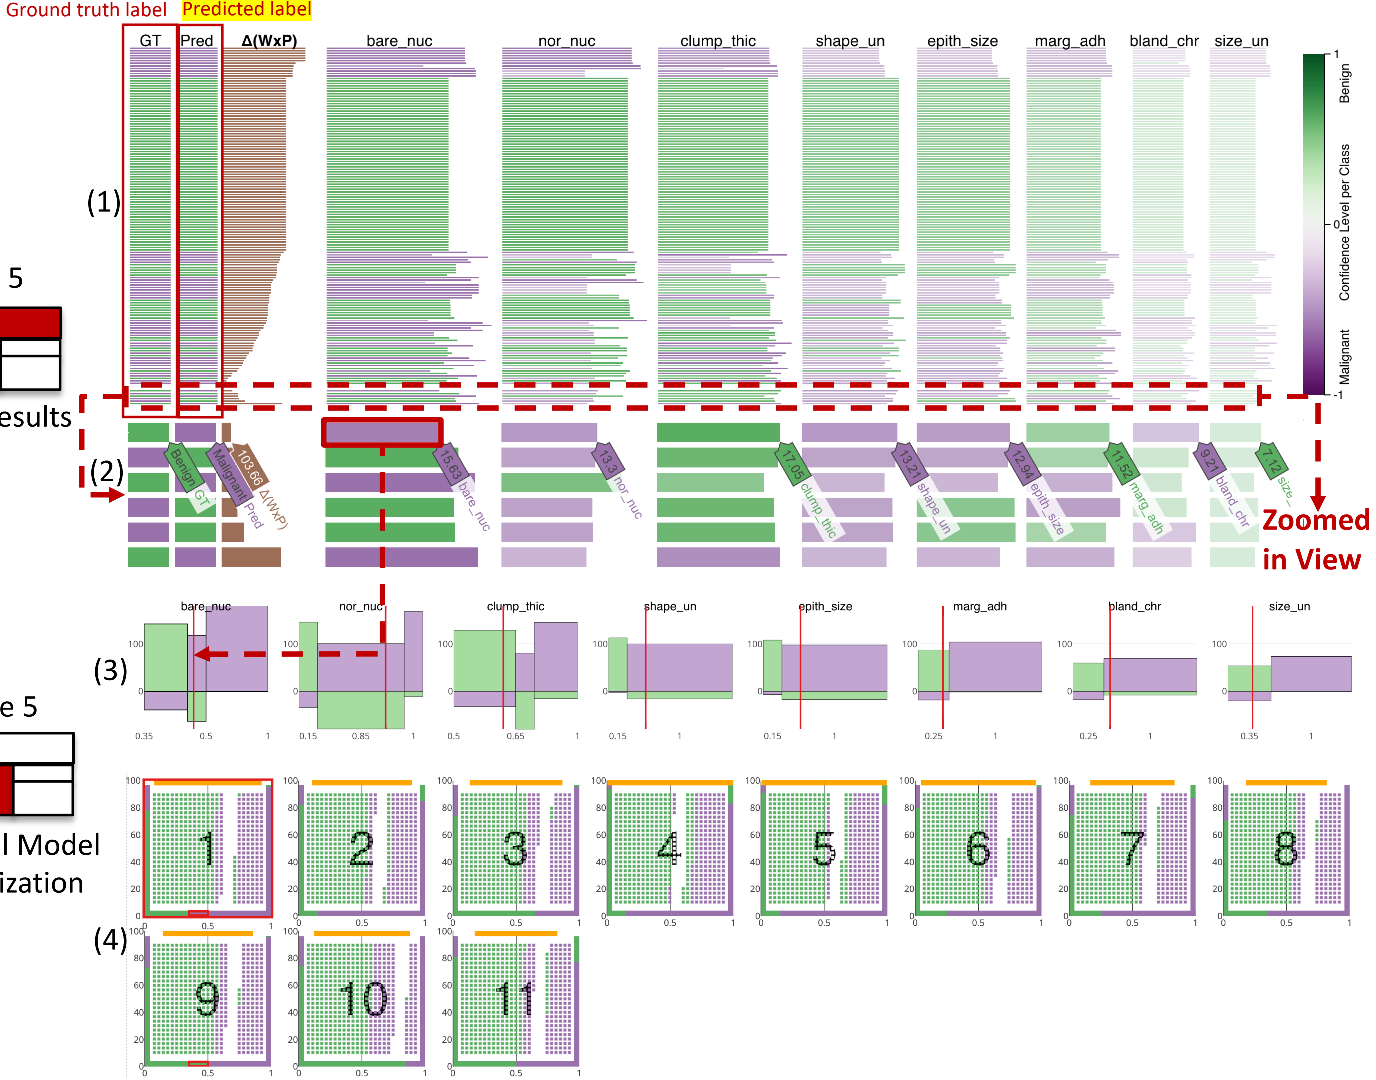


Figure 5

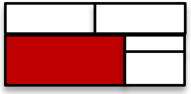

Behavioral Model Summarization

# 4/14

Difference between weighted probability (Δ(WxP)) to predict a test instance from one class to the opposite

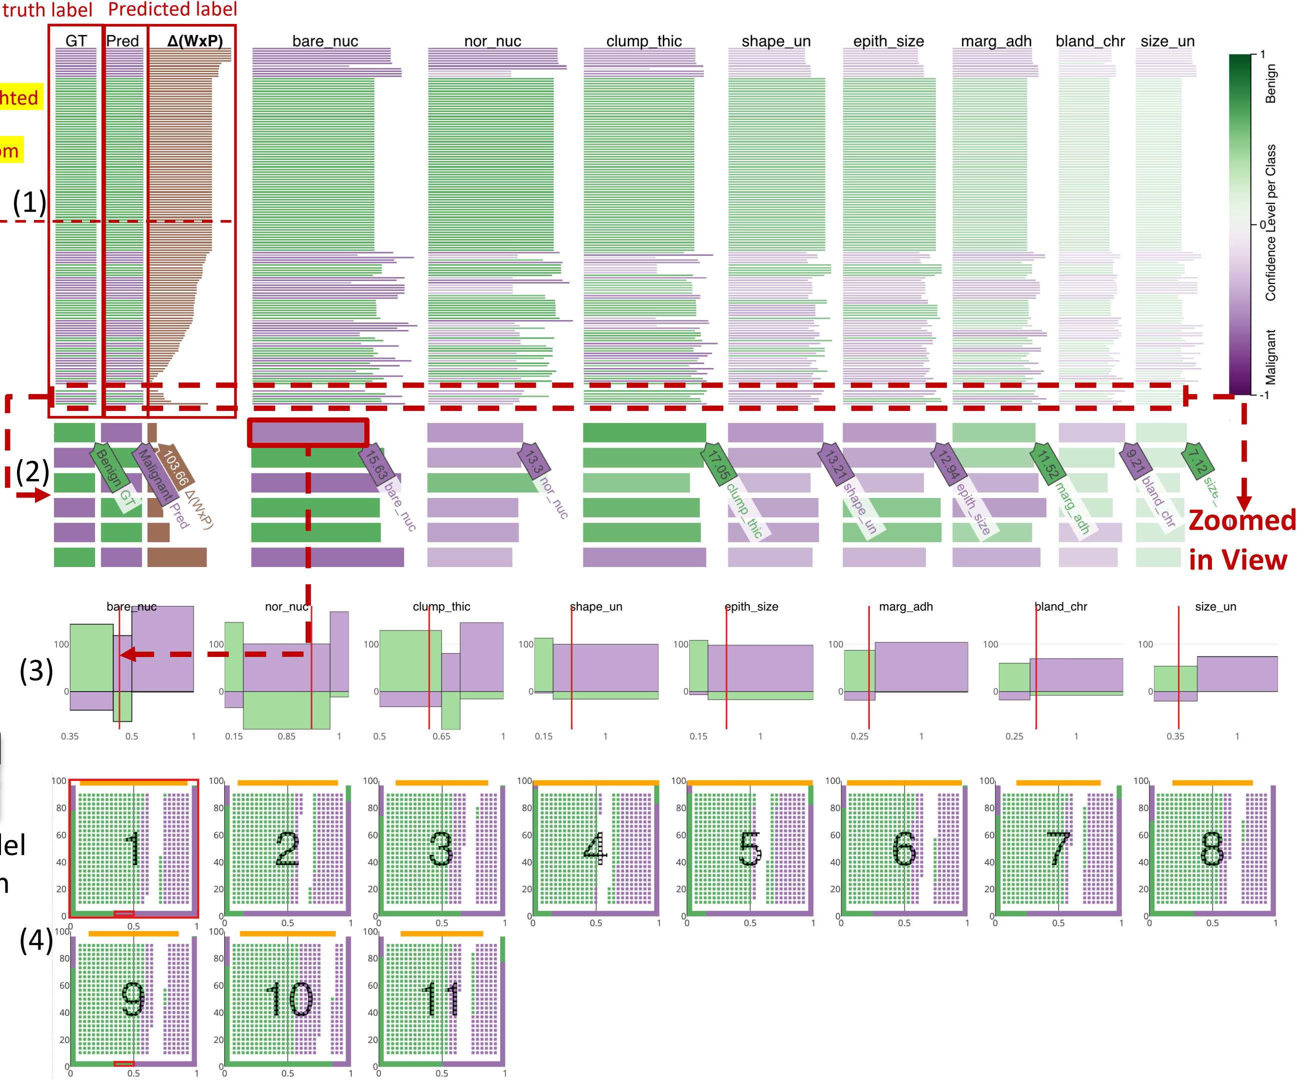


Figure 5

Test Set Results

Figure 5

Behavioral Model Summarization

Difference between weighted probability (Δ(WxP)) to predict a test instance from one class to the opposite

Figure 5

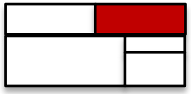

Test Set Results

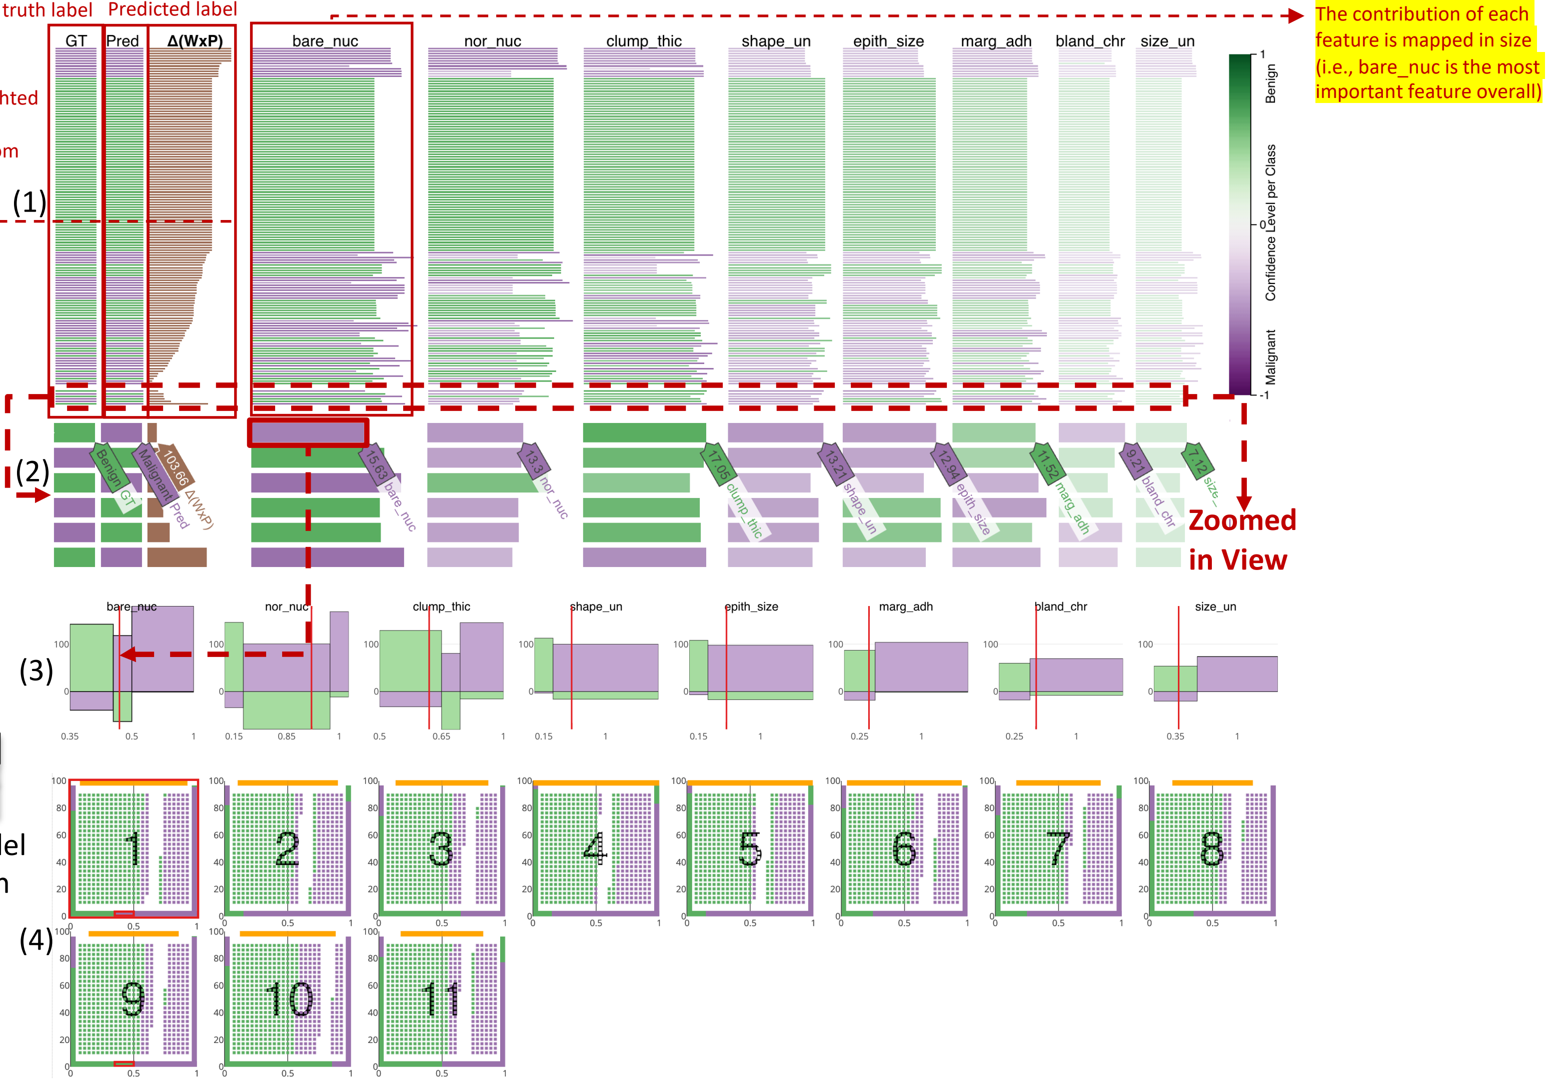



Figure 5

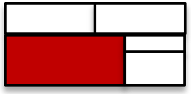

Behavioral Model Summarization

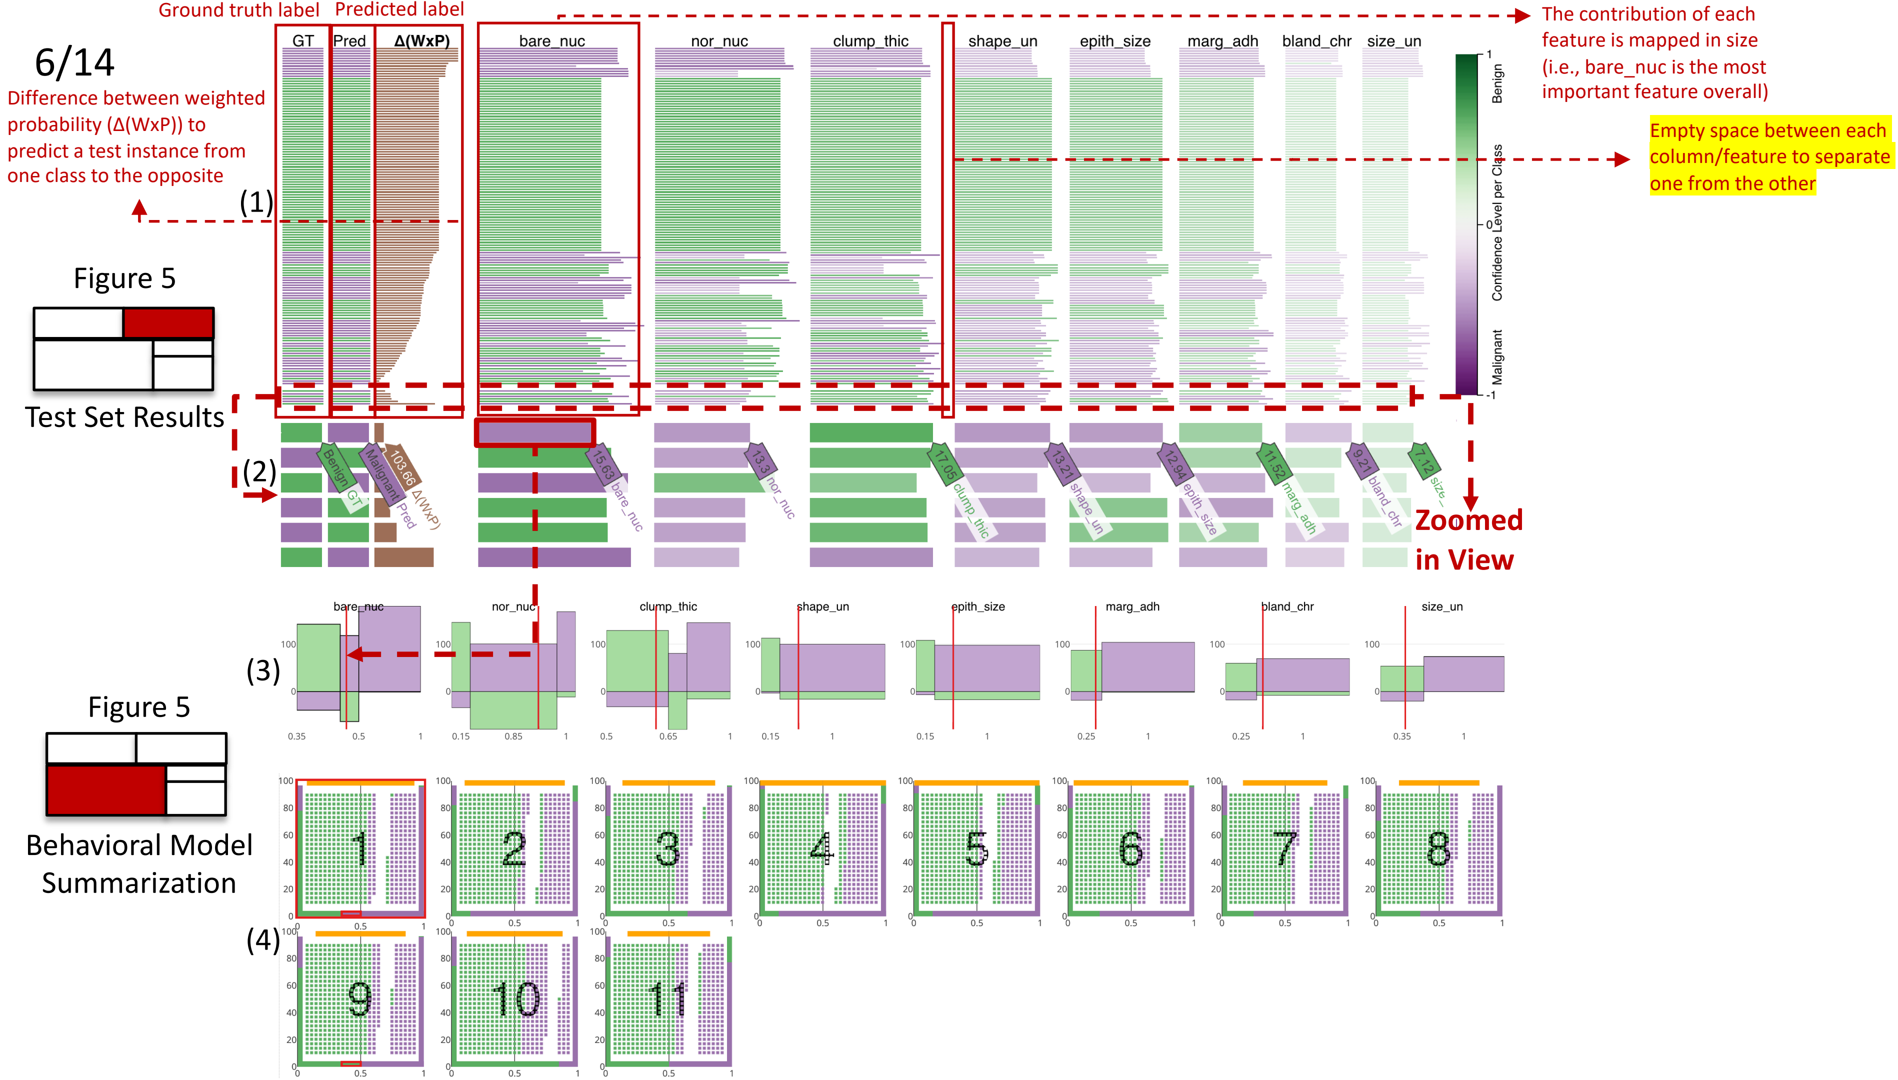
Ground truth label
Predicted label
GT
Pred
Δ(WxP)
bare_nuc
nor_nuc
clump_thic
shape_un
epith_size
marg_adh
bland_chr
size_un
The contribution of each feature is mapped in size (i.e., bare_nuc is the most important feature overall)
Empty space between each column/feature to separate one from the other
Difference between weighted probability (Δ(WxP)) to predict a test instance from one class to the opposite
Benign
Confidence Level per Class
Malignant
(1)
(2)
(3)
(4)
Figure 5
Test Set Results
Benign GT
Malignant Pred
103.66 Δ(WxP)
15.63 bare_nuc
13.3 nor_nuc
17.05 clump_thic
13.21 shape_un
12.94 epith_size
11.52 marg_adh
9.21 bland_chr
7.12 size_
Zoomed in View
Figure 5
Behavioral Model Summarization
1
2
3
4
5
6
7
8
9
10
11

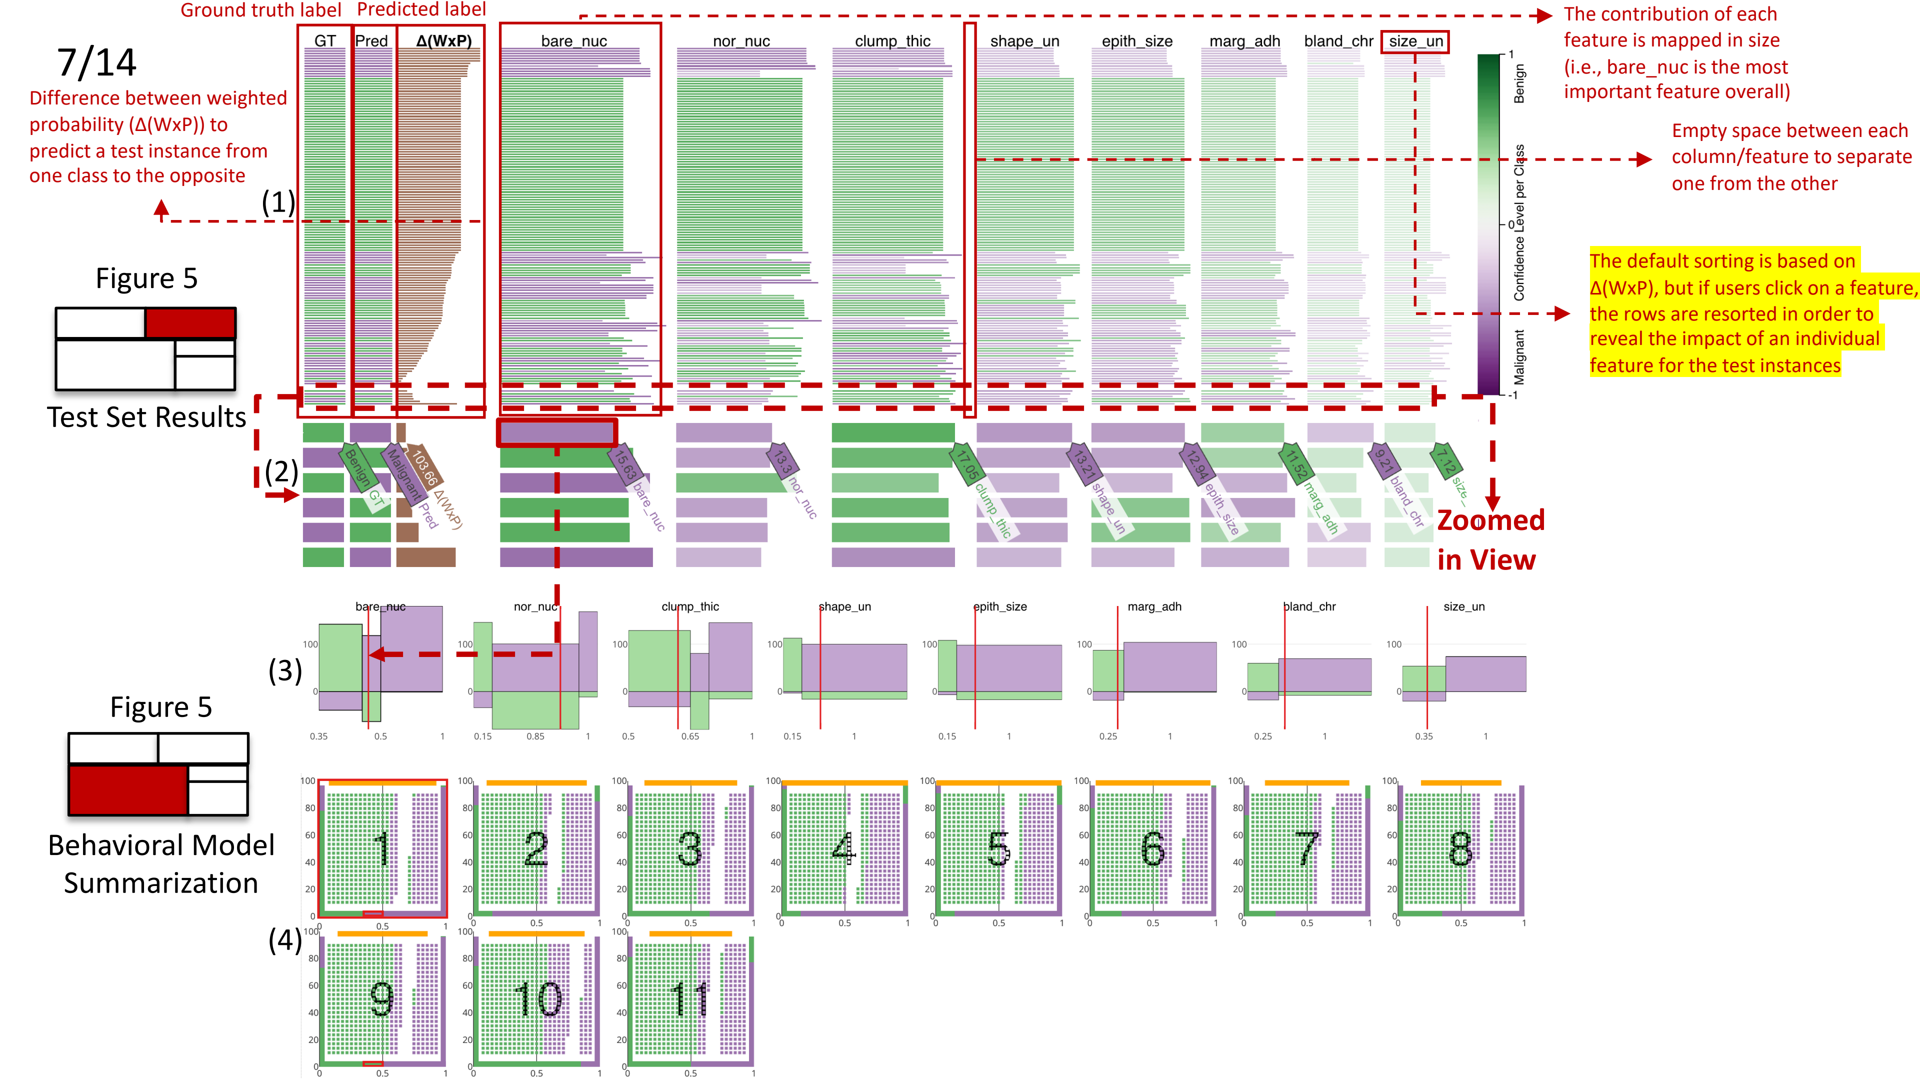
7/14
Ground truth label
Predicted label
Difference between weighted probability (Δ(WxP)) to predict a test instance from one class to the opposite
The contribution of each feature is mapped in size (i.e., bare_nuc is the most important feature overall)
Empty space between each column/feature to separate one from the other
The default sorting is based on Δ(WxP), but if users click on a feature, the rows are resorted in order to reveal the impact of an individual feature for the test instances
Figure 5
Test Set Results
Figure 5
Behavioral Model Summarization
(1)
(2)
(3)
(4)
GT
Pred
Δ(WxP)
bare_nuc
nor_nuc
clump_thic
shape_un
epith_size
marg_adh
bland_chr
size_un
Benign
Confidence Level per Class
Malignant
Zoomed in View
Benign GT
Malignant Pred
103.66 Δ(WxP)
15.63 bare_nuc
13.3 nor_nuc
17.05 clump_thic
13.21 shape_un
12.94 epith_size
11.52 marg_adh
9.21 bland_chr
7.12 size_

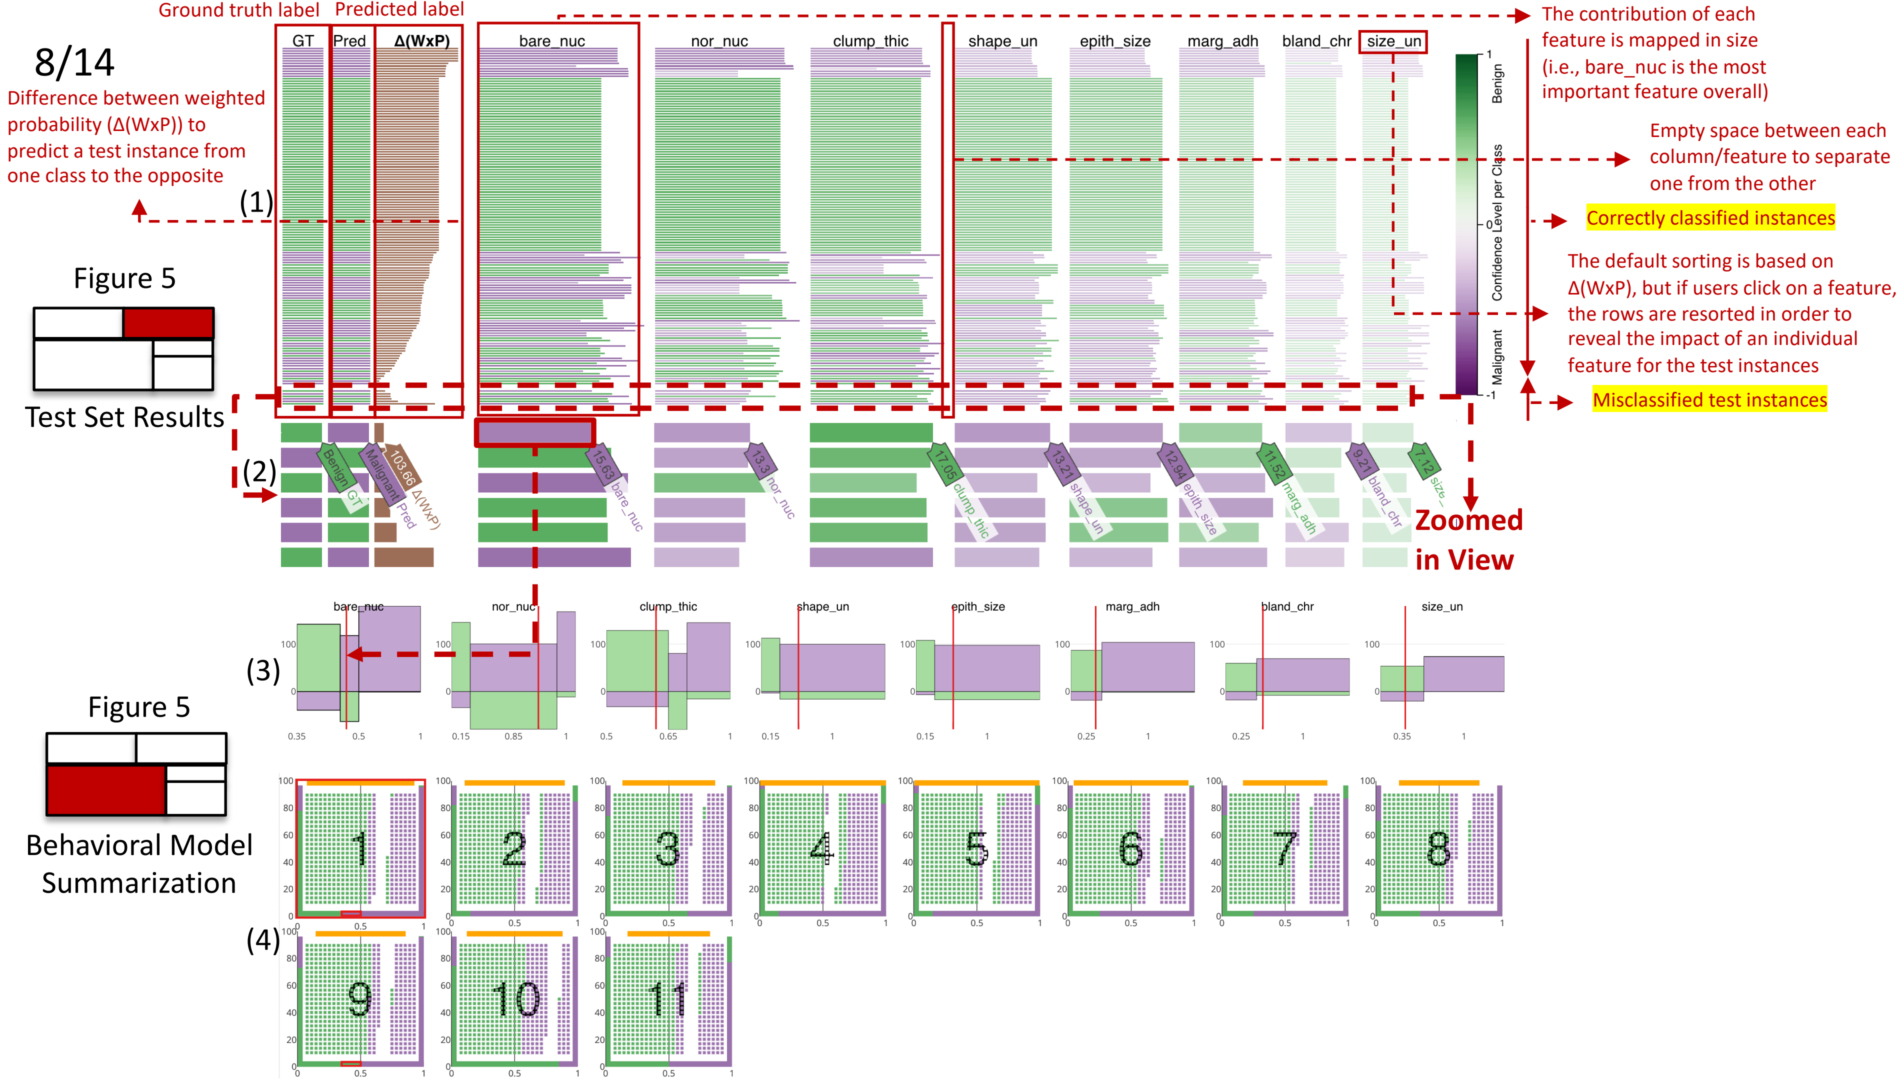
Ground truth label
Predicted label
The contribution of each feature is mapped in size (i.e., bare_nuc is the most important feature overall)
Difference between weighted probability (Δ(WxP)) to predict a test instance from one class to the opposite
Empty space between each column/feature to separate one from the other
Correctly classified instances
The default sorting is based on Δ(WxP), but if users click on a feature, the rows are resorted in order to reveal the impact of an individual feature for the test instances
Misclassified test instances
Figure 5
Test Set Results
(1)
(2)
(3)
(4)
GT
Pred
Δ(WxP)
bare_nuc
nor_nuc
clump_thic
shape_un
epith_size
marg_adh
bland_chr
size_un
Benign
Malignant
Confidence Level per Class
Zoomed in View
Figure 5
Behavioral Model Summarization

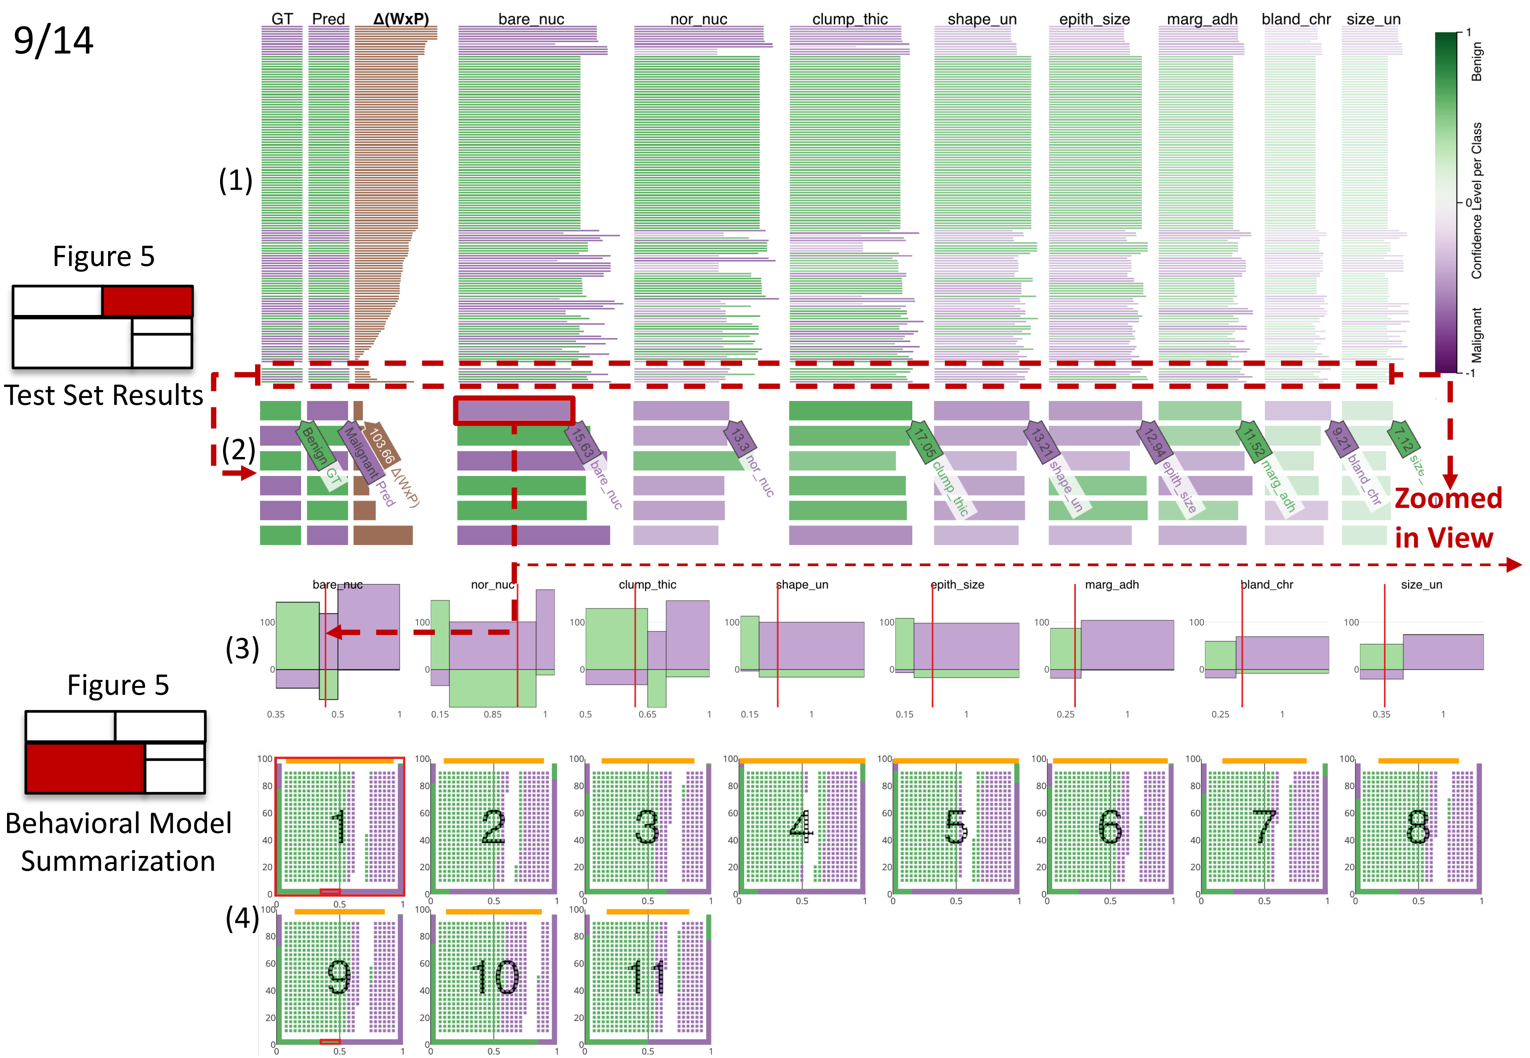


From the misclassified test instances, the top one is the easiest to fix by moving the decision threshold of the most impactful feature (bare_nuc) slightly to the right to predict benign (green) instead of malignant class (purple). The same could be observed for other features voting in favor of the malignant class, such as nor_nuc and shape_un.

Figure 5

Test Set Results

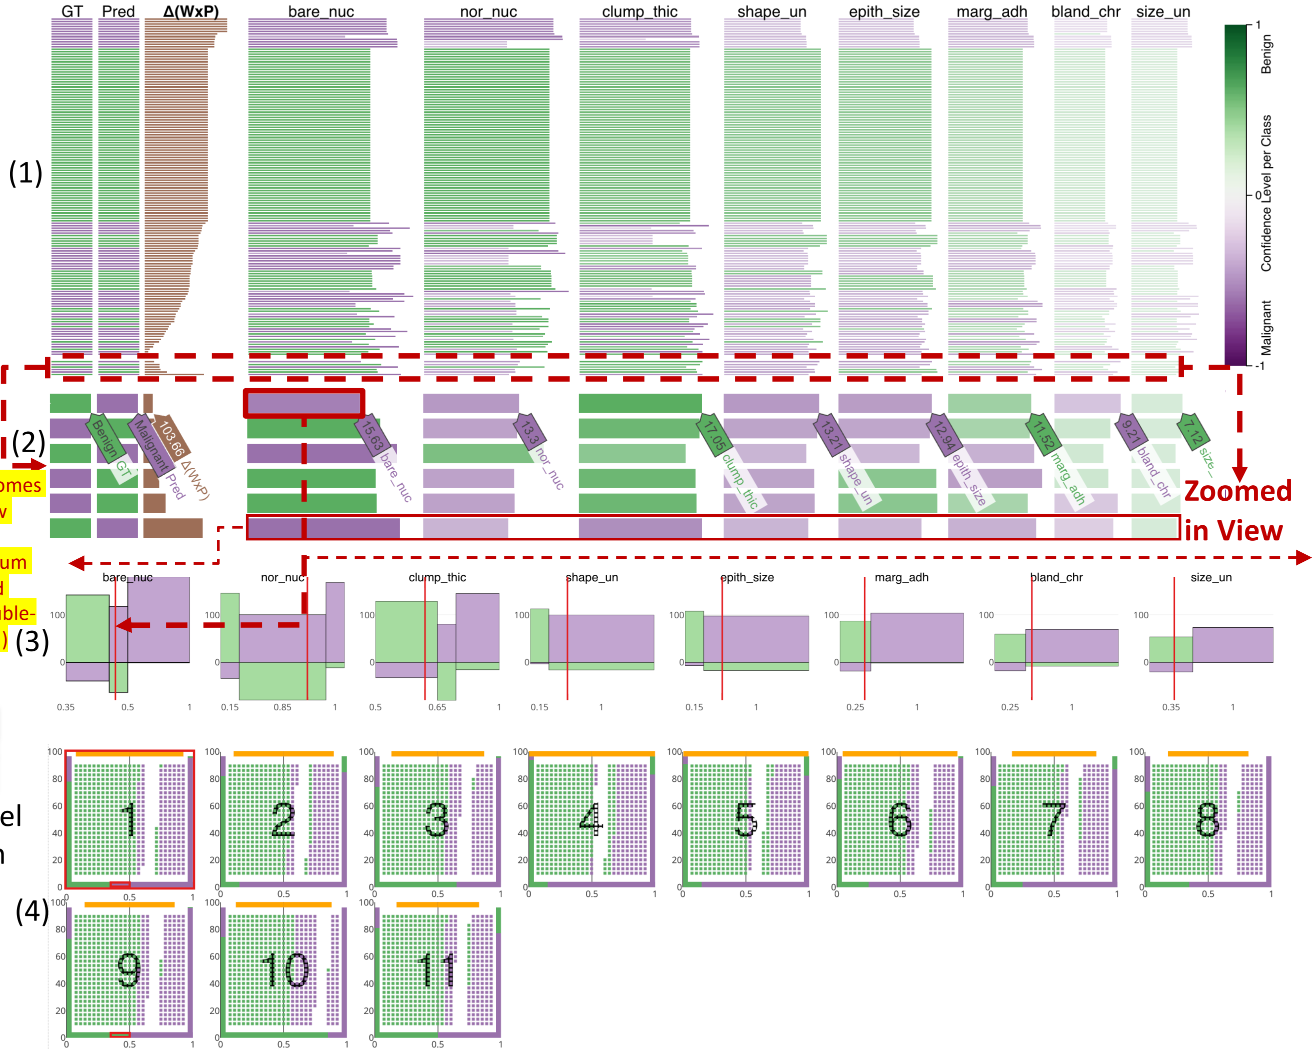


The sum of all features becomes the entire length of the view (100%), with each feature capturing a portion of this sum based on the total weighted probability per feature (double-encoded as color saturation)

Figure 5

Behavioral Model Summarization

From the misclassified test instances, the top one is the easiest to fix by moving the decision threshold of the most impactful feature (bare_nuc) slightly to the right to predict benign (green) instead of malignant class (purple). The same could be observed for other features voting in favor of the malignant class, such as nor_nuc and shape_un.

Figure 5

Test Set Results

Figure 5

Behavioral Model Summarization

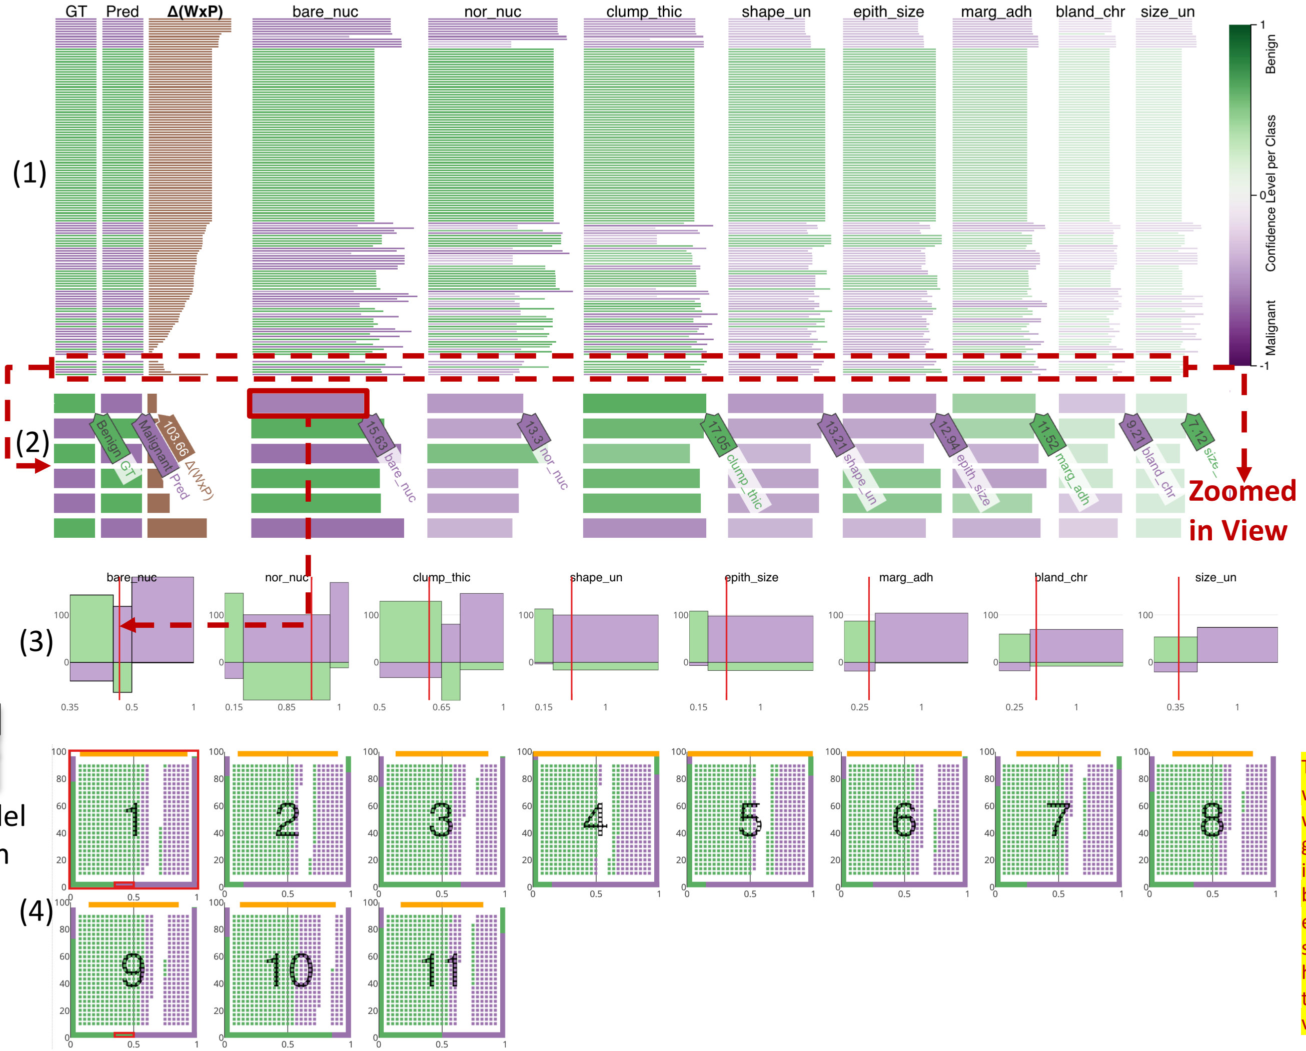


The summarized behavior of the models with the segmented bar chart is explained with the individual decision stumps in the grid below. If scalability in terms of instances is an issue, then the squares can become smaller (until 1 pixel each) or even be replaced with a bar chart as shown before. If the number of features is huge, then the grid of explanations can be transformed into segmented bar charts to visualize as many features as possible.

Figure 5

Test Set Results

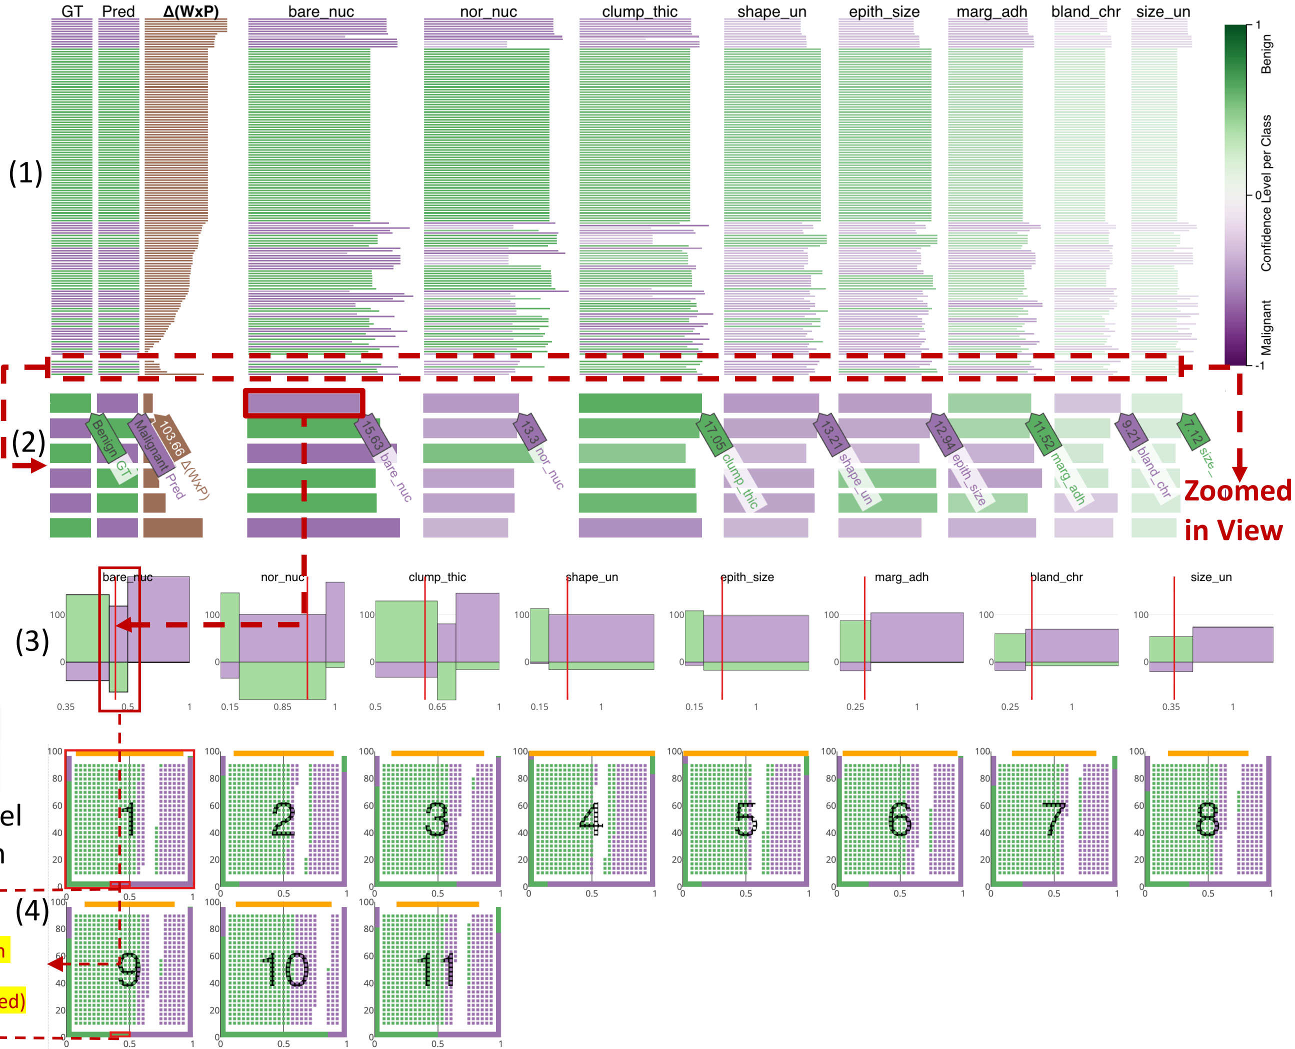


Figure 5

Behavioral Model Summarization

The middle segment is created due to two decision stumps with different thresholds (highlighted in red)

The summarized behavior of the models with the segmented bar chart is explained with the individual decision stumps in the grid below. If scalability in terms of instances is an issue, then the squares can become smaller (until 1 pixel each) or even be replaced with a bar chart as shown before. If the number of features is huge, then the grid of explanations can be transformed into segmented bar charts to visualize as many features as possible.

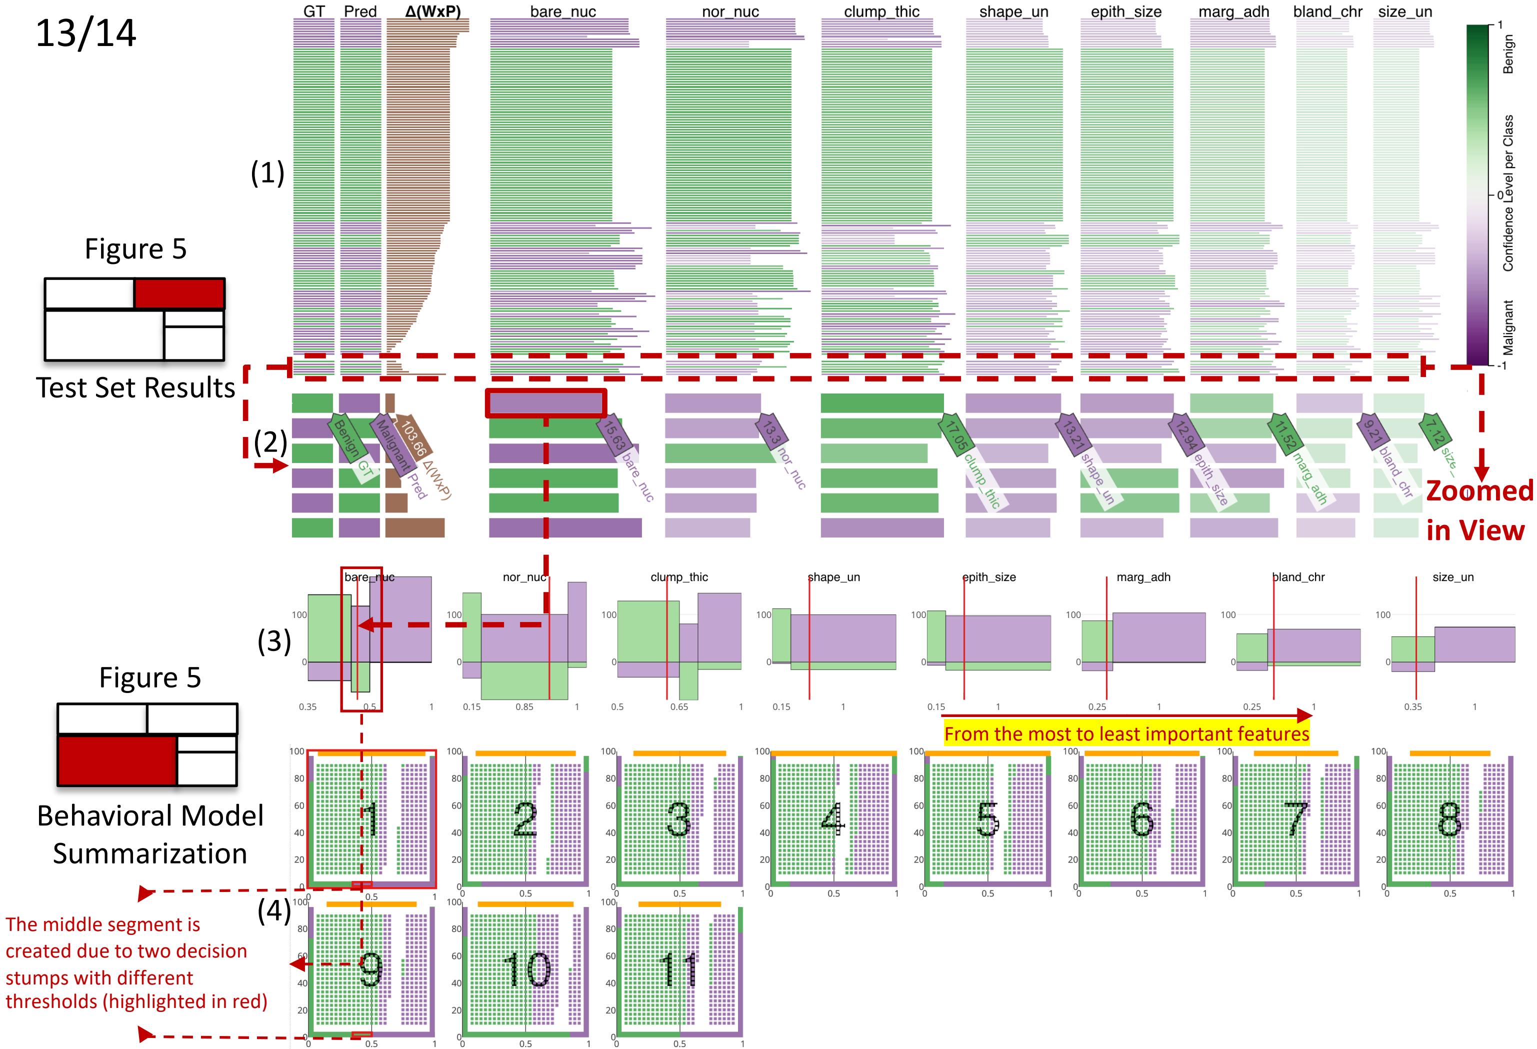


The summarized behavior of the models with the segmented bar chart is explained with the individual decision stumps in the grid below. If scalability in terms of instances is an issue, then the squares can become smaller (until 1 pixel each) or even be replaced with a bar chart as shown before. If the number of features is huge, then the grid of explanations can be transformed into segmented bar charts to visualize as many features as possible.

Figure 5

Test Set Results

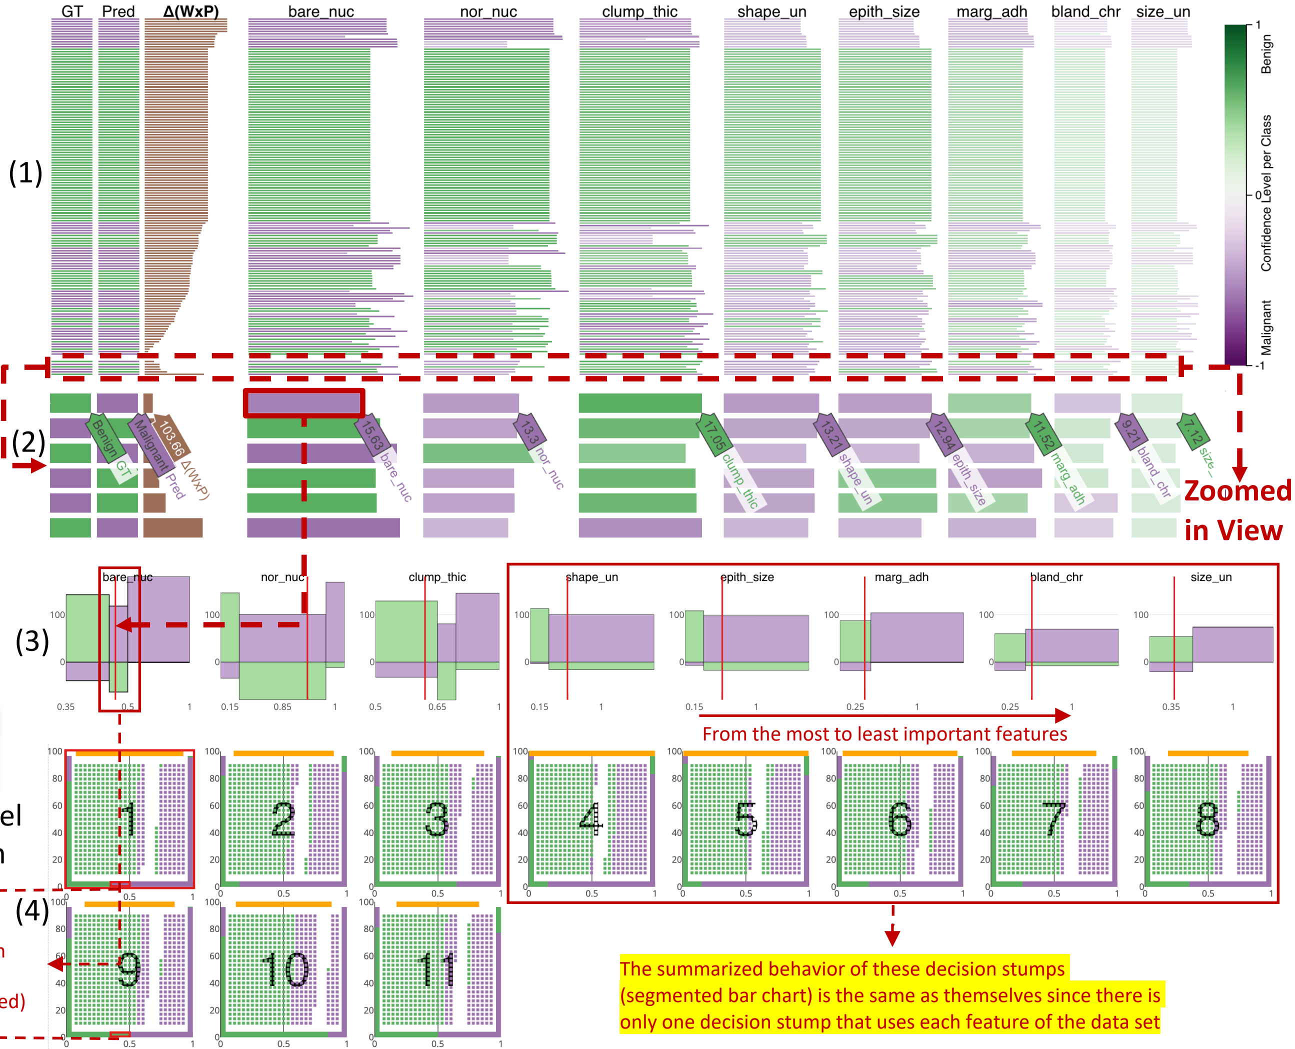


Figure 5

Behavioral Model Summarization

The middle segment is created due to two decision stumps with different thresholds (highlighted in red)

The summarized behavior of the models with the segmented bar chart is explained with the individual decision stumps in the grid below. If scalability in terms of instances is an issue, then the squares can become smaller (until 1 pixel each) or even be replaced with a bar chart as shown before. If the number of features is huge, then the grid of explanations can be transformed into segmented bar charts to visualize as many features as possible.

# Section 6.2: Usage scenario

1/12

**#7-#11**: These five surrogate models are more accurate (see fidelity score) when using fewer decimal digits (2 instead of 4)

**#6**: The first surrogate model with above 90% but relatively low complexity. 5 out of 8 decision stumps have a high weighted probability

**#41**: The decision threshold is at approx. 0.55, with the left subtree doing better than the right subtree due to fewer mixed instances (left bar chart)

**#41**: Insulin is the only feature that contributes to the negative class, then suddenly changes to positive (in purple), and finally continues to vote for negative. That is unusual and requires further investigation

**#41**: This decision stump is the most influential in terms of weight but is divided at about 50% between the two classes. When summing up all decision stumps, this stump is like being ruled out

**#6**: Sorting based on Glucose shows that the prediction of this surrogate model is mostly done based on this feature

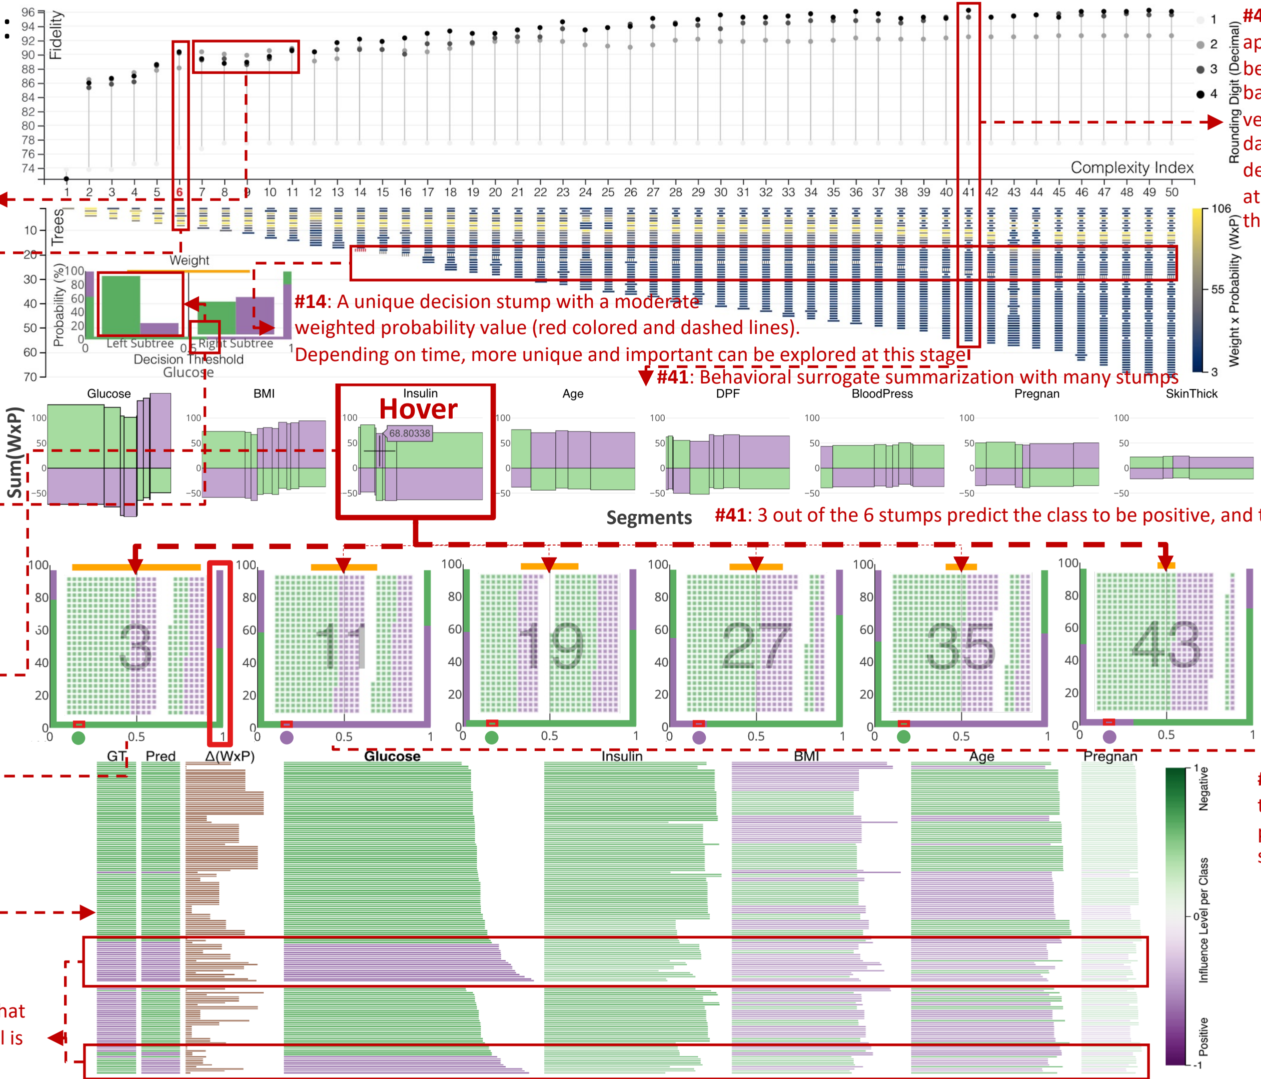


**#14**: A unique decision stump with a moderate weighted probability value (red colored and dashed lines). Depending on time, more unique and important can be explored at this stage

**#41**: Behavioral surrogate summarization with many stumps

**#41**: 3 out of the 6 stumps predict the class to be positive, and the other three negative

**#41**: The default surrogate model with approx. 96% fidelity, with its behavior being summarized in the segmented bar chart. Most decision stumps are very weak (low weighted probability in dark blue), but help smoothen the decision boundaries (check this effect at the multiple decision thresholds of the segmented bar chart)

**#41**: This decision stump becomes the most impactful in favor of the positive class, which is why this strange behavior occurred

(1) Figure 1

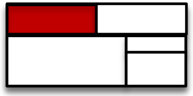

Surrogate Model Selection

(2) Figure 6

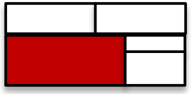

Behavioral Model Summarization

(3) Figure 1

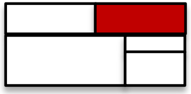

Test Set Results

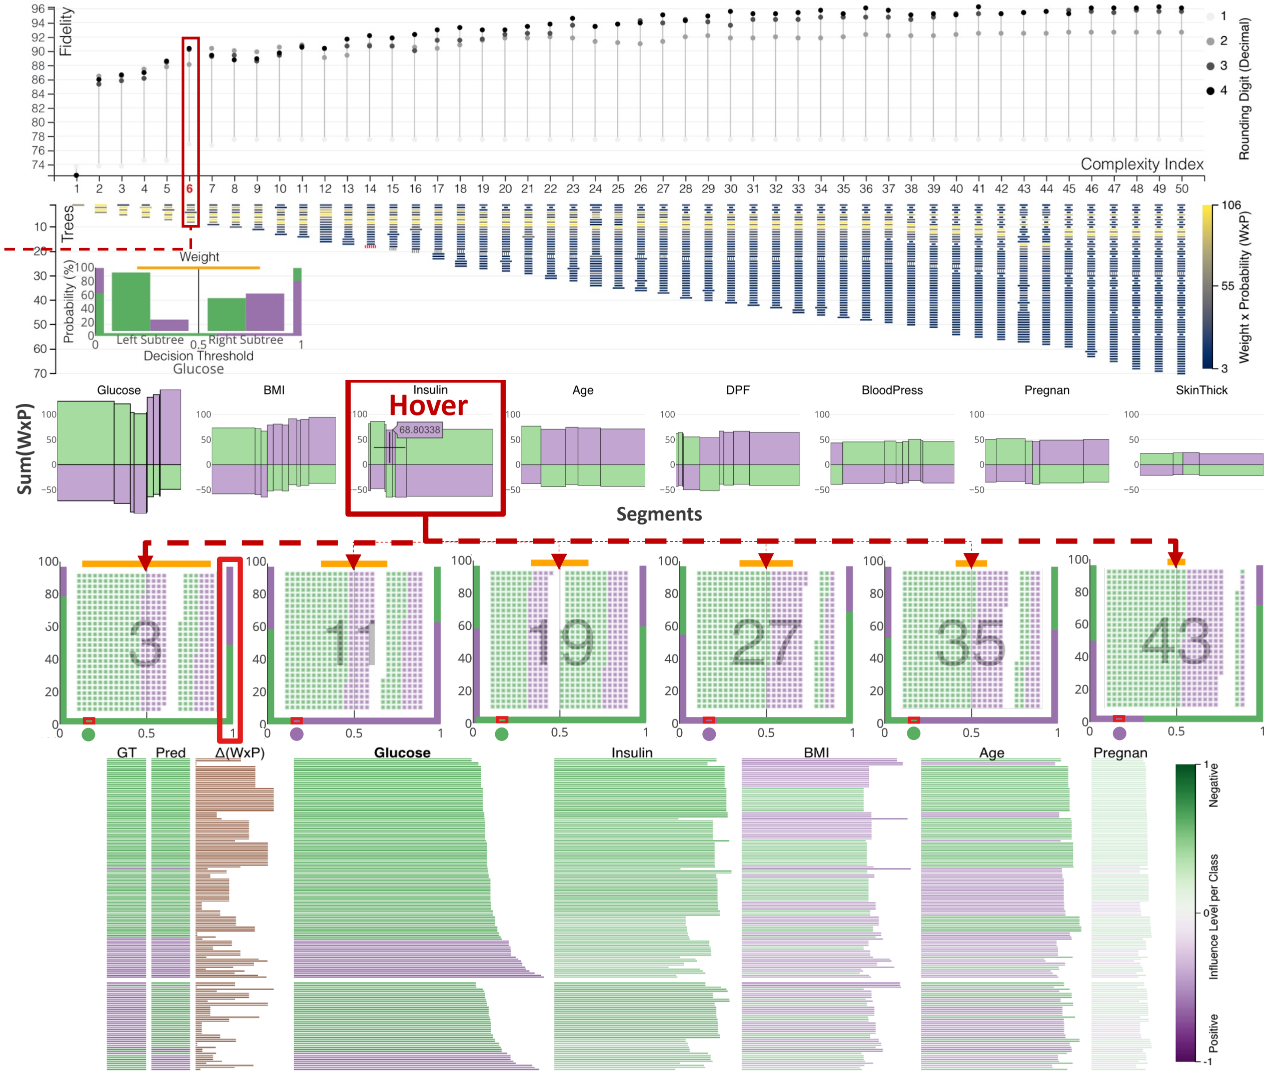


**#6**: The first surrogate model with above 90% but relatively low complexity. 5 out of 8 decision stumps have a high weighted probability

(1)

Figure 1

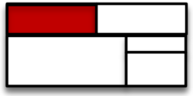

Surrogate Model Selection

(2)

Figure 6

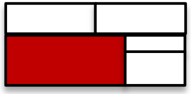

Behavioral Model Summarization

(3)

Figure 1

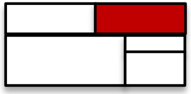

Test Set Results

**#7-#11**: These five surrogate models are more accurate (see fidelity score) when using fewer decimal digits (2 instead of 4)

**#6**: The first surrogate model with above 90% but relatively low complexity. 5 out of 8 decision stumps have a high weighted probability

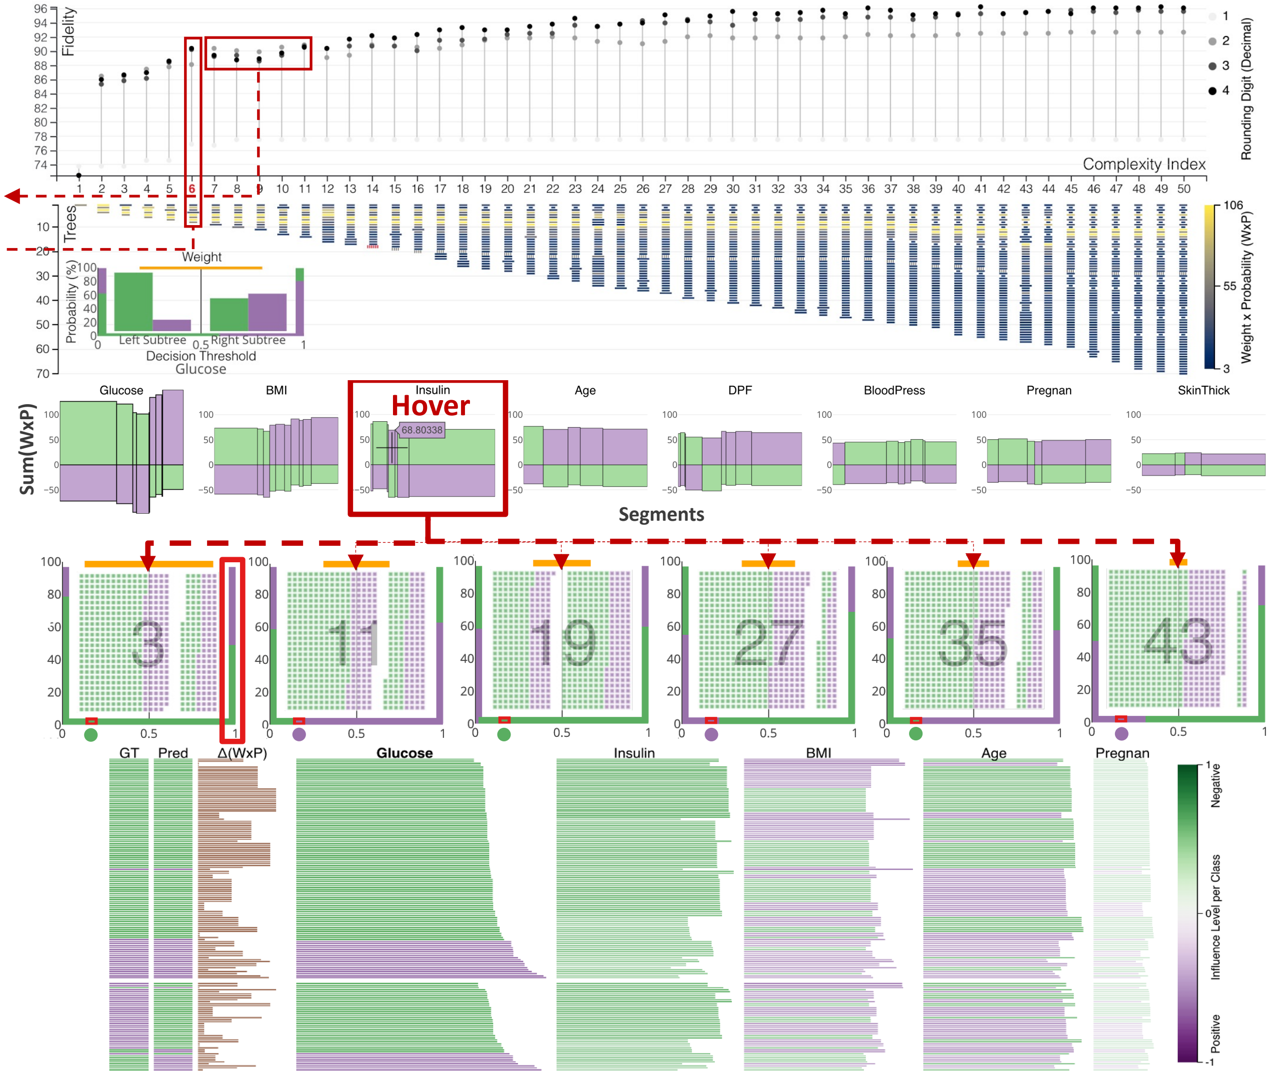


(1) Figure 1 Surrogate Model Selection

(2) Figure 6 Behavioral Model Summarization

(3) Figure 1 Test Set Results

**#7-#11**: These five surrogate models are more accurate (see fidelity score) when using fewer decimal digits (2 instead of 4)

**#6**: The first surrogate model with above 90% but relatively low complexity. 5 out of 8 decision stumps have a high weighted probability

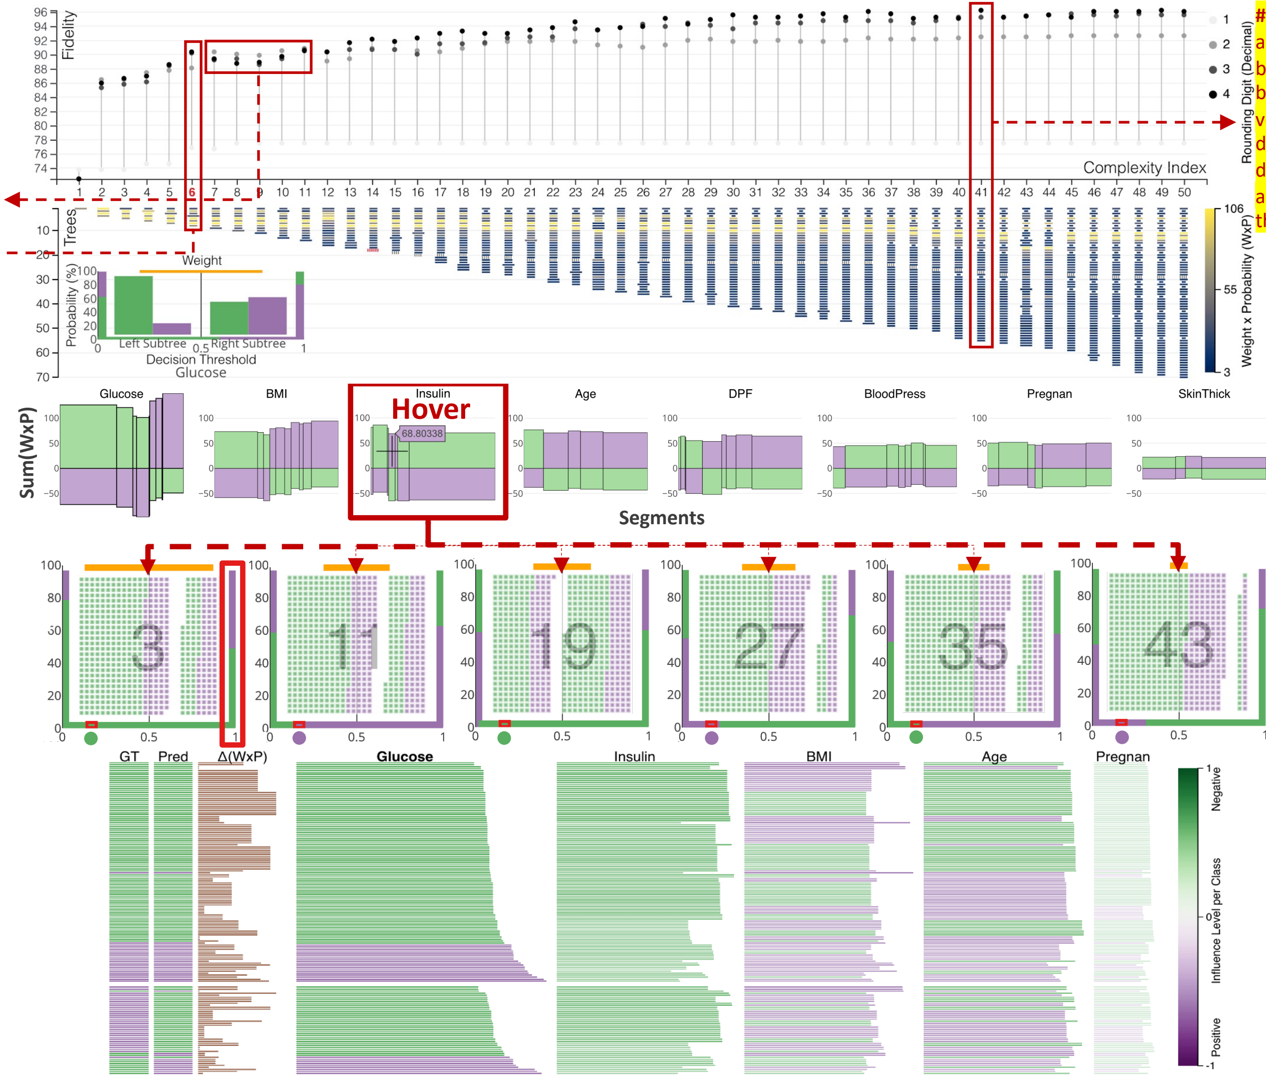


**#41**: The default surrogate model with approx. 96% fidelity, with its behavior being summarized in the segmented bar chart. Most decision stumps are very weak (low weighted probability in dark blue), but help smoothen the decision boundaries (check this effect at the multiple decision thresholds of the segmented bar chart)

(1) Figure 1

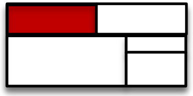

Surrogate Model Selection

(2) Figure 6

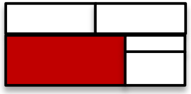

Behavioral Model Summarization

(3) Figure 1

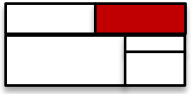

Test Set Results

**#7-#11**: These five surrogate models are more accurate (see fidelity score) when using fewer decimal digits (2 instead of 4)

**#6**: The first surrogate model with above 90% but relatively low complexity. 5 out of 8 decision stumps have a high weighted probability

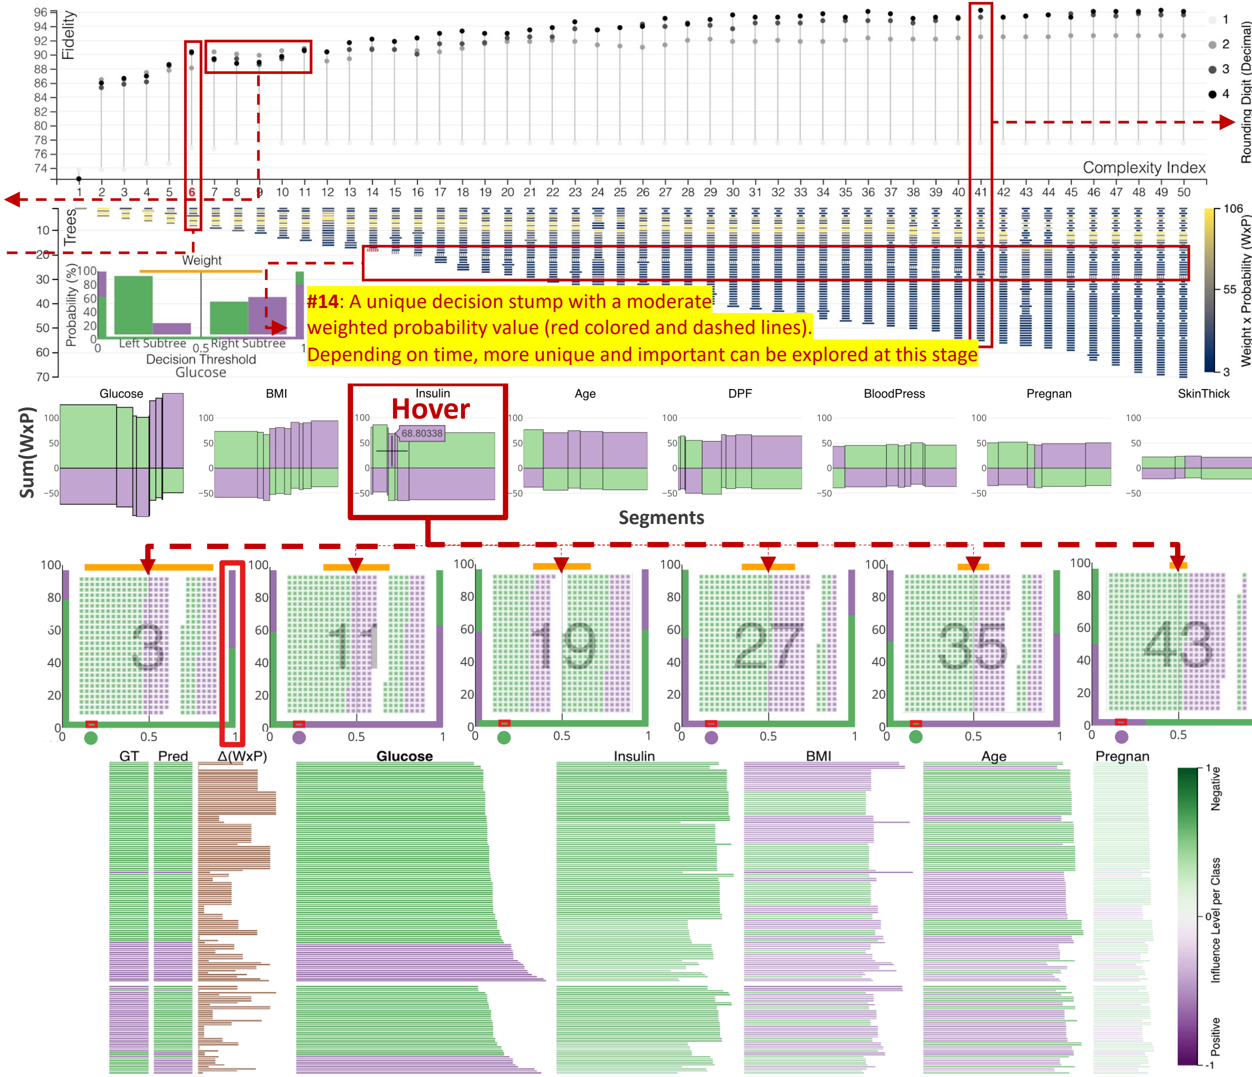


**#41**: The default surrogate model with approx. 96% fidelity, with its behavior being summarized in the segmented bar chart. Most decision stumps are very weak (low weighted probability in dark blue), but help smoothen the decision boundaries (check this effect at the multiple decision thresholds of the segmented bar chart)

(1) Figure 1

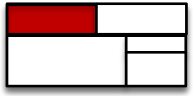

Surrogate Model Selection

(2) Figure 6

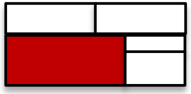

Behavioral Model Summarization

(3) Figure 1

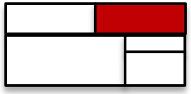

Test Set Results

**#7-#11**: These five surrogate models are more accurate (see fidelity score) when using fewer decimal digits (2 instead of 4)

**#6**: The first surrogate model with above 90% but relatively low complexity. 5 out of 8 decision stumps have a high weighted probability

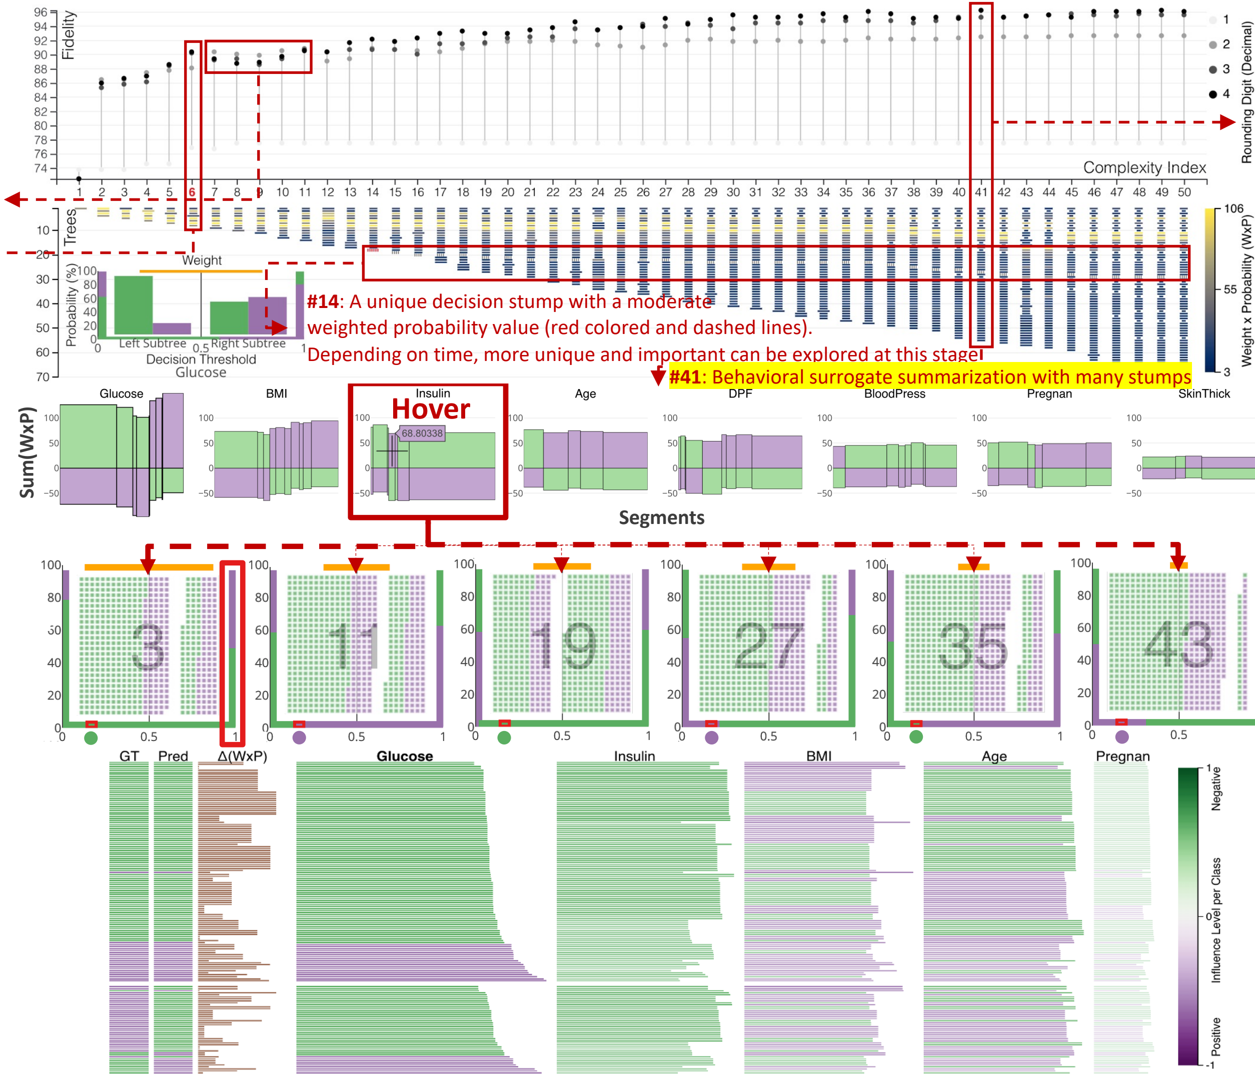


**#41**: The default surrogate model with approx. 96% fidelity, with its behavior being summarized in the segmented bar chart. Most decision stumps are very weak (low weighted probability in dark blue), but help smoothen the decision boundaries (check this effect at the multiple decision thresholds of the segmented bar chart)

(1)

Figure 1

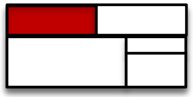

Surrogate Model Selection

(2)

Figure 6

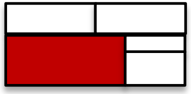

Behavioral Model Summarization

(3)

Figure 1

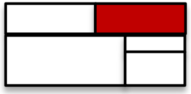

Test Set Results

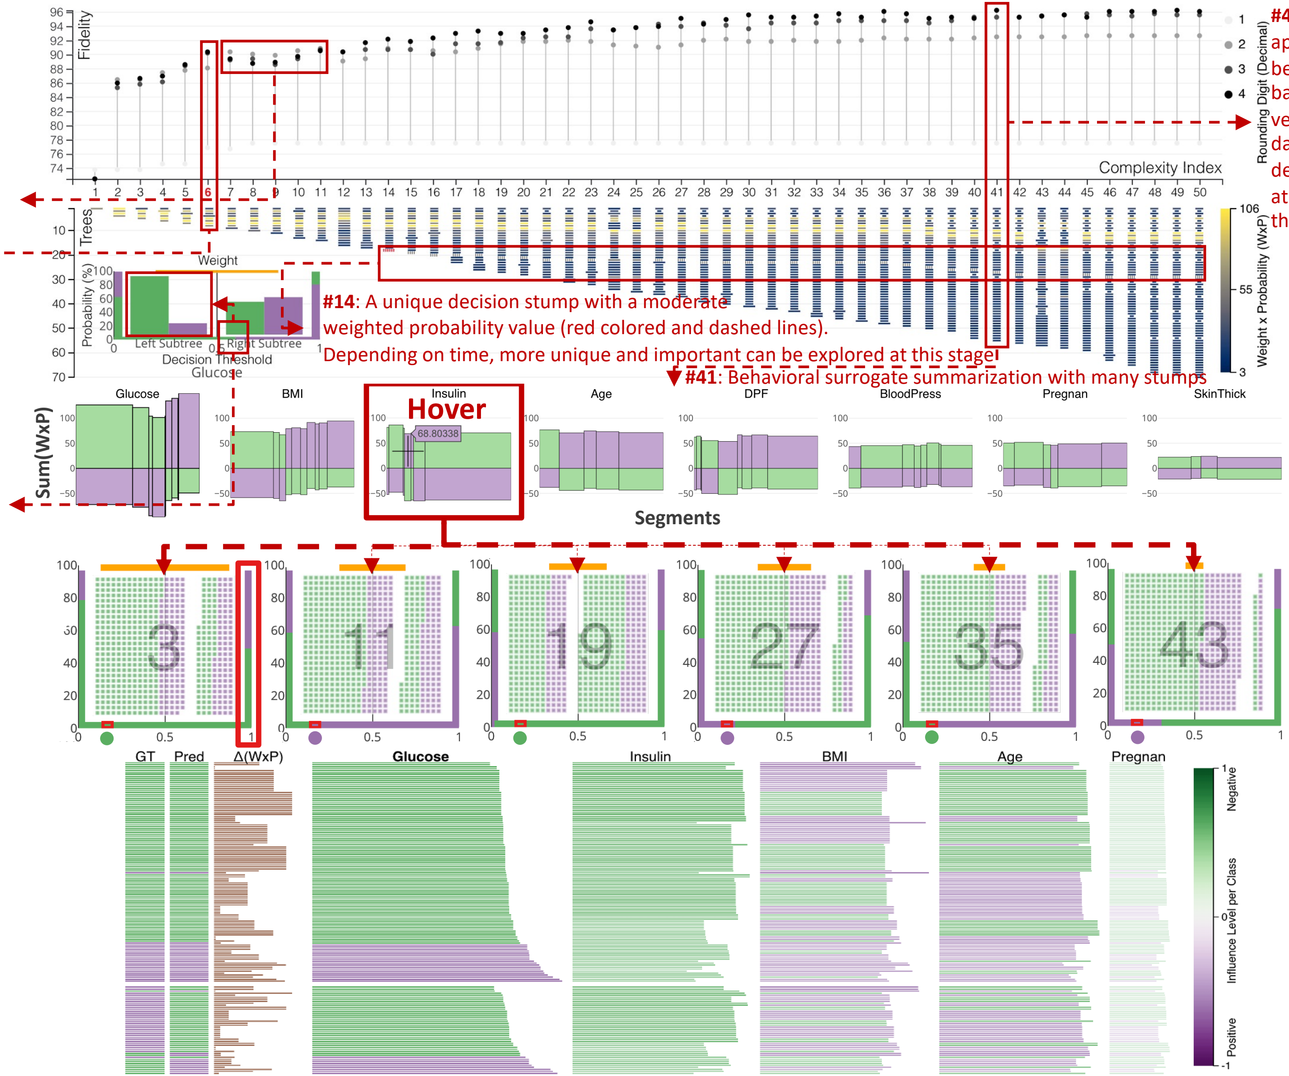


(1)

Figure 1

Surrogate Model Selection

(2)

Figure 6

Behavioral Model Summarization

(3)

Figure 1

Test Set Results

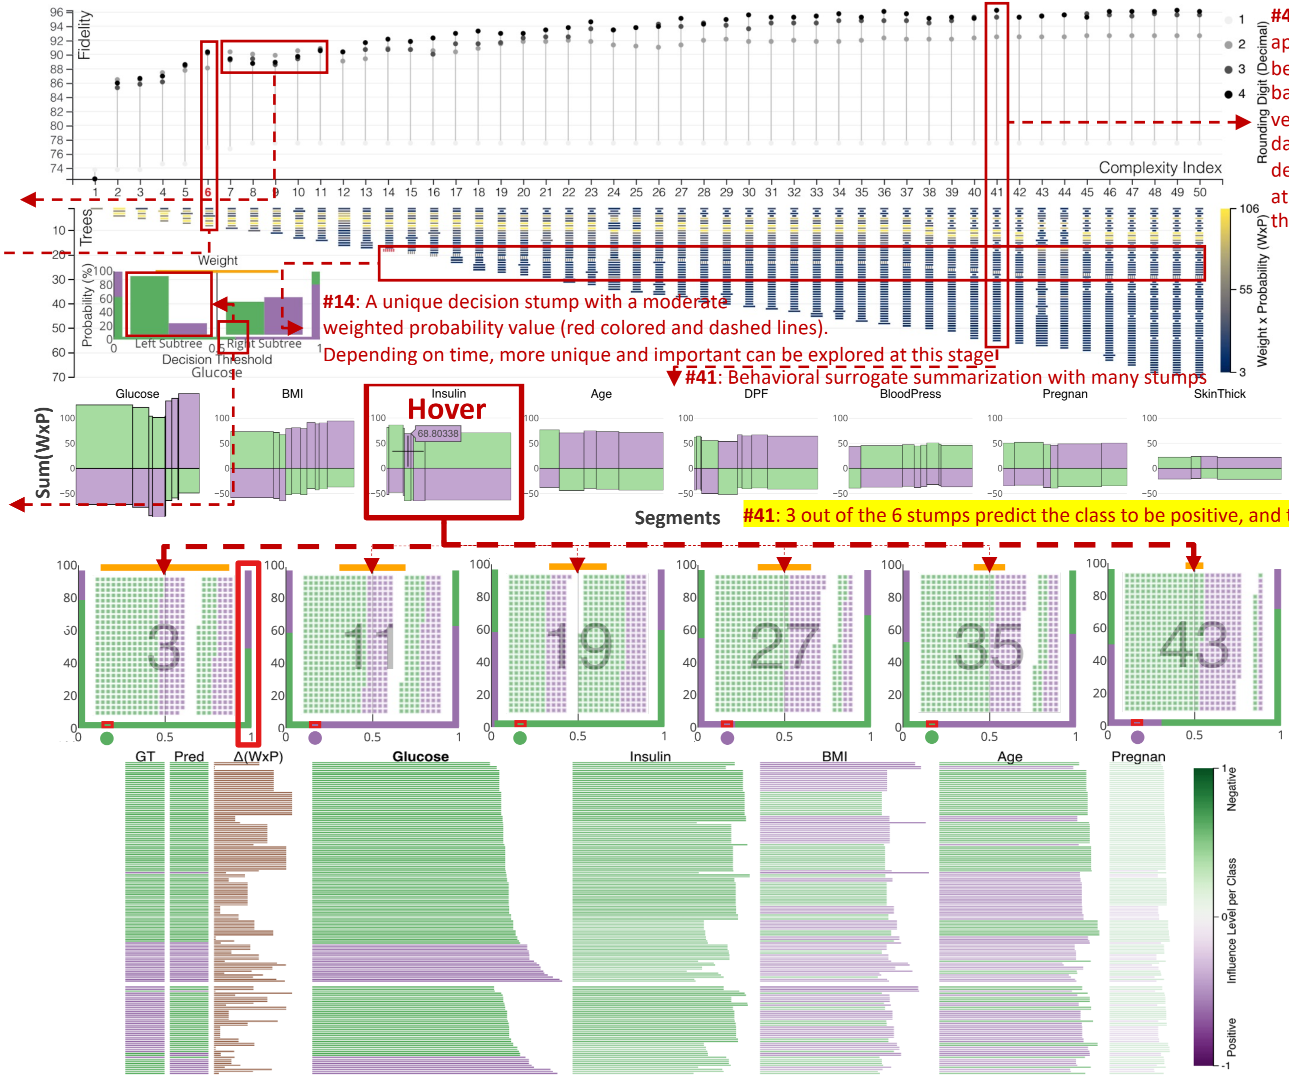


**#7-#11**: These five surrogate models are more accurate (see fidelity score) when using fewer decimal digits (2 instead of 4)

**#6**: The first surrogate model with above 90% but relatively low complexity. 5 out of 8 decision stumps have a high weighted probability

**#41**: The decision threshold is at approx. 0.55, with the left subtree doing better than the right subtree due to fewer mixed instances (left bar chart)

**#14**: A unique decision stump with a moderate weighted probability value (red colored and dashed lines). Depending on time, more unique and important can be explored at this stage!

**#41**: Behavioral surrogate summarization with many stumps

**#41**: 3 out of the 6 stumps predict the class to be positive, and the other three negative

**#41**: The default surrogate model with approx. 96% fidelity, with its behavior being summarized in the segmented bar chart. Most decision stumps are very weak (low weighted probability in dark blue), but help smoothen the decision boundaries (check this effect at the multiple decision thresholds of the segmented bar chart)

Figure 1

(1) Surrogate Model Selection

Figure 6

(2) Behavioral Model Summarization

Figure 1

(3) Test Set Results

**#7-#11**: These five surrogate models are more accurate (see fidelity score) when using fewer decimal digits (2 instead of 4)

**#6**: The first surrogate model with above 90% but relatively low complexity. 5 out of 8 decision stumps have a high weighted probability

**#41**: The decision threshold is at approx. 0.55, with the left subtree doing better than the right subtree due to fewer mixed instances (left bar chart)

**#41**: Insulin is the only feature that contributes to the negative class, then suddenly changes to positive (in purple), and finally continues to vote for negative. That is unusual and requires further investigation

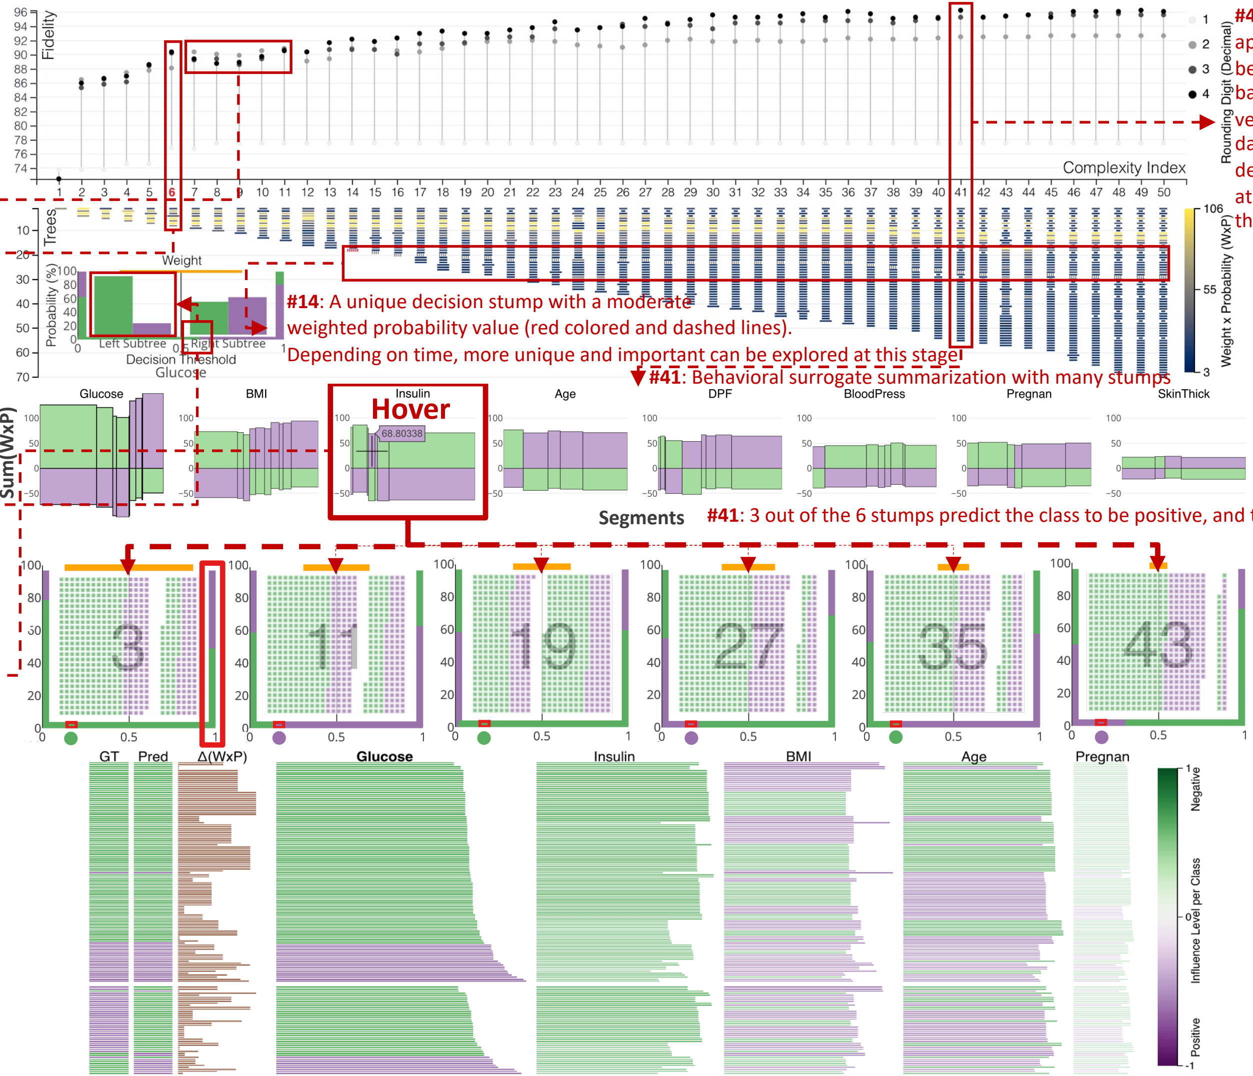


**#41**: The default surrogate model with approx. 96% fidelity, with its behavior being summarized in the segmented bar chart. Most decision stumps are very weak (low weighted probability in dark blue), but help smoothen the decision boundaries (check this effect at the multiple decision thresholds of the segmented bar chart)

(1) Figure 1

Surrogate Model Selection

(2) Figure 6

Behavioral Model Summarization

(3) Figure 1

Test Set Results

**#7-#11**: These five surrogate models are more accurate (see fidelity score) when using fewer decimal digits (2 instead of 4)

**#6**: The first surrogate model with above 90% but relatively low complexity. 5 out of 8 decision stumps have a high weighted probability

**#41**: The decision threshold is at approx. 0.55, with the left subtree doing better than the right subtree due to fewer mixed instances (left bar chart)

**#41**: Insulin is the only feature that contributes to the negative class, then suddenly changes to positive (in purple), and finally continues to vote for negative. That is unusual and requires further investigation

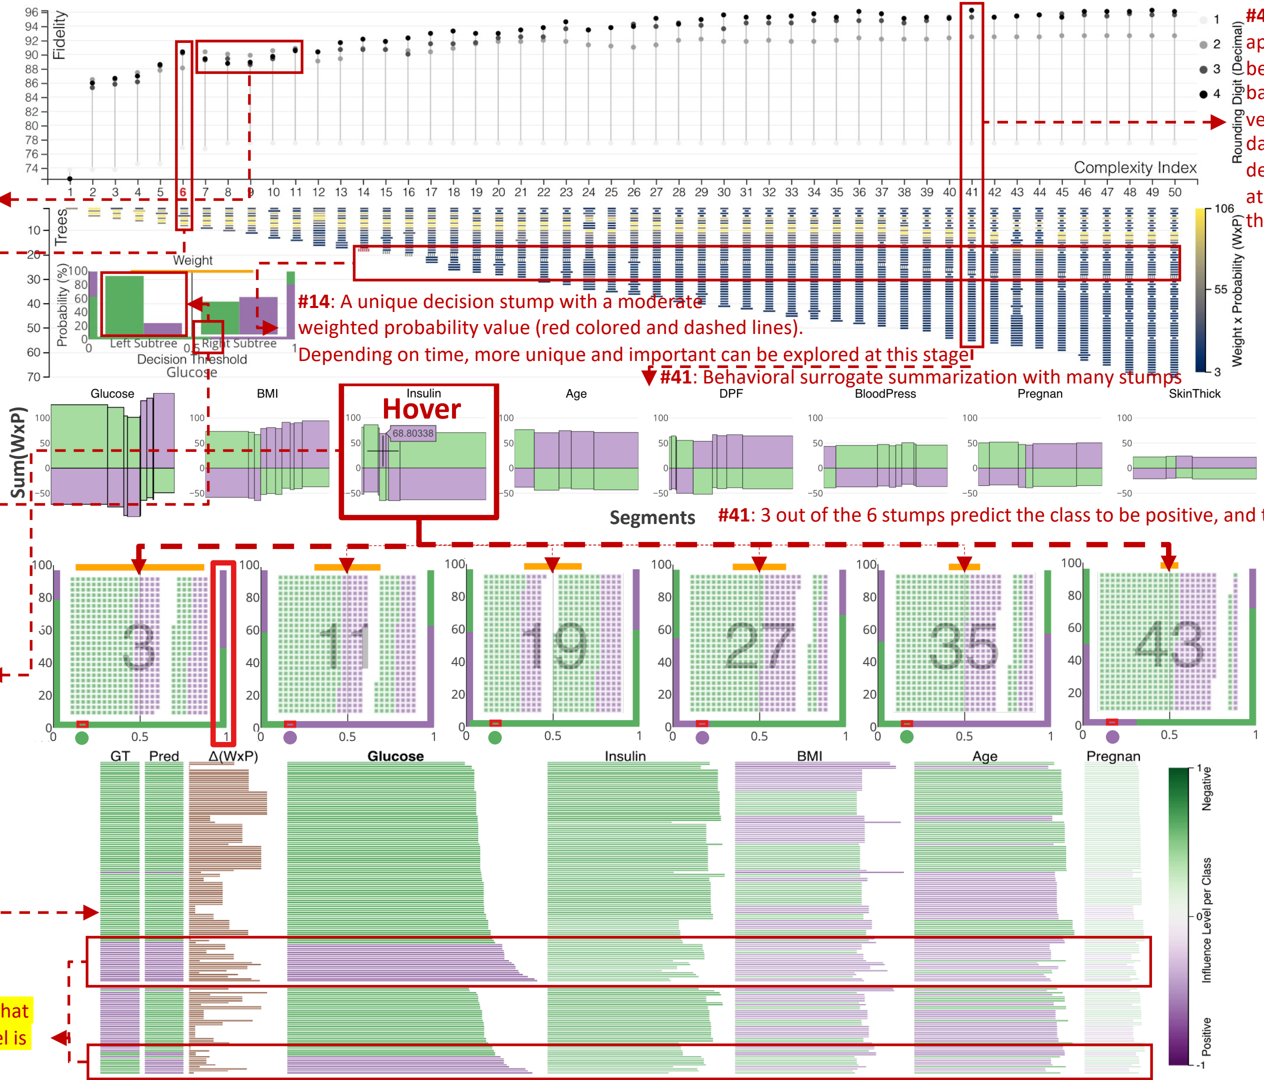


**#14**: A unique decision stump with a moderate weighted probability value (red colored and dashed lines). Depending on time, more unique and important can be explored at this stage

**#41**: Behavioral surrogate summarization with many stumps

**#41**: 3 out of the 6 stumps predict the class to be positive, and the other three negative

**#6**: Sorting based on Glucose shows that the prediction of this surrogate model is mostly done based on this feature

**#41**: The default surrogate model with approx. 96% fidelity, with its behavior being summarized in the segmented bar chart. Most decision stumps are very weak (low weighted probability in dark blue), but help smoothen the decision boundaries (check this effect at the multiple decision thresholds of the segmented bar chart)

(1) Figure 1

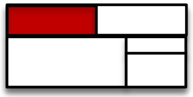

Surrogate Model Selection

(2) Figure 6

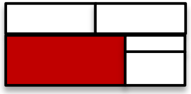

Behavioral Model Summarization

(3) Figure 1

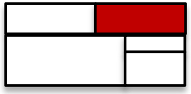

Test Set Results

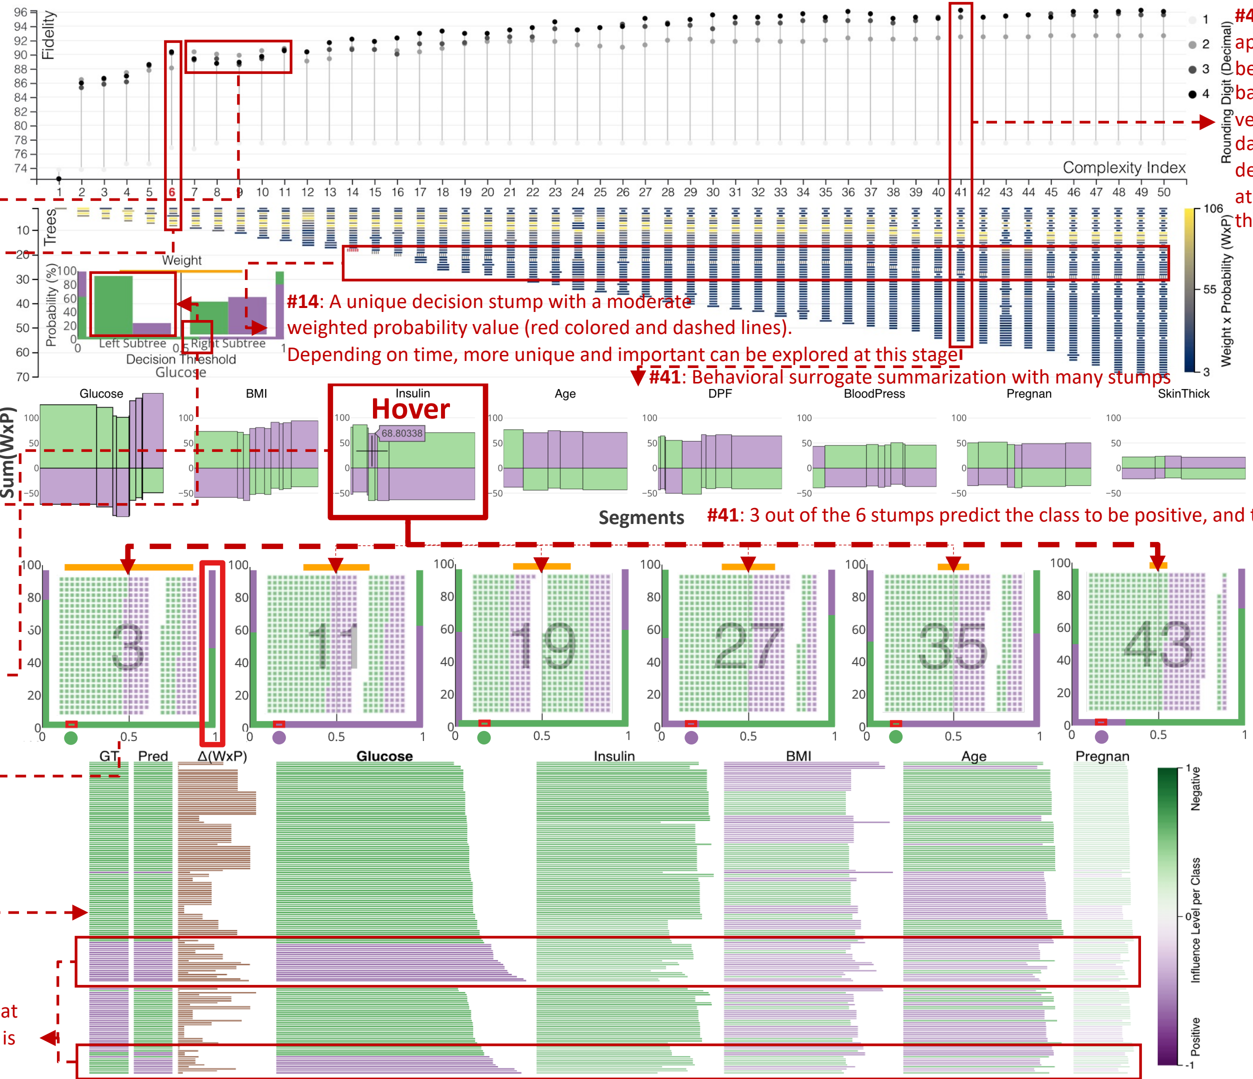


**#41**: The default surrogate model with approx. 96% fidelity, with its behavior being summarized in the segmented bar chart. Most decision stumps are very weak (low weighted probability in dark blue), but help smoothen the decision boundaries (check this effect at the multiple decision thresholds of the segmented bar chart)

**#7-#11**: These five surrogate models are more accurate (see fidelity score) when using fewer decimal digits (2 instead of 4)

**#6**: The first surrogate model with above 90% but relatively low complexity. 5 out of 8 decision stumps have a high weighted probability

**#14**: A unique decision stump with a moderate weighted probability value (red colored and dashed lines). Depending on time, more unique and important can be explored at this stage!

**#41**: Behavioral surrogate summarization with many stumps

**#41**: The decision threshold is at approx. 0.55, with the left subtree doing better than the right subtree due to fewer mixed instances (left bar chart)

**#41**: 3 out of the 6 stumps predict the class to be positive, and the other three negative

**#41**: Insulin is the only feature that contributes to the negative class, then suddenly changes to positive (in purple), and finally continues to vote for negative. That is unusual and requires further investigation

**#41**: This decision stump is the most influential in terms of weight but is divided at about 50% between the two classes. When summing up all decision stumps, this stump is like being ruled out

**#6**: Sorting based on Glucose shows that the prediction of this surrogate model is mostly done based on this feature

(1) Figure 1

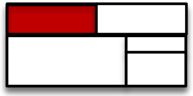

Surrogate Model Selection

(2) Figure 6

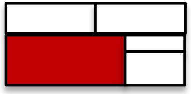

Behavioral Model Summarization

(3) Figure 1

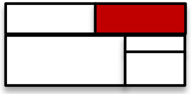

Test Set Results

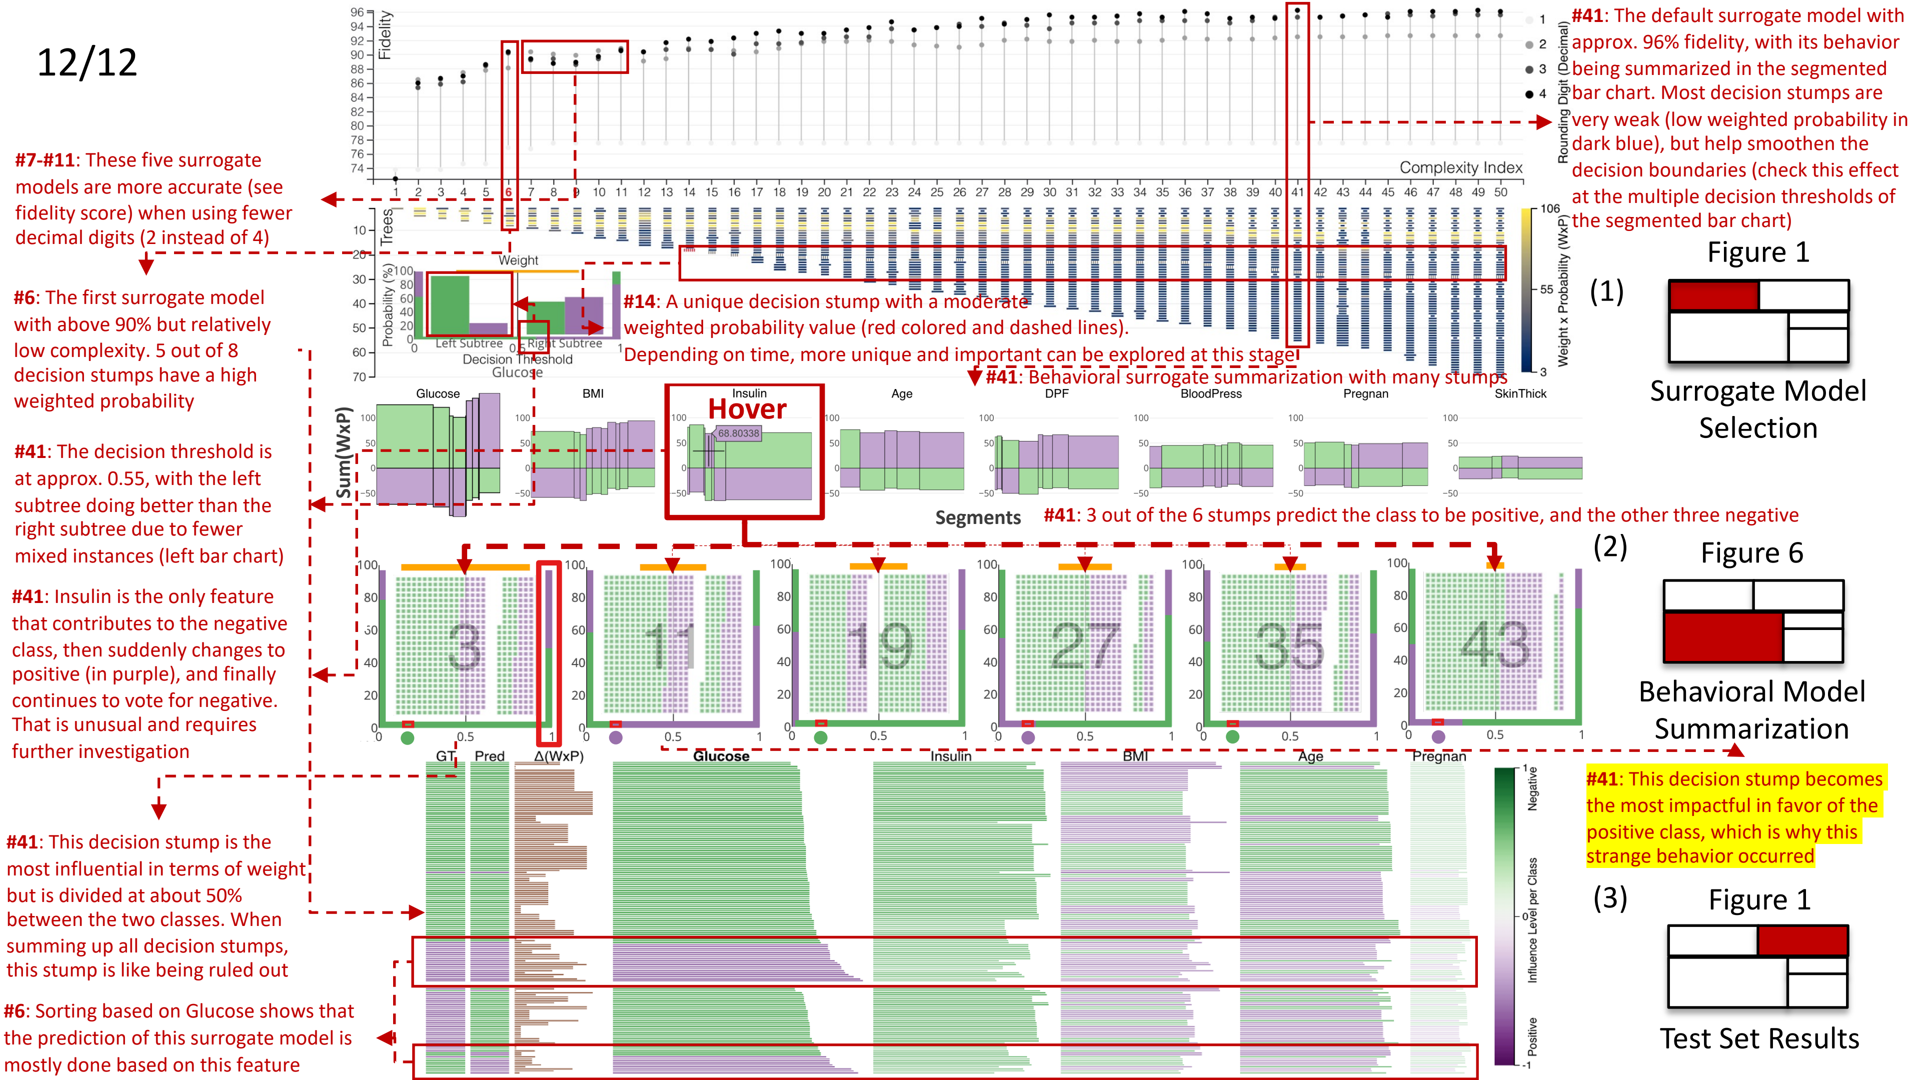
#7-#11: These five surrogate models are more accurate (see fidelity score) when using fewer decimal digits (2 instead of 4)
#6: The first surrogate model with above 90% but relatively low complexity. 5 out of 8 decision stumps have a high weighted probability
#41: The decision threshold is at approx. 0.55, with the left subtree doing better than the right subtree due to fewer mixed instances (left bar chart)
#41: Insulin is the only feature that contributes to the negative class, then suddenly changes to positive (in purple), and finally continues to vote for negative. That is unusual and requires further investigation
#41: This decision stump is the most influential in terms of weight but is divided at about 50% between the two classes. When summing up all decision stumps, this stump is like being ruled out
#6: Sorting based on Glucose shows that the prediction of this surrogate model is mostly done based on this feature
Fidelity
Complexity Index
Rounding Digit (Decimal)
Trees
Weight
Probability (%)
Left Subtree
Right Subtree
Decision Threshold
Glucose
Weight x Probability (WxP)
#14: A unique decision stump with a moderate weighted probability value (red colored and dashed lines). Depending on time, more unique and important can be explored at this stage
#41: Behavioral surrogate summarization with many stumps
Sum(WxP)
Glucose
BMI
Insulin
Hover
68.80338
Age
DPF
BloodPress
Pregnan
SkinThick
Segments
#41: 3 out of the 6 stumps predict the class to be positive, and the other three negative
3
11
19
27
35
43
GT
Pred
Δ(WxP)
Glucose
Insulin
BMI
Age
Pregnan
Influence Level per Class
Negative
Positive
#41: The default surrogate model with approx. 96% fidelity, with its behavior being summarized in the segmented bar chart. Most decision stumps are very weak (low weighted probability in dark blue), but help smoothen the decision boundaries (check this effect at the multiple decision thresholds of the segmented bar chart)
(1)
Figure 1
Surrogate Model Selection
(2)
Figure 6
Behavioral Model Summarization
#41: This decision stump becomes the most impactful in favor of the positive class, which is why this strange behavior occurred
(3)
Figure 1
Test Set Results

Figure 1

Behavioral Model Summarization

(1)

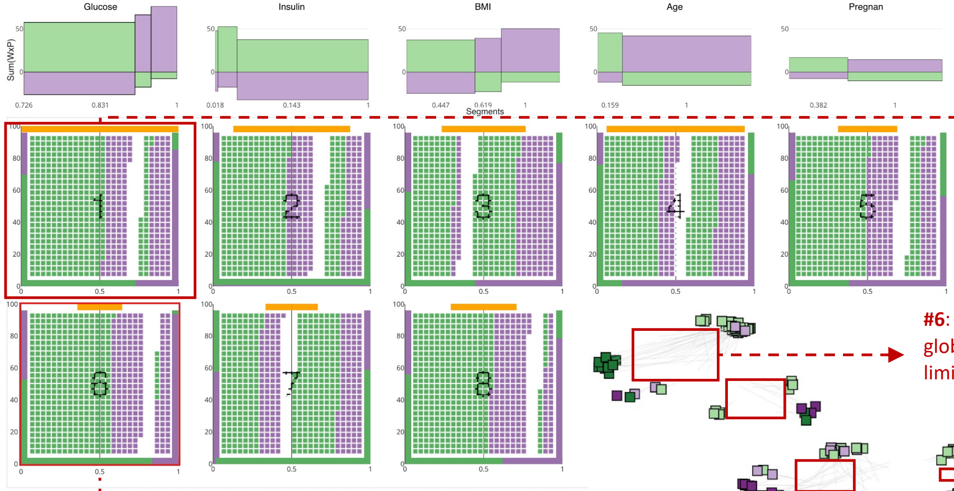


#6: If one decision stump had to be chosen, this is clearly the one that summarizes the behavior of the black box, more complex, model

#6: Inspired by the decision stump in #14, this secondary decision stump could be adjusted by lowering the threshold to approx. 0.55

(3)

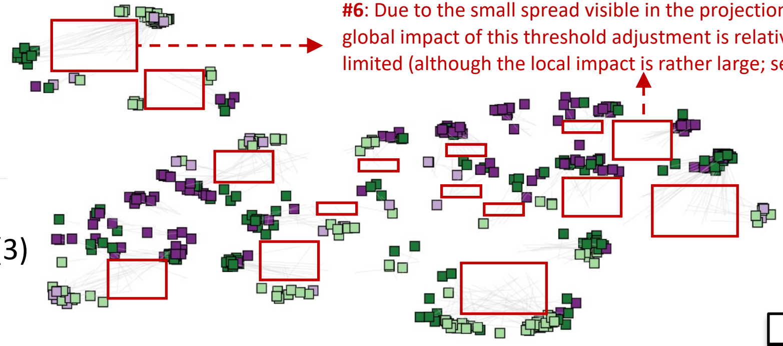

#6: Due to the small spread visible in the projection, the global impact of this threshold adjustment is relatively limited (although the local impact is rather large; see colors)

Figure 1

Decisions Comparison

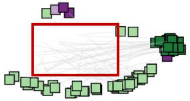

#6: Since many negative to diabetes training instances will fall into the wrong subtree, the domain experts should investigate and evaluate this model behavior further

Figure 1

Rule Overriding

#6: The currently selected decision stump has the lowest impurity and a rather low weighted probability

(2)

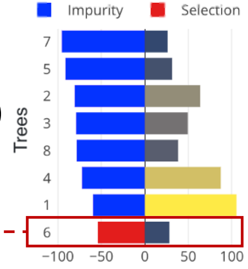


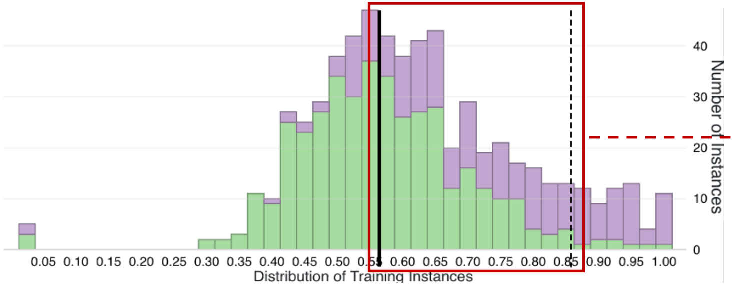

Figure 1

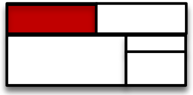

Behavioral Model Summarization

(1)

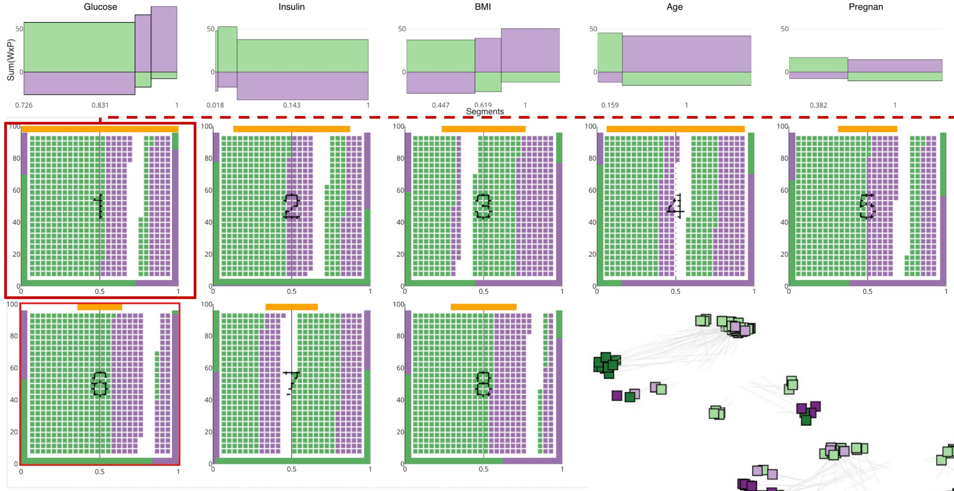


**#6**: If one decision stump had to be chosen, this is clearly the one that summarizes the behavior of the black box, more complex, model

(3)

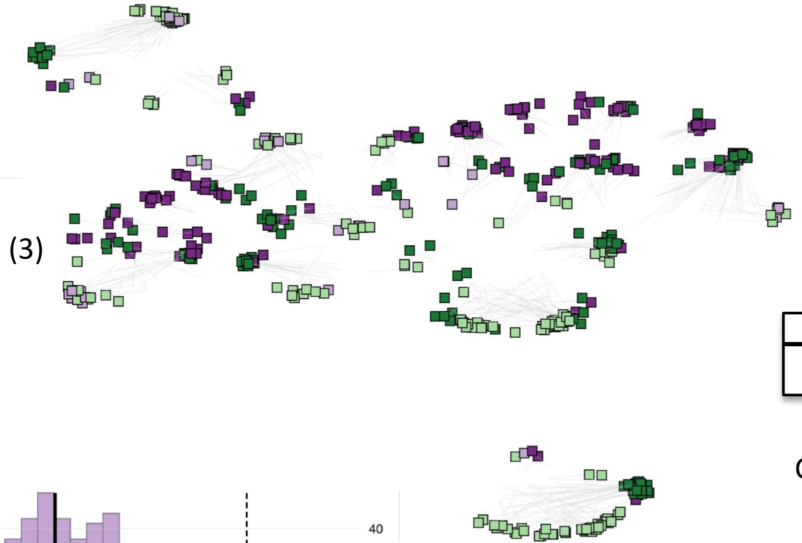

Figure 1

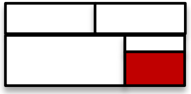

Decisions Comparison

Figure 1

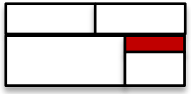

Rule Overriding

(2)

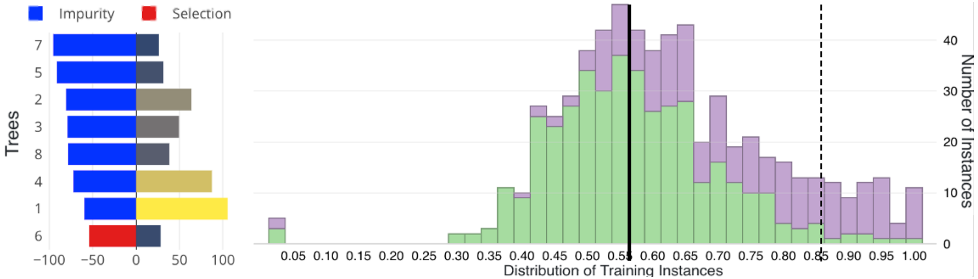

3/6

Figure 1

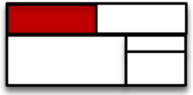

Behavioral Model Summarization

(1)

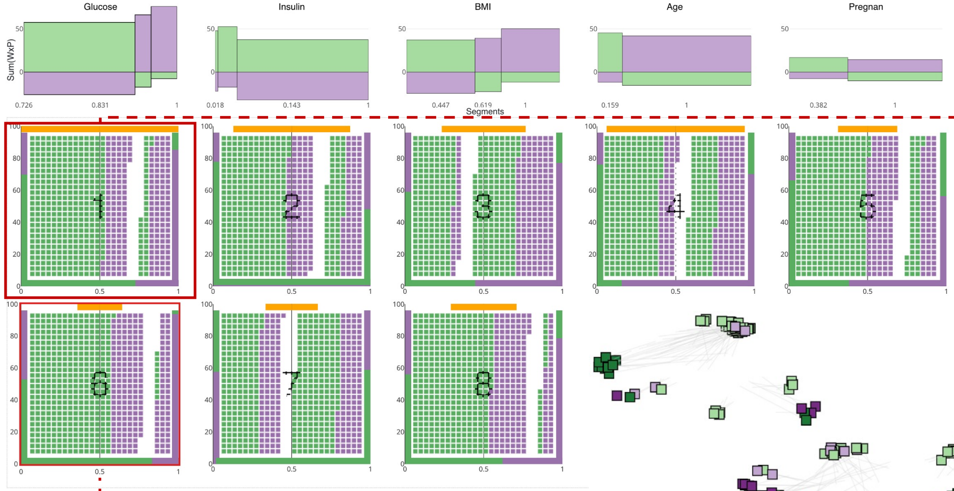


#6: If one decision stump had to be chosen, this is clearly the one that summarizes the behavior of the black box, more complex, model

#6: Inspired by the decision stump in #14, this secondary decision stump could be adjusted by lowering the threshold to approx. 0.55

(3)

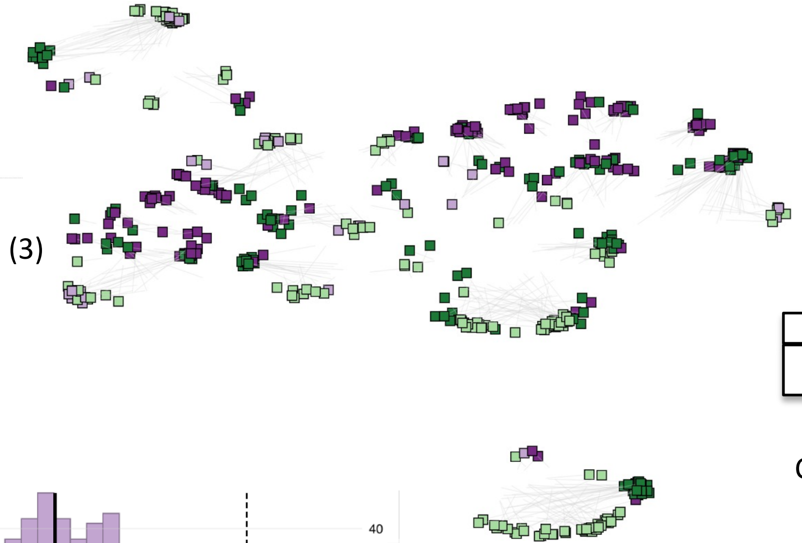

Figure 1

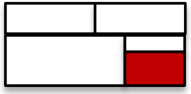

Decisions Comparison

Figure 1

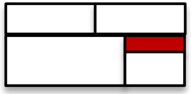

Rule Overriding

(2)

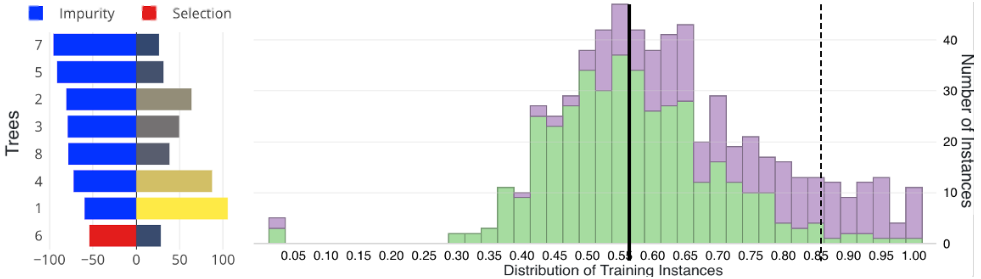

Figure 1

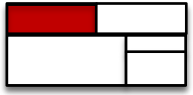

Behavioral Model Summarization

(1)

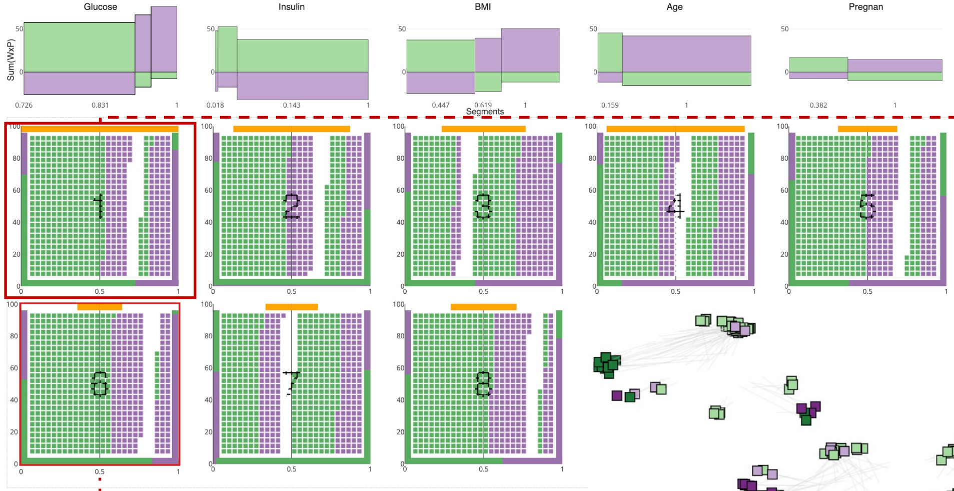


**#6**: If one decision stump had to be chosen, this is clearly the one that summarizes the behavior of the black box, more complex, model

**#6**: Inspired by the decision stump in #14, this secondary decision stump could be adjusted by lowering the threshold to approx. 0.55

(3)

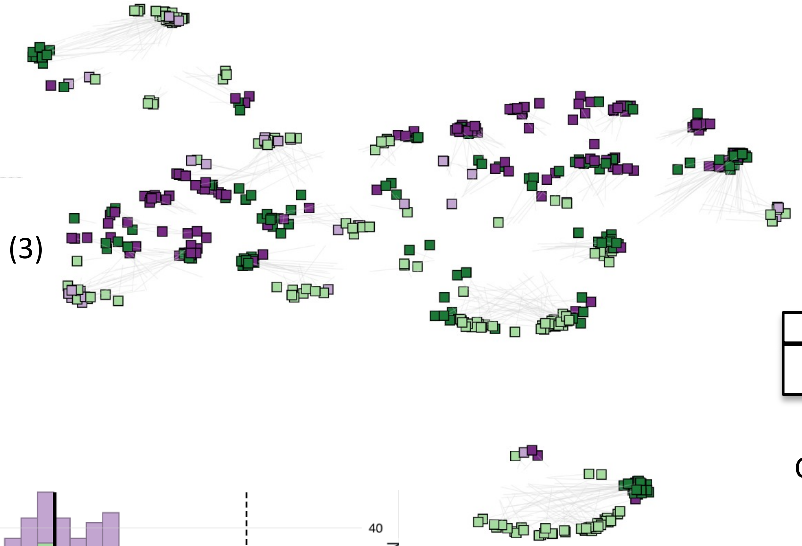

Figure 1

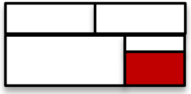

Decisions Comparison

**#6**: The currently selected decision stump has the lowest impurity and a rather low weighted probability

Figure 1

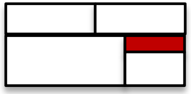

Rule Overriding

(2)

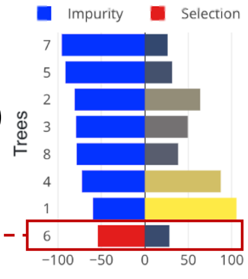


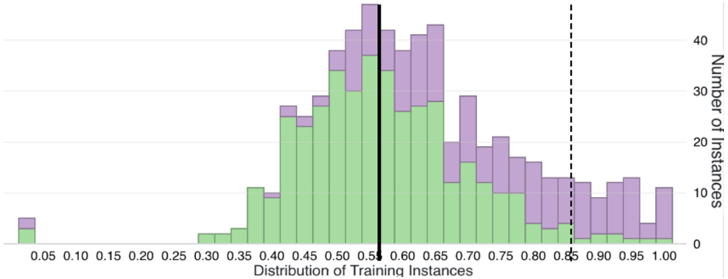

Figure 1

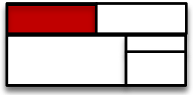

Behavioral Model Summarization

(1)

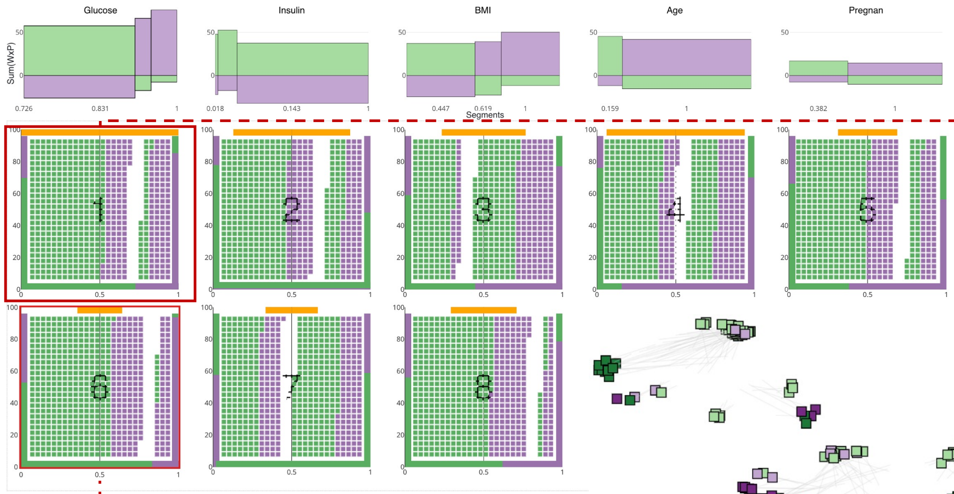


**#6**: If one decision stump had to be chosen, this is clearly the one that summarizes the behavior of the black box, more complex, model

**#6**: Inspired by the decision stump in #14, this secondary decision stump could be adjusted by lowering the threshold to approx. 0.55

(3)

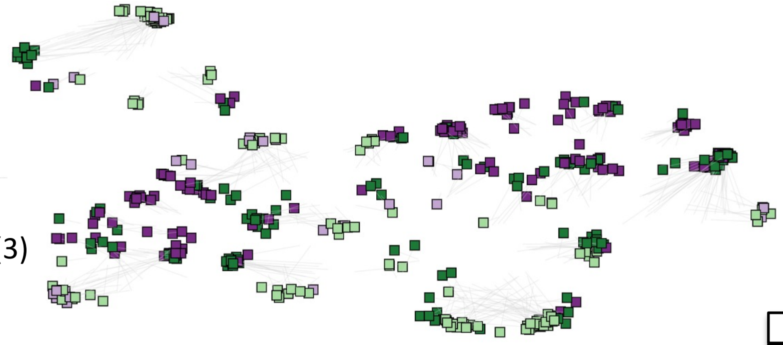

Figure 1

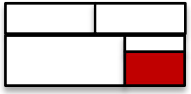

Decisions Comparison

**#6**: Since many negative to diabetes training instances will fall into the wrong subtree, the domain experts should investigate and evaluate this model behavior further

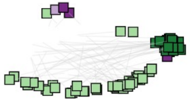

**#6**: The currently selected decision stump has the lowest impurity and a rather low weighted probability

Figure 1

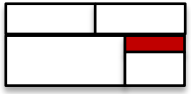

Rule Overriding

(2)

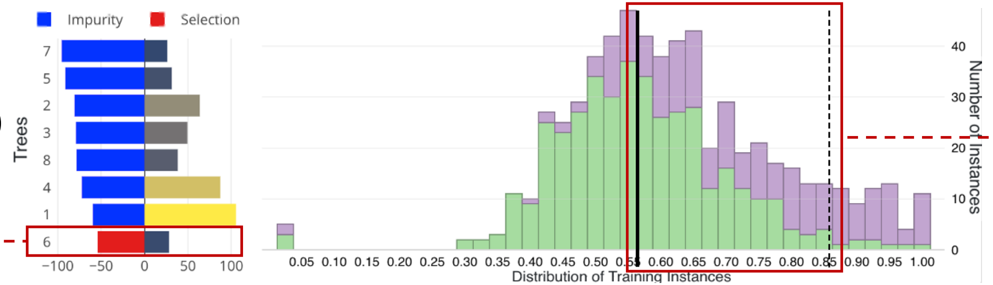

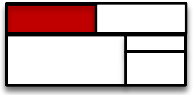


(1)

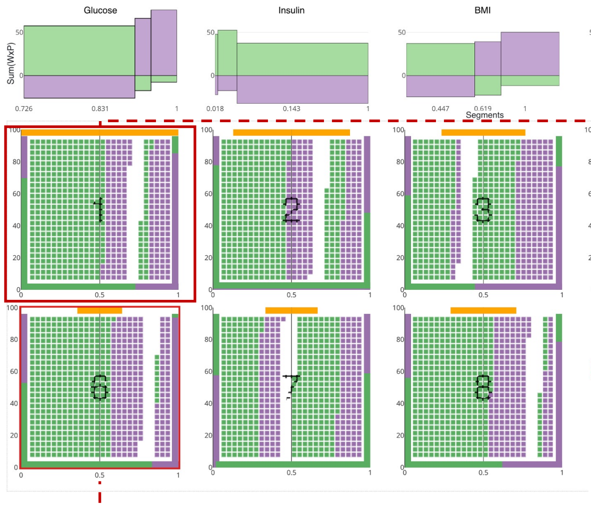


#6: If one decision stump had to be chosen, this is clearly the one that summarizes the behavior of the black box, more complex, model

#6: Due to the small spread visible in the projection, the global impact of this threshold adjustment is relatively limited (although the local impact is rather large; see colors)

#6: Inspired by the decision stump in #14, this secondary decision stump could be adjusted by lowering the threshold to approx. 0.55

(3)

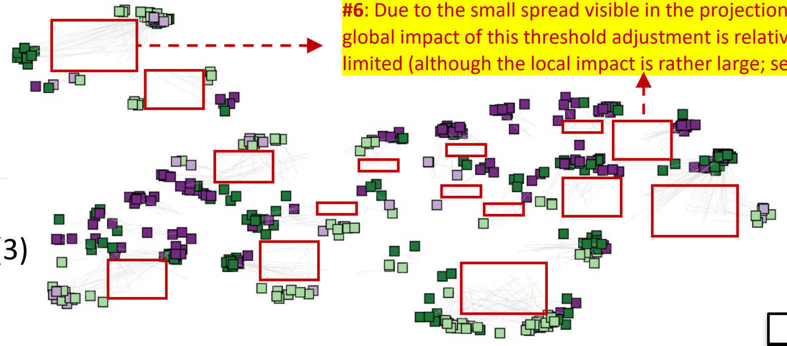

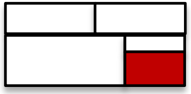


#6: Since many negative to diabetes training instances will fall into the wrong subtree, the domain experts should investigate and evaluate this model behavior further

#6: The currently selected decision stump has the lowest impurity and a rather low weighted probability

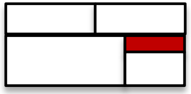


(2)

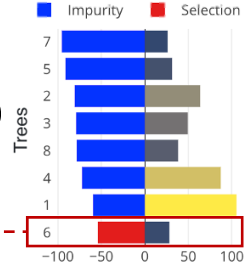


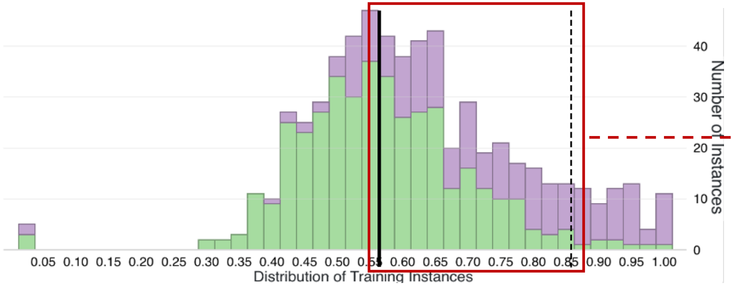


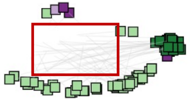

Supplement: Supplementary file 1 [file supplemental_step-by-step.pdf]
