# Supplementary material for: DeforestVis: Behavior Analysis of Machine Learning Models with Surrogate Decision Stumps
Source: arXiv:2304.00133 source file (2024-04-18)

# DeforestVis: Behavior Analysis of Machine Learning Models with Surrogate Decision Stump

## Section 6.1: Use case

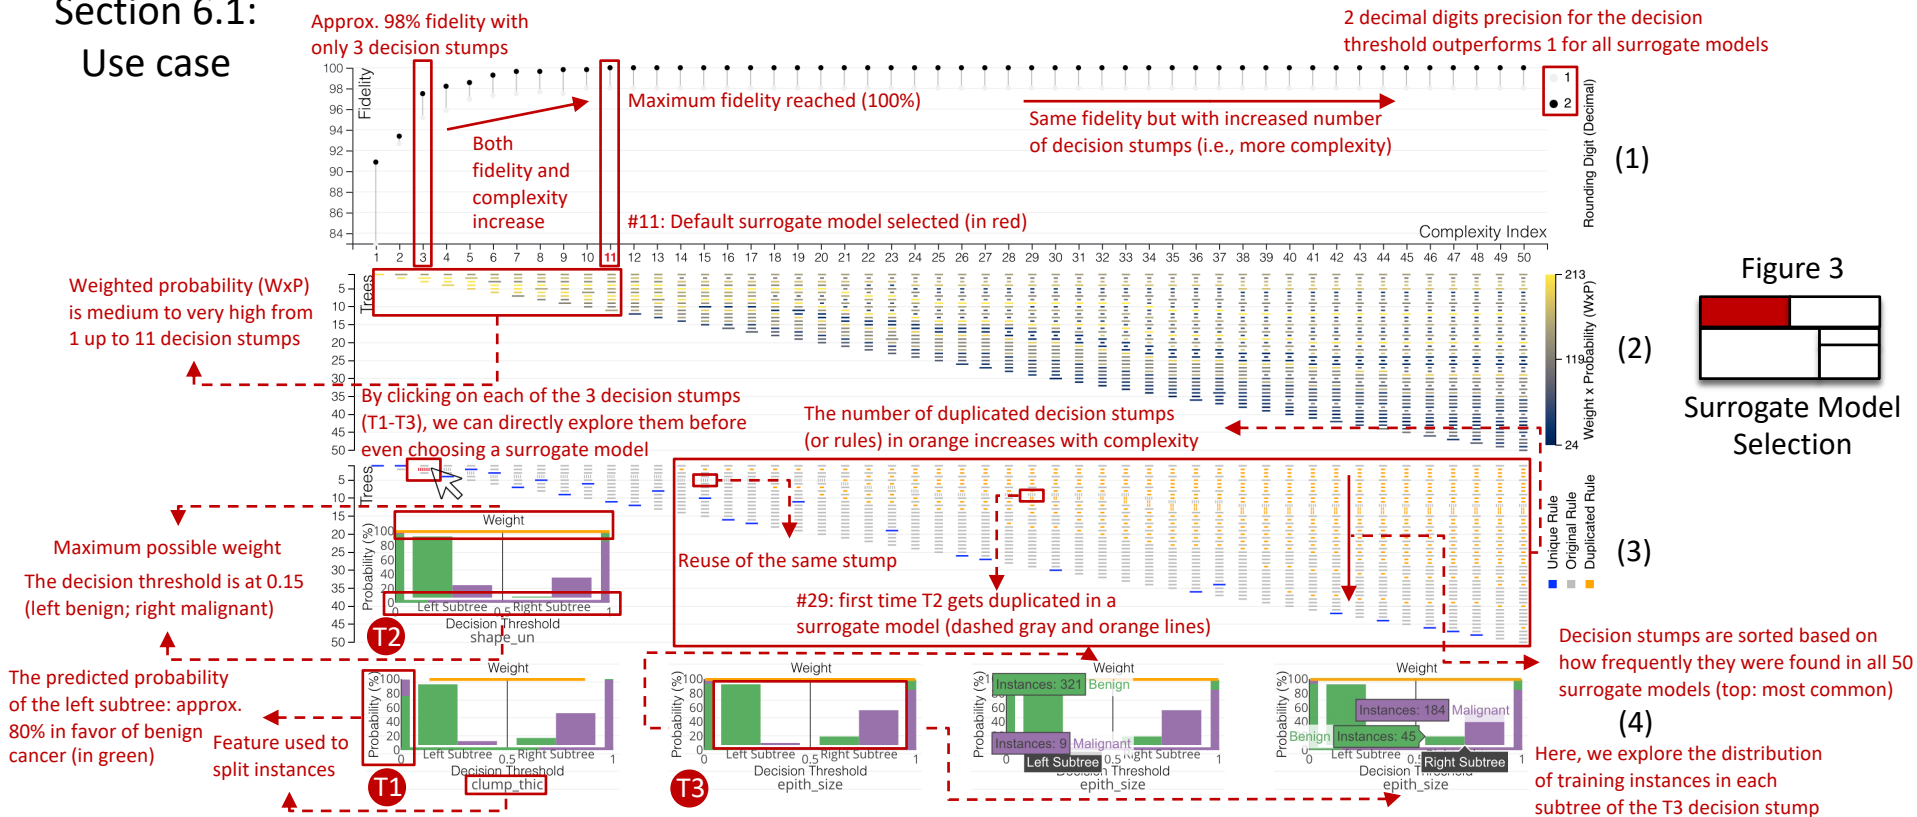

Figure 4

## Overriding

T2 is the least informative  
decision stump  
(smallest bar)

T2 is the most impactful decision stump out of the 3 because of the highest weighted probability ( $W \times P$ ; vibrant yellow)

Initially, the T2 threshold is at 0.15 (dashed line), but many benign samples (in green) are classified as malignant (right subtree) according to the ground truth

After inspecting what will happen if the threshold becomes 0.25, we confirm this change

The hovered benign instance from the right subtree moved to the left subtree, which is correct. It is now an easy-to-classify instance far away from the border since the grid of instances is sorted based on how easy it is to be classified in the opposite class

Figure 4

## Behavioral Model Summarization

(1)

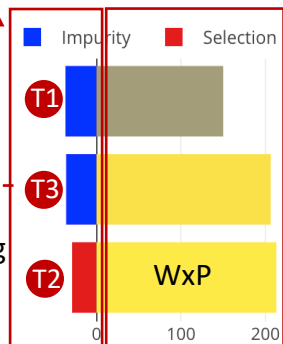

(2)

The position in the projection is based on the 3 decision stumps (6 dimensions in total; left and right subtrees times 3 stumps) being reduced to 2 dimensions

Each group means instances belong to similar subtrees for all decision stumps. The first pair of white and red small boxes shows T2 (shape\_un), then T3 (epith\_size), and finally T1 (clump\_thic)

The colors are for the selected stump T2 (local examination)

|                          |                           |
|--------------------------|---------------------------|
| Left Subtree (Benign)    | Right Subtree (Benign)    |
| Left Subtree (Malignant) | Right Subtree (Malignant) |

## Problematic Cases

## A Misclassified Benign Instance

These benign instances were in the right subtree (dark green). After changing the decision threshold to 0.25, they moved to the left subtree (light green). Their new position is closer to the other benign samples, which is ideal (global examination)

## Fixed Most Cases

The problematic benign samples moved from the right subtree to the left subtree after adapting the decision threshold (see trajectories as gray lines)

(3)

Figure 4

## Decisions Comparison

(4)

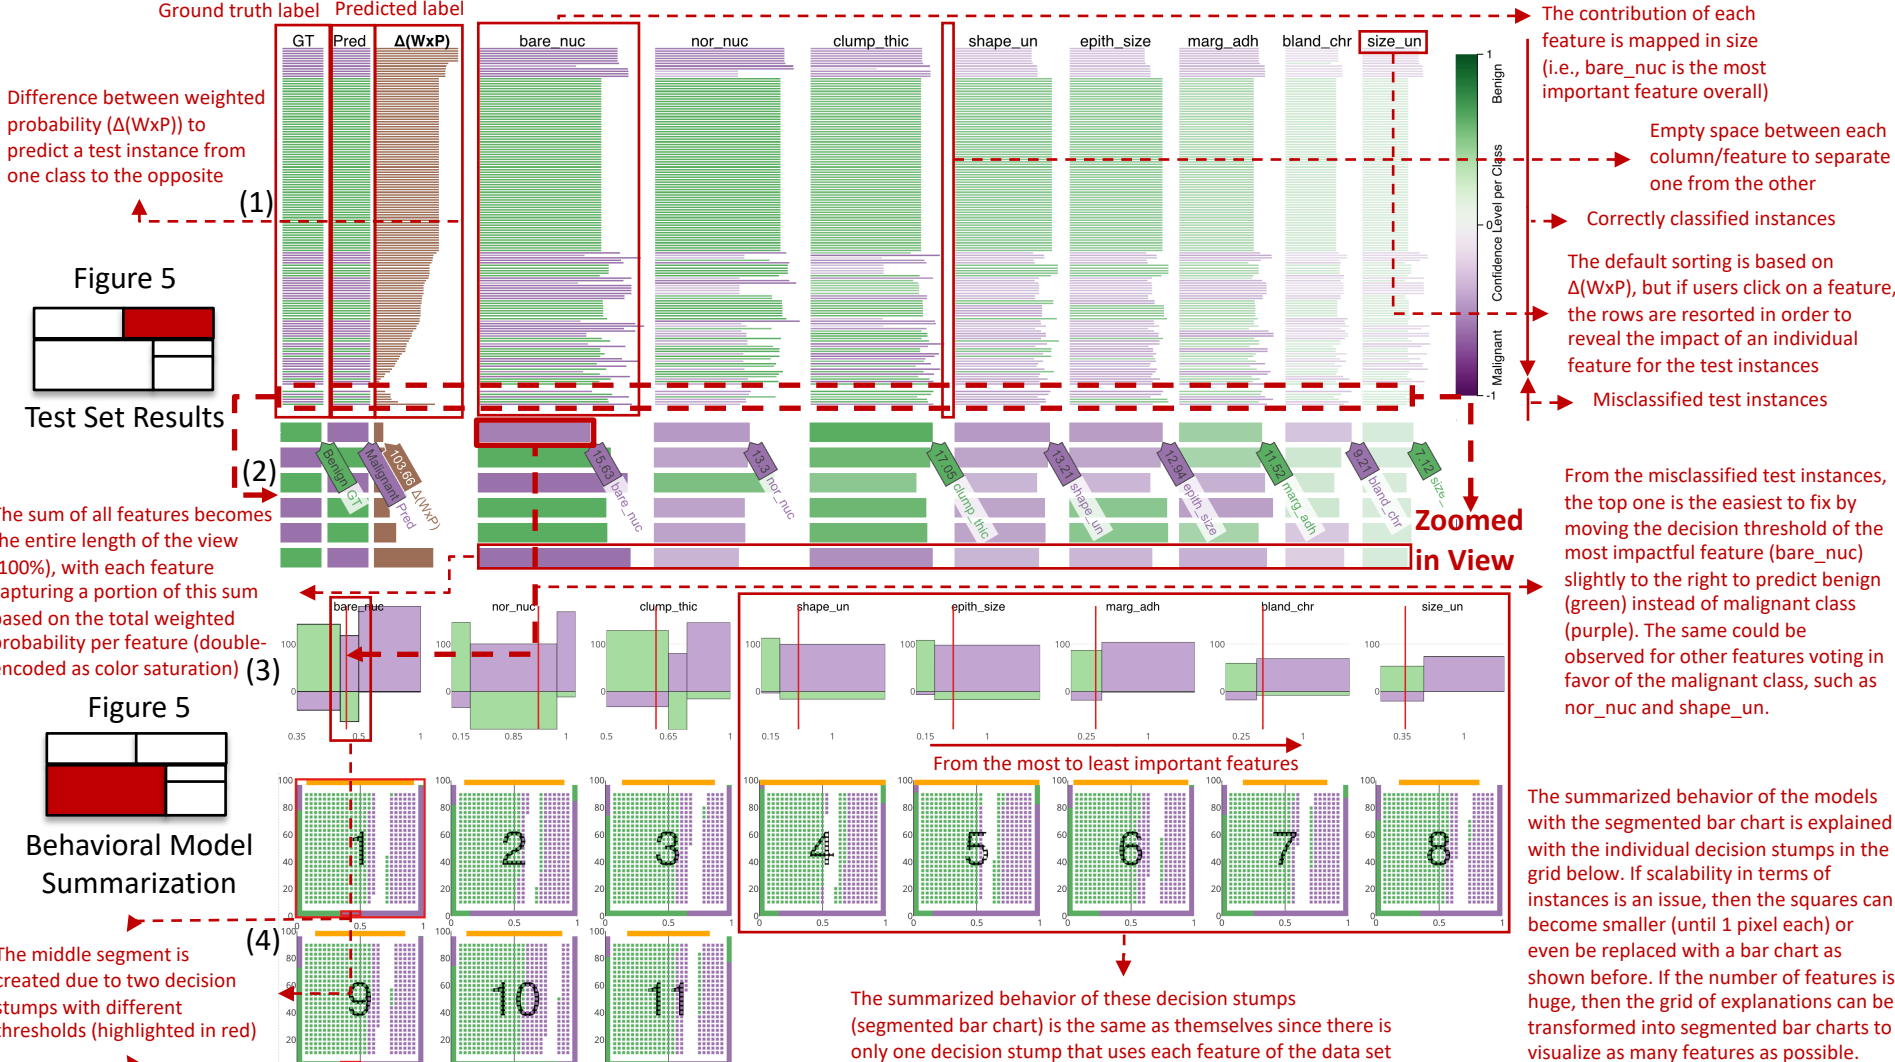

## Section 6.2: Usage scenario

**#7-#11:** These five surrogate models are more accurate (see fidelity score) when using fewer decimal digits (2 instead of 4)

**#6:** The first surrogate model with above 90% but relatively low complexity. 5 out of 8 decision stumps have a high weighted probability

**#41:** The decision threshold is at approx. 0.55, with the left subtree doing better than the right subtree due to fewer mixed instances (left bar chart)

**#41:** Insulin is the only feature that contributes to the negative class, then suddenly changes to positive (in purple), and finally continues to vote for negative. That is unusual and requires further investigation

**#41:** This decision stump is the most influential in terms of weight but is divided at about 50% between the two classes. When summing up all decision stumps, this stump is like being ruled out

**#6:** Sorting based on Glucose shows that the prediction of this surrogate model is mostly done based on this feature

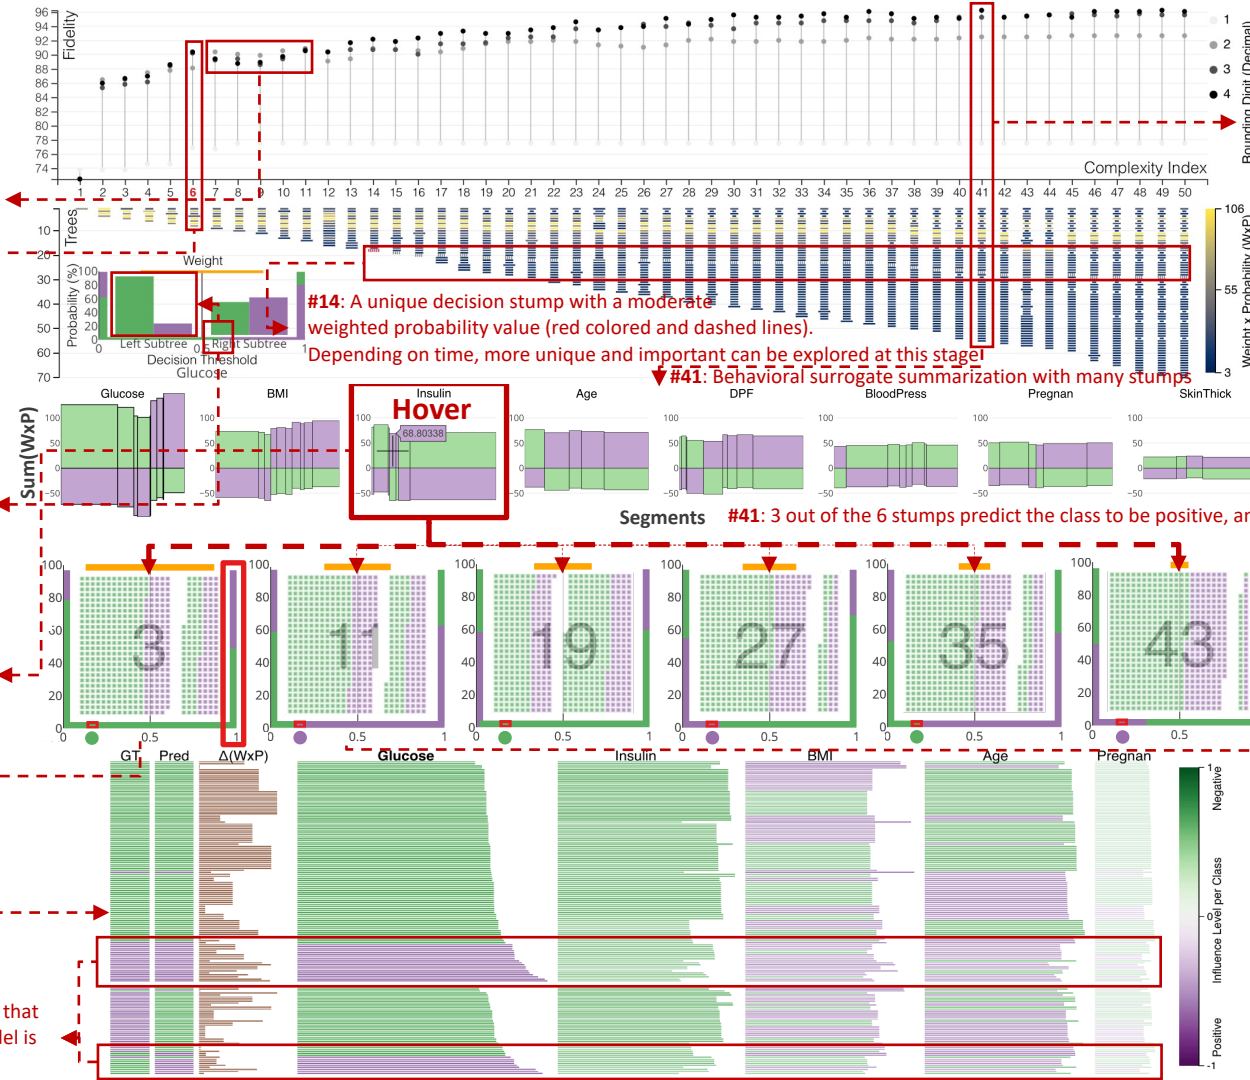

**#41:** The default surrogate model with approx. 96% fidelity, with its behavior being summarized in the segmented bar chart. Most decision stumps are very weak (low weighted probability in dark blue), but help smoothen the decision boundaries (check this effect at the multiple decision thresholds of the segmented bar chart)

Figure 1

(1)

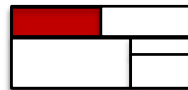

Surrogate Model  
Selection

(2)

Figure 6

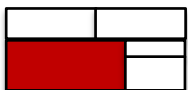

Behavioral Model  
Summarization

(3)

Figure 1

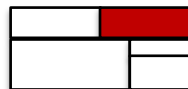

Test Set Results

**#41:** This decision stump becomes the most impactful in favor of the positive class, which is why this strange behavior occurred

Figure 1

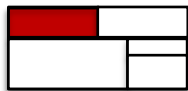

Behavioral Model  
Summarization

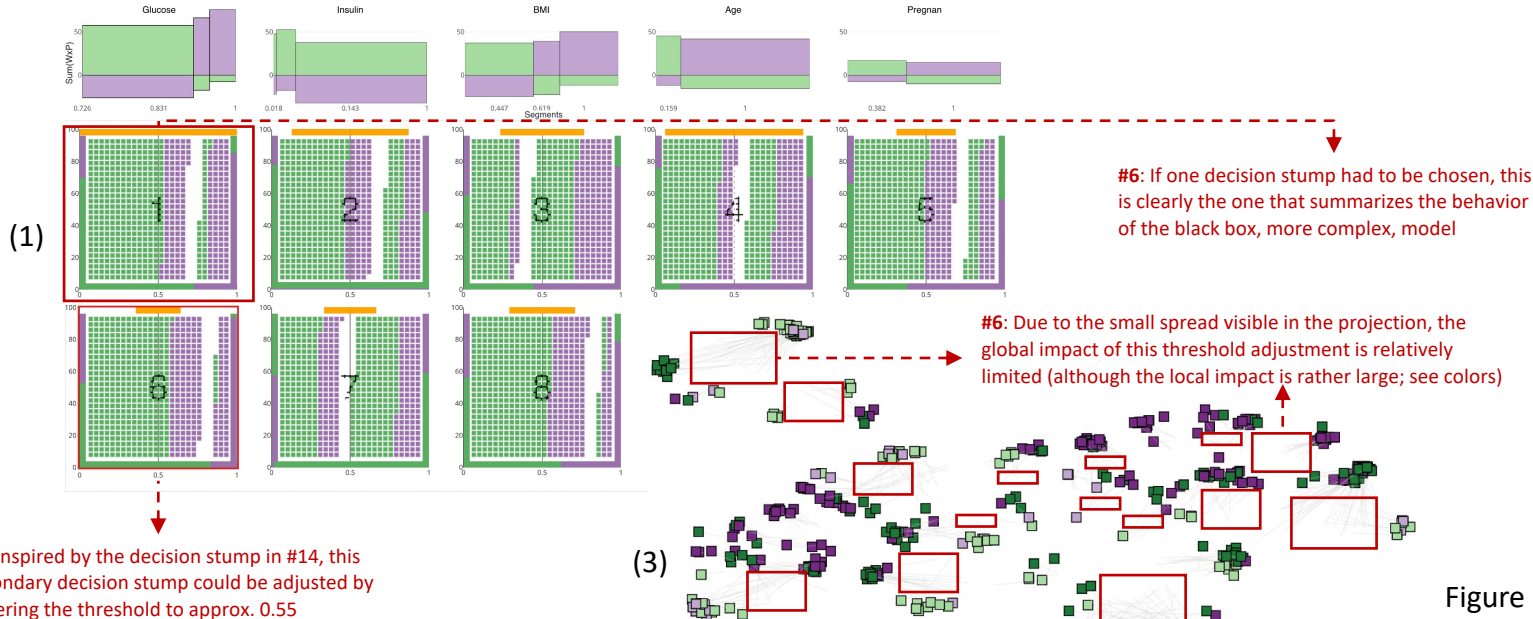

Figure 1

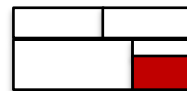

Decisions  
Comparison

Figure 1

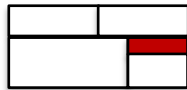

Rule Overriding

#6: The currently selected decision stump has the lowest impurity and a rather low weighted probability

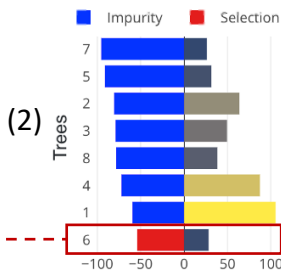

#6: Since many negative to diabetes training instances will fall into the wrong subtree, the domain experts should investigate and evaluate this model behavior further

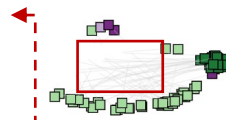

Supplement: Supplementary file 2 [file supplemental.pdf]
